# Supplementary material for: Inertial-Range Reconnection in Magnetohydrodynamic Turbulence and in the Solar Wind
Source: arXiv:1503.00509 ancillary file (2015-03-02)
Supplement: Supplementary file 1 [file Fig2_3-3D-documentation.pdf]

## Documentation for Fig2-3D.pdf and Fig3-3D.pdf

The 3DPDF versions of Figs.2 and 3 are, except for being 3D, identical to the figures that appear in the Letter. Here we just list some additional quantitative details that could not be provided in the limited space of the Letter.

In Figure 3 the “X-point” was located by eye by plotting trial field-lines of the coarse-grained magnetic field and the location determined to be approximately [2.83, 1.31, 5.72], marked with the solid black dot • in the figure. The magnetic flux-rope in figure 3 visualized by the yellow surface is the half-maximum (0.301) isosurface of the magnitude of the coarse-grained magnetic field. The red and green straight lines through the “X-point” are, respectively, in the L- and N-directions of a minimum-variance frame (MVF) of the fine-grained magnetic field. We calculate the MVF from data in a sphere around the “X-point” with radius equal to one magnetic integral length (0.35). This MVF eigenbasis was found to be given by the following unit vectors:

L-direction: [ 0.7480 -0.6189 0.2398];  
M-direction: [-0.2729 -0.6161 -0.7389];  
N-direction: [-0.6050 -0.4872 0.6298].

In the main text of the Letter this was compared with the MVF calculated using the fine-grained magnetic field on the original 1D datacut, with center at point [2.96, 0.91, 5.84] and extending length 0.7 along the simulation y-axis. The MVF for this “simulated spacecraft” data had the eigenbasis:

L-direction: [ 0.6014 -0.5716 0.5582];  
M-direction: [-0.7950 -0.4977 0.3469];  
N-direction: [-0.0795 0.6523 0.7537].

In Figure 3 are also plotted field lines of the coarse-grained magnetic field through points placed regularly along the L- and N-axes at the “X-point”. 15 upstream and 15 downstream points were placed along the L-axis, with a separation of 0.06. Along the N-axis, 20 upstream and 15 downstream points were placed at a separation of 0.03. A twice smaller separation was used along the N-direction, because the width of the reconnection region along the N-direction is about twice smaller than its length in the L-direction. The field-lines of the coarse-grained field passing through the points placed along the L-axis appear in red, and the lines through the points along the N-axis appear in green, corresponding to “outgoing” and “incoming” lines, respectively. Along these field-lines we also plot as blue arrows → the coarse-grained velocity-field vectors at regular distances. We subtracted the local mean velocity of the plasma, which we determined by averaging over points in a ball around the “X-point” of radius 0.4, giving a local mean velocity of [0.1902, -0.0184, 0.0550].

Figure 2 is very similar to Figure 3, except that the field-lines are those of the fine-grained magnetic field and the yellow surface represents the half-maximum

## Documentation for Fig2-3D.pdf and Fig3-3D.pdf

(1.107) isosurface of the magnitude of the fine-grained magnetic field. Note, however, that the solid black dot • is the same as for Figure 3 and represents an “X-point” of the coarse-grained magnetic field. Likewise, the **red** and **green** straight lines through the “X-point” represent the L- and N-axes for the same MVF as in Figure 2. Due to the complex wandering of the lines of the fine-grained magnetic field, no velocity vectors are plotted on field-lines in Figure 2.

These and all other 3D figures included as Supplemental Material can be viewed with Acrobat Reader, version 7.0 and later. For full documentation, see

<https://helpx.adobe.com/acrobat/using/displaying-3d-models-pdfs.html>

For readers who may wish to manipulate the images in Acrobat Reader, we provide here a list of all objects as they appear under Toggle Model Tree.

|                          | Object in fig2_3D.pdf | Object in fig3_3D.pdf |
|--------------------------|-----------------------|-----------------------|
| x-axis                   | Plot_74               | Plot_1                |
| y-axis                   | Plot_75               | Plot_2                |
| z-axis                   | Plot_76               | Plot_3                |
| L-axis                   | Plot_108              | Plot_35               |
| N-axis                   | Plot_145              | Plot_72               |
| U-field on L-lines       | NA                    | Traj_1                |
| U-field on N-lines       | NA                    | Traj_2                |
| Center of 1D datacut     | Drop_3                | Drop_1                |
| X-point                  | Drop_4                | Drop_2                |
| 1D datacut               | Plot_146              | Plot_73               |
| B-isosurface             | Triplot_2             | Triplot_1             |
| Field-lines along L-axis | Plot_77 to Plot_107   | Plot_4 to Plot_34     |
| Field-lines along N-axis | Plot_109 to Plot_144  | Plot_36 to Plot_71    |
