# Supplementary material for: Inertial-Range Reconnection in Magnetohydrodynamic Turbulence and in the Solar Wind
Source: arXiv:1503.00509 ancillary file (2015-03-02)
Supplement: Supplementary file 2 [file Fig4_QSL-3D-documentation.pdf]

The 3DPDF version of Fig.4 is not identical to the figure that appears in the Letter, but instead shows the entire calculated QSL. To see cross-sections of the QSL, as in the Letter, select “Show Cross Section” from the 3D toolbar in Acrobat Reader. The default cross-section is perpendicular to the z-axis and through the center, but offsets and tilts of the cutting plane can be specified by selecting “Cross Section Properties” from the 3D toolbar.

To give additional perspective, we provided two additional 3DPDF’s, which plot the QSL together with other objects. The first of these two additional 3DPDF’s, “QSL\_and\_lines\_3D.pdf”, plots the QSL in **cyan** together with the lines of the coarse-grained magnetic field from Fig.3, with incoming lines in **blue** and outgoing in **red**. One can easily check that the “V’s” of the out-going field lines frame the “X” of the QSL. The second 3DPDF, “QSL\_and\_current\_3D.pdf” plots the QSL in **cyan** together with the intense (half-maximum) current sheets from Fig. 5a in **green**. One can check there is some tendency for these strong current sheets to form in the vicinity of the QSL (particularly at the lower right arm of the QSL as viewed in Fig.4), but the current sheets are not coincident with the QSL and some sheets in the reconnection region are quite distant from the QSL.

We give here some brief details about the calculation of the QSL, which follows standard approaches. After locating an “X-point” by eye at (2.8, 1.35, 5.65) we surrounded it with a sphere of radius 1.6 L. The QSL that we calculate was for the sphere-to-sphere mapping defined by the field-lines, from “launch points” on the sphere where lines enter at spherical coordinates  $(\theta, \phi)$  to “target points” where they exit at spherical coordinates  $(\Theta, \Phi)$ . Detailed formulas are provided by Titov (2007), who defined the perpendicular squashing factor by the ratio

$$Q_{\perp} = N_{\perp}^2 / |\Delta_{\perp}|$$

with

$$|\Delta_{\perp}| = |\mathbf{B}| / |\mathbf{B}^*|,$$

where the asterisk \* denotes the outgoing field-line, and with

$$N_{\perp}^2 = \text{tr}(D^T G_{\perp}^* D G^{\perp}),$$

$$D = \begin{pmatrix} \frac{\partial \Phi}{\partial \phi} & \frac{\partial \Phi}{\partial \theta} \\ \frac{\partial \Theta}{\partial \phi} & \frac{\partial \Theta}{\partial \theta} \end{pmatrix}$$

for

$$\begin{aligned}
 G_{\perp}^* &\equiv [g_{\perp ij}]^* \\
 &= R_*^2 \begin{pmatrix} \sin^2 \Theta \left( 1 - \frac{B_{\phi}^{*2}}{B^{*2}} \right) & -\sin \Theta \frac{B_{\phi}^* B_{\theta}^*}{B^{*2}} \\ -\sin \Theta \frac{B_{\phi}^* B_{\theta}^*}{B^{*2}} & 1 - \frac{B_{\theta}^{*2}}{B^{*2}} \end{pmatrix}, \\
 G^{\perp} &\equiv [g^{\perp ik}] = R_{\odot}^{-2} \begin{pmatrix} \sin^{-2} \theta \left( 1 + \frac{B_{\phi}^2}{B_r^2} \right) & \frac{B_{\phi} B_{\theta}}{\sin \theta B_r^2} \\ \frac{B_{\phi} B_{\theta}}{\sin \theta B_r^2} & 1 + \frac{B_{\theta}^2}{B_r^2} \end{pmatrix}
 \end{aligned}$$

We first tried to calculate the derivatives in the Jacobian matrix  $D$  by using finite-difference approximations, but this proved to be insufficiently accurate. Instead we followed an alternative numerical approach which gives accurate derivatives to machine precision. Let  $X(s, x_0)$  be the position along a field-line in arclength  $s$  for starting position  $x_0$ , determined by the ODE

$$(d/ds)X = \mathbf{b}(X), \quad X(0, x_0) = x_0 \quad (*)$$

where  $\mathbf{b} = \mathbf{B}/|\mathbf{B}|$  is the unit versor field for the magnetic field. Then it is easy to see that the Jacobian  $\mathbf{J} = \partial X(s, x_0) / \partial x_0$  is given by solving the matrix ODE

$$(d/ds)\mathbf{J} = (\partial \mathbf{b} / \partial \mathbf{x})(X(s)) \mathbf{J} \quad (**)$$

in arclength  $s$  along that line, with initial condition  $\mathbf{J} = \mathbf{I}$  for  $s=0$ . These equations can be solved in any coordinate system. However, if we represent  $X = (R, \Theta, \Phi)$  and  $x_0 = (r, \theta, \phi)$  in spherical coordinates, then the Jacobian  $\mathbf{D}$  is given for a launch point  $x_0$  and target point  $X$  on the sphere by the derivative  $(\partial X / \partial x_0)_R$  with  $R$  fixed. It is straightforward calculus to obtain this derivative by

$$(\partial X / \partial x_0)_R = (\partial X / \partial x_0) - (\mathbf{b}(X) / b_R(X)) \partial R / \partial x_0. \quad (***)$$

Using these formulas, the calculation of  $\mathbf{D}$  can be done in Cartesian coordinates  $X = (X, Y, Z)$  by integrating ODE (\*) to determine a field-line from launch to target point and then integrating the ODE (\*\*) twice. For the first integration of (\*\*), take the initial condition for the  $\phi$ -column vector of  $\mathbf{J}$  at the "launch point" to be

$$(\mathbf{J}_0)_{\phi} = \partial x_0 / \partial \phi = (-y_0, x_0, 0)^T$$

and integrate in  $s$  to get the  $\phi$  column  $(\mathbf{J}(s))_\phi = \partial \mathbf{X}(s)/\partial \phi$  for positive  $s$ . For the second integration, take initial condition for the  $\theta$ -column vector of  $\mathbf{J}$  at the "launch point" to be

$$(\mathbf{J}_0)_\theta = \partial \mathbf{x}_0 / \partial \theta = (x_0 z_0, y_0 z_0, -x_0^2 - y_0^2)^T / (x_0^2 + y_0^2)^{1/2}$$

and integrate in  $s$  to get the  $\theta$ -column  $(\mathbf{J}(s))_\theta = \partial \mathbf{X}(s)/\partial \theta$ . At the target point where the the field-line exits the sphere, one must exploit (\*\*\*) to convert these derivatives  $\partial \mathbf{X}/\partial \phi$ ,  $\partial \mathbf{X}/\partial \theta$  to derivatives  $(\partial \mathbf{X}/\partial \phi)_R$ ,  $(\partial \mathbf{X}/\partial \theta)_R$  at constant  $R$ , using  $R \partial R / \partial \mathbf{x}_0 = X \partial X / \partial \mathbf{x}_0 + Y \partial Y / \partial \mathbf{x}_0 + Z \partial Z / \partial \mathbf{x}_0$  to evaluate  $\partial R / \partial \phi$ ,  $\partial R / \partial \theta$ . Finally, to get derivatives of  $\Phi$ ,  $\Theta$  at constant  $R$ , use the standard cartesian to spherical transformations

$$d\Phi = (XdY - YdX)/(X^2 + Y^2)$$

and

$$d\Theta = (1/R) [XZ dX + YZ dY - (X^2 + Y^2) dZ] / (X^2 + Y^2)^{1/2}.$$

We implemented the above scheme numerically, solving the ODE's (\*),(\*\*) using a 1st-order Euler scheme (validated against the 2nd-order Heun scheme for selected points) with launch points distributed on the sphere. The  $\mathbf{B}$ ,  $\partial \mathbf{B} / \partial \mathbf{x}$  values required in (\*),(\*\*) were obtained from the MHD database, and interpolated with 5th-order splines to positions  $\mathbf{X}(s)$  of the numerical solution of (\*). In this way we obtain the Jacobian matrix  $D$  for any point on the surface of the sphere. However, to get the factor  $N_\perp^2$  one needs not only  $D$  but also the matrix  $G^\perp$ , and the latter has coordinate singularities at  $\theta=0, \pi$ . These singularities can be avoided by the use of a pair of overlapping spherical coordinate systems, as discussed in Titov (2007). This approach yielded accurate values of the perpendicular squashing factor  $Q_\perp$  on the surface of the sphere and values extended into the interior of the sphere as constants along the field-line between launch and target point.

However, to plot isosurfaces of  $Q_\perp$ , we need its values on a regular Cartesian grid. Thus, we chose a regular cubic grid of  $192^3$  points with spacing  $dx=2\pi/1024$  which contains the sphere and integrated (\*) to obtain the field-lines through each of these points. For each of the grid-points whose field-line entered the sphere we could integrate (\*\*) as described above to obtain a value of  $Q_\perp$  at that point. If the field-line through the grid-point did not enter the sphere, then we assigned the minimum possible value  $Q_\perp=2$  to that point. This procedure was employed to create Fig.4 in the Letter and the 3DPDF's discussed here, which plot the  $Q_\perp=32$  isosurface. We found that the structure of this "quasi-separatrix layer" (QSL) is relatively insensitive to the precise level value employed, with the QSL becoming a bit thicker for  $Q_\perp < 32$  and a bit thinner for  $Q_\perp > 32$ . It is worth noting that there is some additional structure in our QSL besides the standard "X" shaped structure, which is due to large values of  $Q_\perp$  for field lines entering or exiting the sphere

tangentially, at points where  $B_r=0$ . This is analogous to the case of the “polarity inversion line” on the photosphere in the case of reconnection in the solar corona, as discussed by Titov (2007). However, for our problem the sphere is chosen purely by convention and has no objective physical significance. Thus the large  $Q_{\perp}$  values arising from the points on the sphere where  $B_r=0$  can be regarded as “spurious”. These large values are also unavoidable, however, for any closed surface. The absence of magnetic monopoles implies that there must be a curve on any closed surface where the normal component  $B_n$  changes sign, i.e.  $B_n=0$ . Thus, these additional contributions to the QSL can only be eliminated by considering the squashing factor for field-line mappings from one open surface to another open surface. In any case, our QSL defined for the sphere-to-sphere field-line mapping suffices to reveal the main “X” shaped structure.

The “hyperbolic flux tube” (HFT) is defined as the union of the centers of all of the “X”s in the QSL. We determined the length of the HFT by finding the cross-section of the QSL in cutting planes normal to the M-axis of the minimum-variance frame (see discussion of Figure 3). By varying the offset of the cutting plane, we could determine the range over which the “X” structure existed as about 0.54, which we take as the length of the HFT. Furthermore, the direction of the HFT as determined by the end-to-end vector between the centers of the extreme “X”s has an angle of about  $35^\circ$  with respect to the M-axis. We note here that for a certain narrow range of offsets there appear to be two “X”s in the cutting plane. Examination of the 3DPDF shows that the second apparent “X” is due to the fact that one of the “sheets” of the QSL (corresponding to the bottom left arm of the “X” in Fig.4) is non-planar and folds downward and over toward another “sheet” (corresponding to the bottom right arm of the “X” in Fig.4).

For readers who may wish to manipulate 3D Figure 4 and the additional two 3D plots of the QSL in Acrobat Reader, we provide here a list of all objects in those 3DPDF’s as they appear under Toggle Model Tree.

|             | <b>Fig4_3D</b> | <b>QSL_and_current</b> | <b>QSL_and_lines</b> |
|-------------|----------------|------------------------|----------------------|
| QSL         | Surf3_8        | Surf3_7                | Surf3_1              |
| current     | NA             | Surf3_8                | NA                   |
| field-lines | NA             | NA                     | Plot_4-Plot_67       |
| x-axis      | Plot_40        | Plot_37                | Plot_1               |
| y-axis      | Plot_41        | Plot_38                | Plot_2               |
| z-axis      | Plot_42        | Plot_39                | Plot_3               |
