# Supplementary material for: Inertial-Range Reconnection in Magnetohydrodynamic Turbulence and in the Solar Wind
Source: arXiv:1503.00509 ancillary file (2015-03-02)

## MHD Event Catalogue Documentation

The MHD Event Catalogue contains the simulated “spacecraft data” for the 27 events that we identified in a representative sample from the MHD turbulence database which satisfy our modified Gosling criterion.

We searched the initial  $1024^3$  time-slice  $t=0$  in the MHD database and along  $3 \times 4^3=192$  linear cuts through that time-slice in the 3 coordinate directions. The cuts were chosen semi-randomly, with each square face of the computational cube divided first into a  $4^2$  regular lattice and then small random perturbations added to each lattice point to determine the center of a cut perpendicular to that face. The random perturbations were added to avoid intersections of the linear cuts, so as to sample independent events.

The “modified Gosling criterion” that we employed was as follows: At each point  $x$  in the sampled linear cut we calculated the magnetic field and velocity increments across a fixed separation distance  $r$ , as follows

$$\delta \mathbf{B}(1) = \mathbf{B}(x+r/2) - \mathbf{B}(x-r/2), \quad \delta \mathbf{u}(1) = \mathbf{u}(x+r/2) - \mathbf{u}(x-r/2),$$

where the label “1” for the point  $x$  indicates that this is the “first point” considered. We then searched for a “second point” labelled 2, by examining all  $x'$  satisfying  $x < x' < s$ , with increments defined similarly as

$$\delta \mathbf{B}(2) = \mathbf{B}(x'+r/2) - \mathbf{B}(x'-r/2), \quad \delta \mathbf{u}(2) = \mathbf{u}(x'+r/2) - \mathbf{u}(x'-r/2).$$

We then selected pairs of points 1,2 which satisfy all of the following criteria:

- (i)  $|\delta \mathbf{B}(1)| > thresh, |\delta \mathbf{u}(1)| > thresh$
- (ii)  $|\delta \mathbf{B}(2)| > thresh, |\delta \mathbf{u}(2)| > thresh$
- (iii)  $\delta \mathbf{B}(1) \cdot \delta \mathbf{B}(2) > 0$
- (iv)  $\delta \mathbf{u}(1) \cdot \delta \mathbf{u}(2) < 0$
- (v)  $(\delta \mathbf{B}(1) \cdot \delta \mathbf{u}(1)) \times (\delta \mathbf{B}(2) \cdot \delta \mathbf{u}(2)) < 0$

The conditions (i-ii) set a minimum threshold value, *thresh*, on the magnitudes of the increments at both points. The condition (iii) requires that increments in  $\mathbf{B}$  be aligned at the points 1,2, while condition (iv) requires that increments in  $\mathbf{u}$  be anti-aligned at these two points. The condition (v) requires that increments in  $\mathbf{u}$  and  $\mathbf{B}$  must be aligned at one point and anti-aligned at the other. This last condition is redundant if the increments are achieved mainly by the change of a single component, for then (v) follows from (iii-iv).

These conditions are similar to those applied by Gosling to the solar wind data; see the review of Gosling (2012). In particular, (v) corresponds to Gosling’s requirement that candidate reconnection events should be “bounded by correlated changes in the dominant components of velocity,  $\mathbf{V}$ , and magnetic field,  $\mathbf{B}$ , on one side and anti-correlated changes in the dominant components of  $\mathbf{V}$  and  $\mathbf{B}$  on the other side.” This condition, however, is completely symmetrical in velocity and magnetic fields, so that it allows events with large “reversals” in velocity and “jets” in magnetic field. Thus, it is better to apply conditions (iii) and (iv), which select for “reversals” in  $\mathbf{B}$  and “jets” in  $\mathbf{u}$ .

## MHD Event Catalogue Documentation

The main difference of our criterion from Gosling's is that we require  $r$  to be a sizable fraction of the integral length  $L$ , so that we allow the large field increments at points 1,2 to be achieved more gradually, over inertial-range length-scales. For our specific results in this catalogue and in the Letter, we chose  $r=6*dx$  or about  $1/10$  of the magnetic integral length  $L=0.35$ . We also allowed the two points 1,2 to be separated by a distance up to  $s=32*dx$  or about  $L/2$ , in order to capture very large-scale events with widths of nearly an integral-scale length. Our imposed threshold on the increment magnitudes was 2 times the rms value of  $|\delta \mathbf{B}|$  at separation  $r=6*dx$ , or  $thresh=0.4$ .

To avoid multiple occurrences of the same event in our catalogue, we applied a simple clustering algorithm: whenever our criterion was satisfied by two pairs of points 1,2 and 1',2' we considered them part of the same "cluster" if 1 and 1' were separated by a single grid space  $dx$ . We found that clustering the observations in this manner largely eliminated multiple appearances of the same event in our catalogue. Each "cluster" consists of all grid points extending from the first 1-point to the final 2-point in the event.

In the catalogue we show all 27 "clusters" found by our algorithm in the 192 linear cuts, one cluster per page. The  $(x,y,z)$  coordinate of the center of each cluster are listed at the top of the page. The direction of the cut is indicated by the labels on the abscissa of each plot, either "x", "y" or "z". The top panels show the raw data for the three field components, with red for x-component, green for y-component, and blue for z-component, with magnetic fields on the left and velocity fields on the right. The bottom panels show the components rotated into a minimum-variance frame (MVF) of the magnetic field, calculated over all the points of the "cluster", with red for L-component (maximum variance), green for M-component (median variance), and blue for N-component (minimum variance). All of the (1,2) point-pairs in the cluster are plotted on the abscissa, with green asterisks \* for 1-points and red asterisks \* for 2-points.

The event discussed in detail in the Letter appears as cluster 25 in the catalogue. There are many other events in the catalogue that appear quite similar to this one, e.g. clusters 1, 4, 6, 10, 13, 15, 17, 19, 20, 21, 24. There are also several events that appear more like those selected by Gosling, with relatively sharp magnetic field rotations at the boundaries of the event and with a "plateau" region of intermediate magnetic field rotation inside. For example, clusters 2, 9, 11, 18, 22, 23, 27 all show such "Gosling-like" features. The above identified events in the MHD turbulence database all appear as plausible candidates for large-scale reconnection and are interesting for further detailed study.

(0.3068, 1.4419, 2.0862)

Magnetic Fields

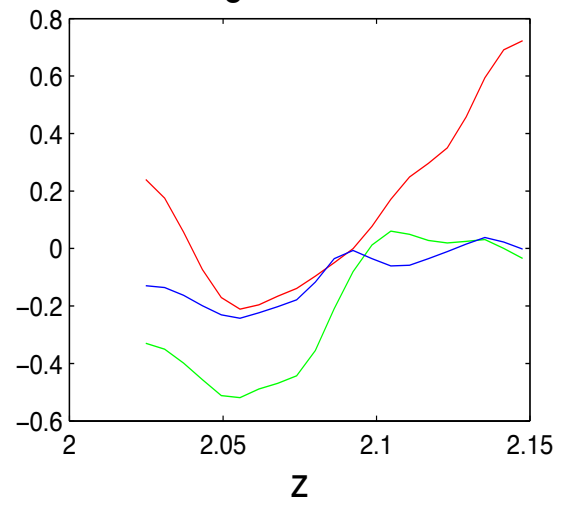

Velocity Fields

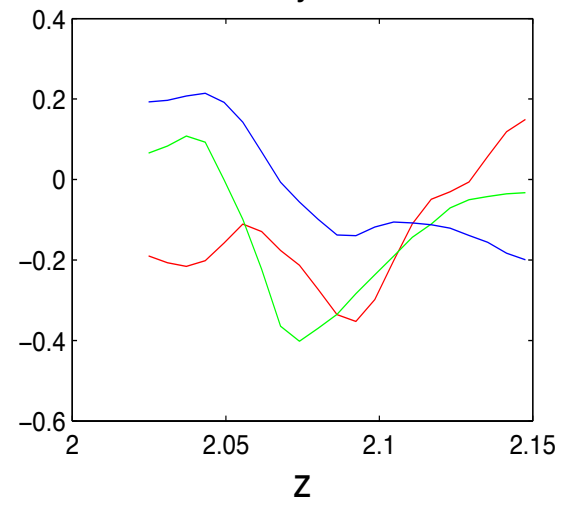

Magnetic Field Rotated

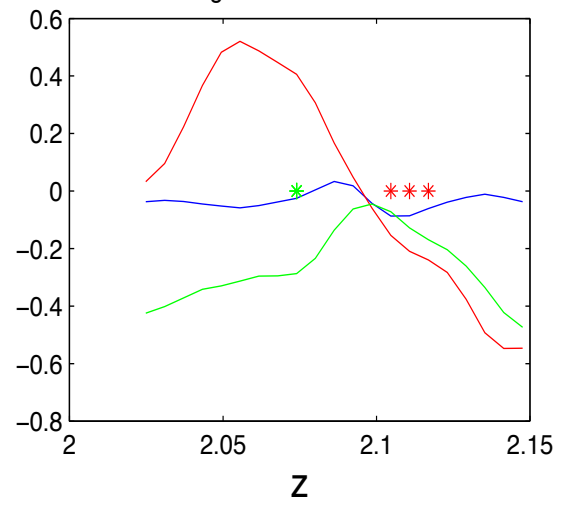

Velocity Field Rotated

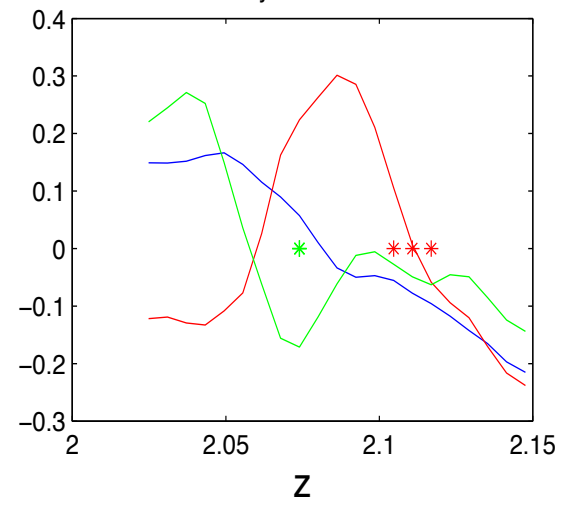

ns=32, cluster 1

(1.2088, 5.0253, 5.3137)

Magnetic Fields

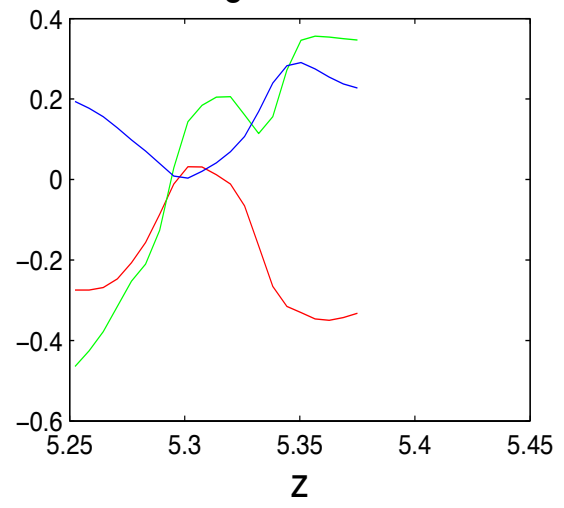

Velocity Fields

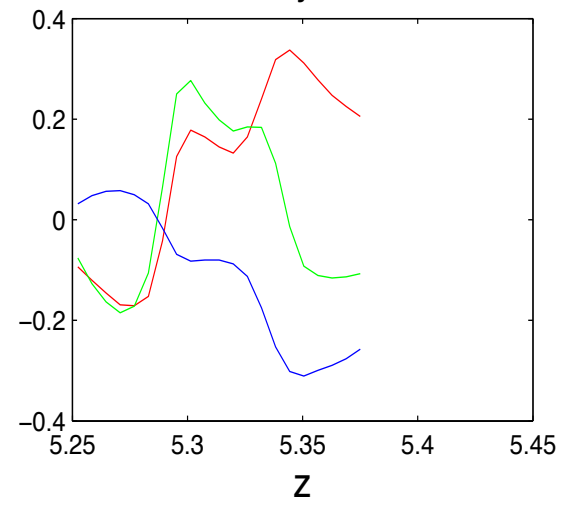

Magnetic Field Rotated

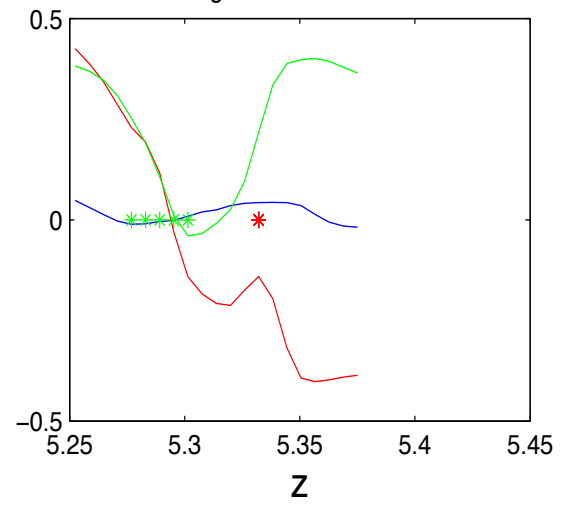

Velocity Field Rotated

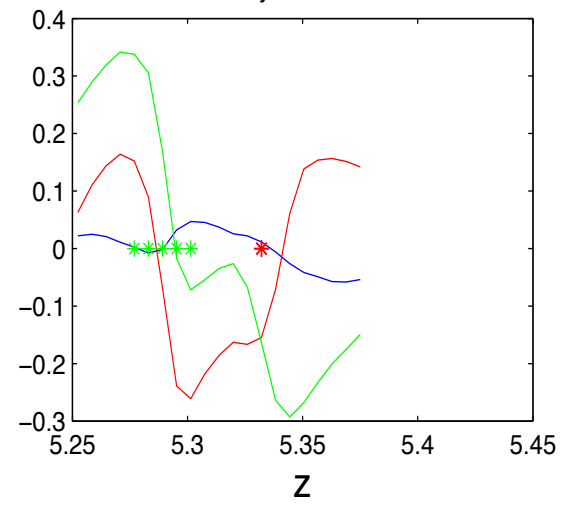

ns=32, cluster 2

(3,1293,5.0253,1.985)

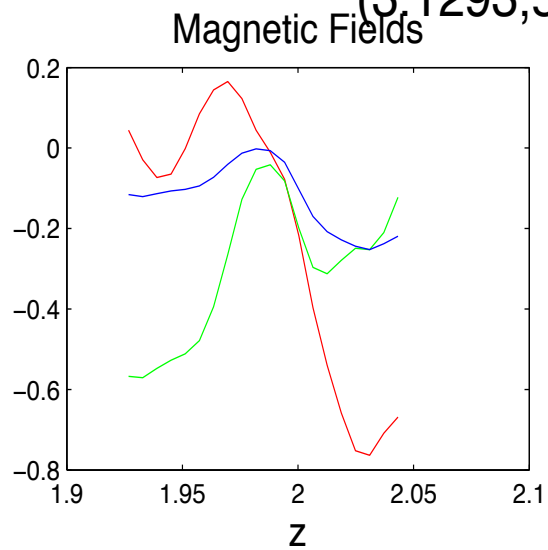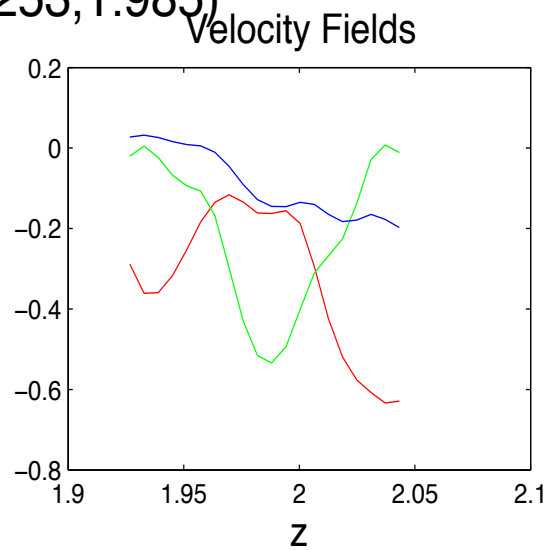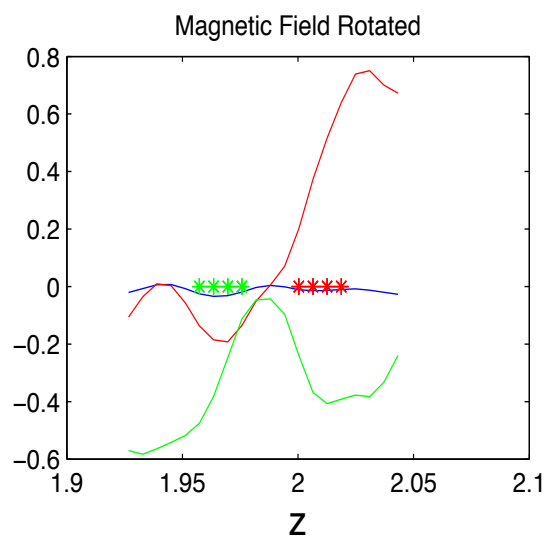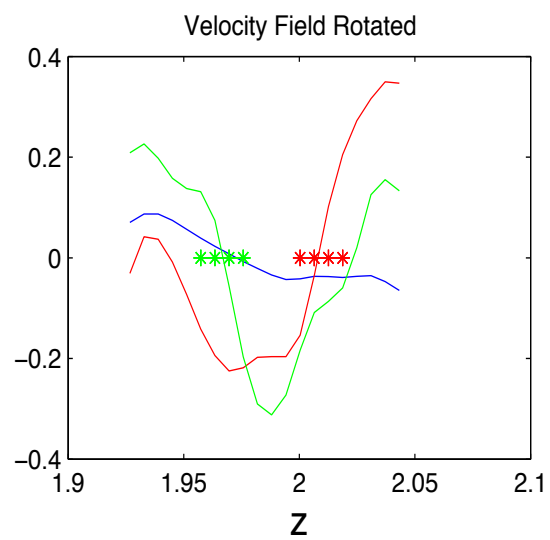

ns=32, cluster 3

(3.43,2.9637,5.0192)

Magnetic Fields

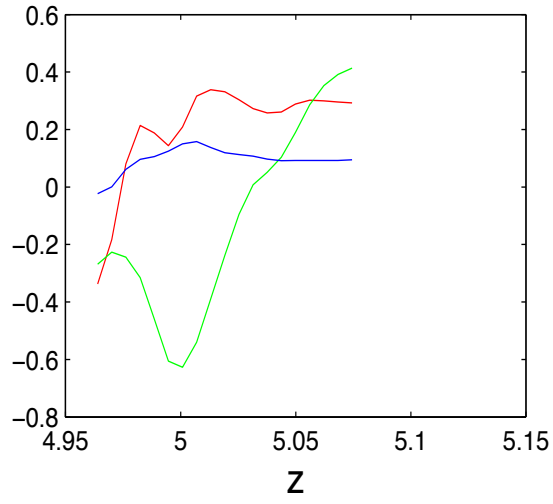

Velocity Fields

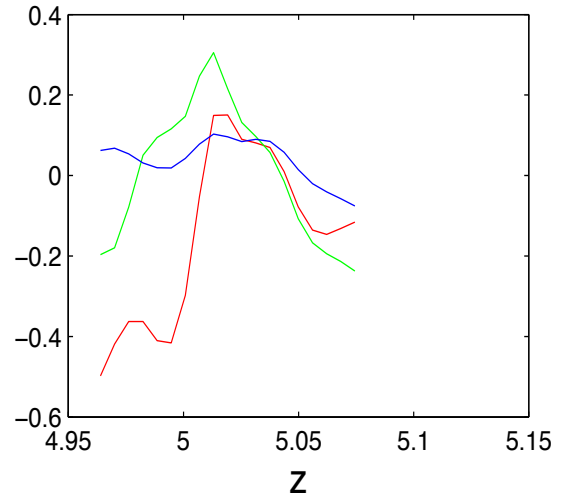

Magnetic Field Rotated

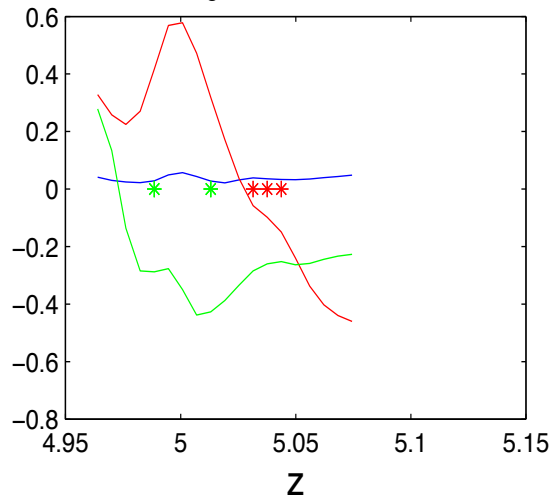

Velocity Field Rotated

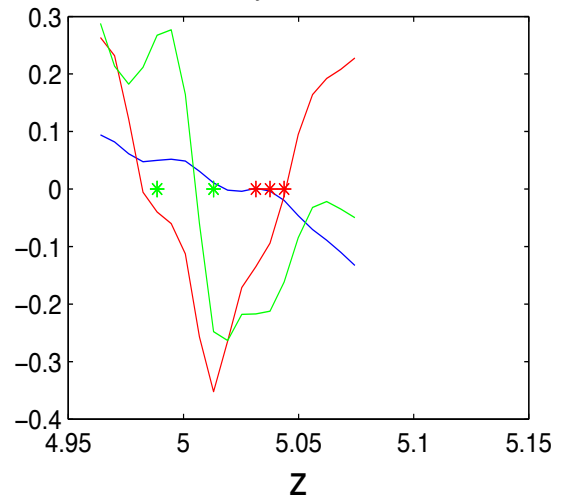

ns=32, cluster 4

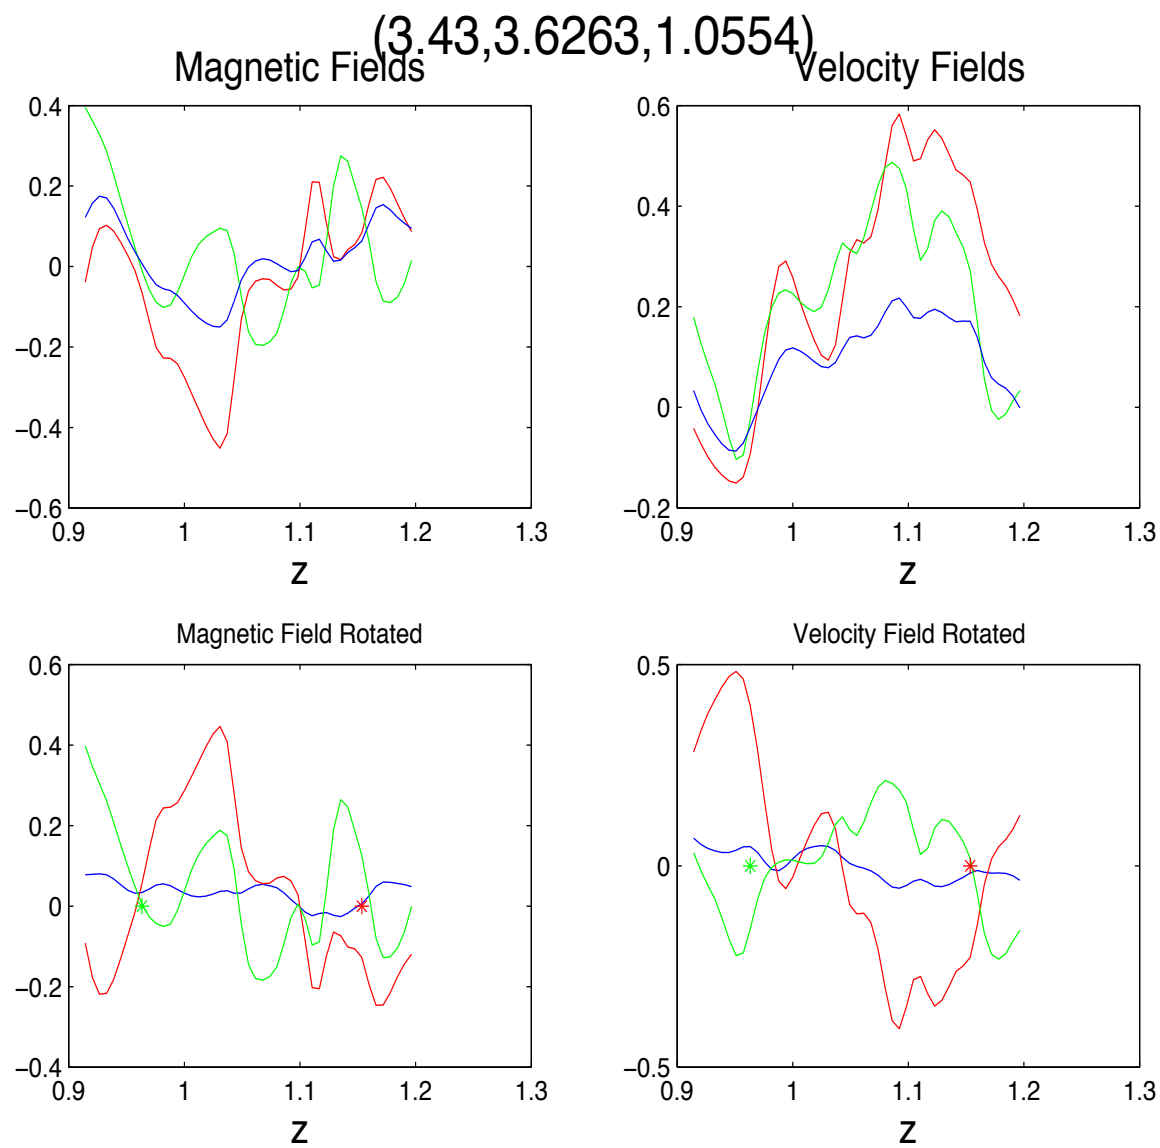

ns=32, cluster 5

(4.6204, 2.9637, 4.1264)

Magnetic Fields

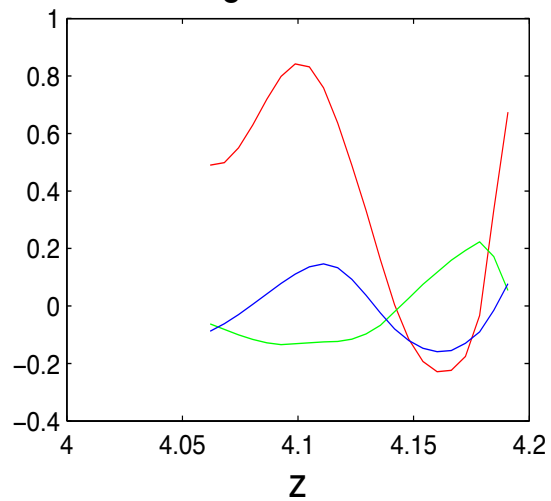

Velocity Fields

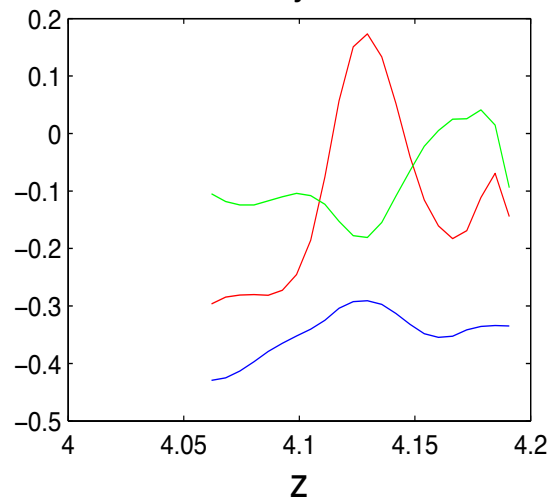

Magnetic Field Rotated

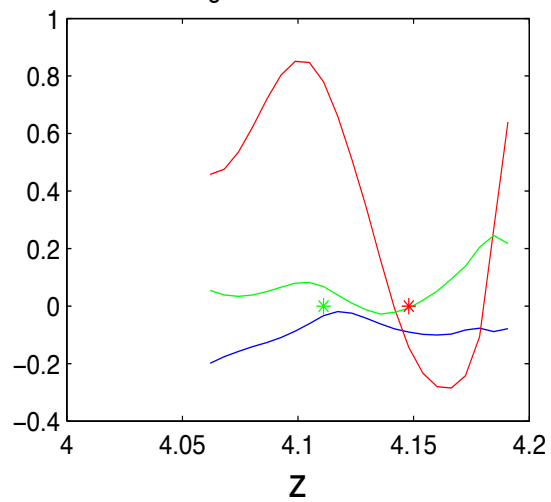

Velocity Field Rotated

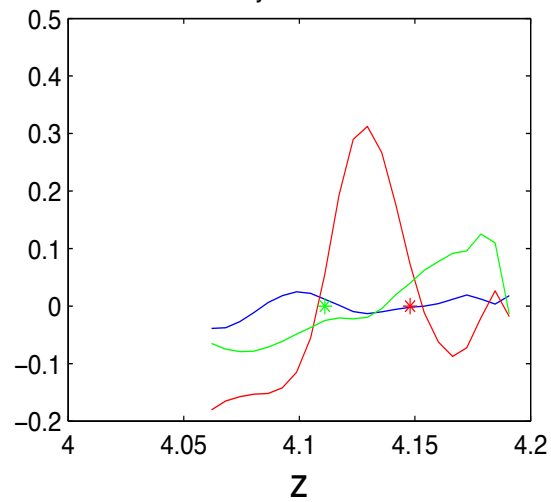

ns=32, cluster 6



(4.6204, 3.6263, 0.81915)

Magnetic Fields

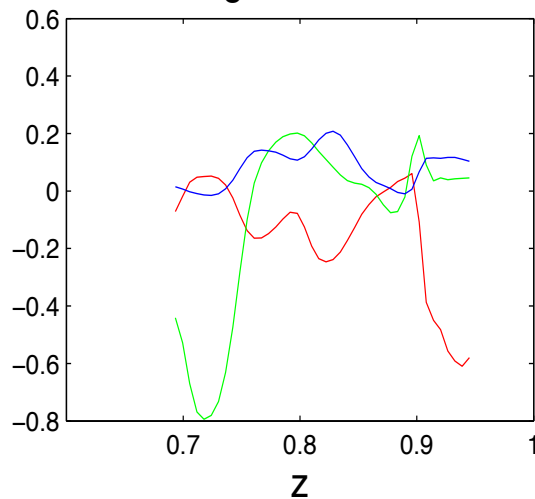

Velocity Fields

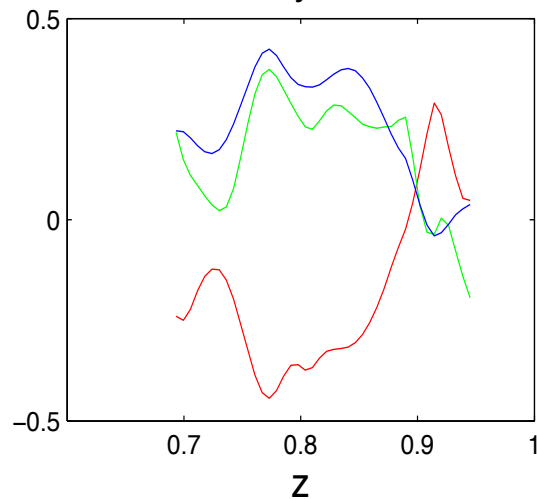

Magnetic Field Rotated

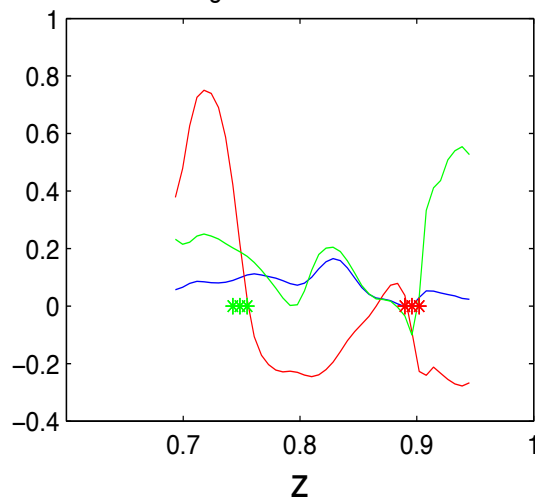

Velocity Field Rotated

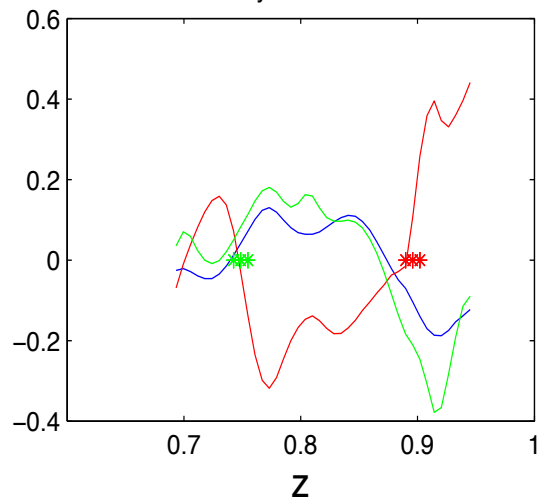

ns=32, cluster 7

(4.6204, 5.9703, 0.51235)

Magnetic Fields

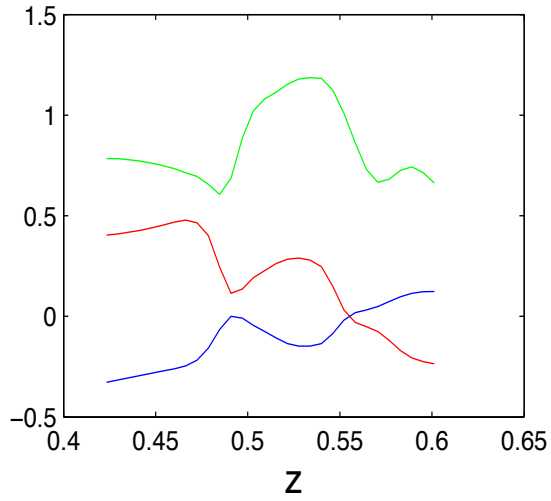

Velocity Fields

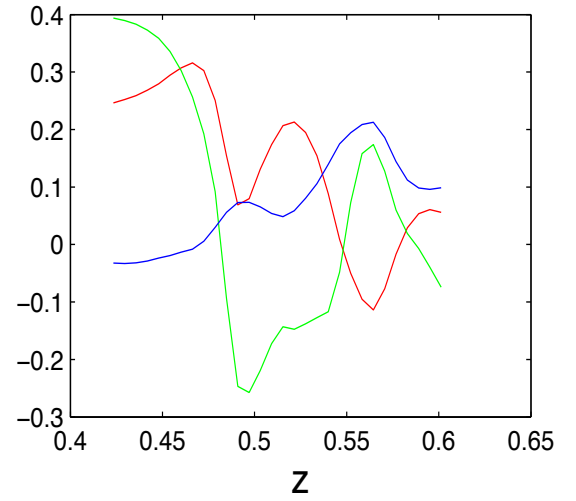

Magnetic Field Rotated

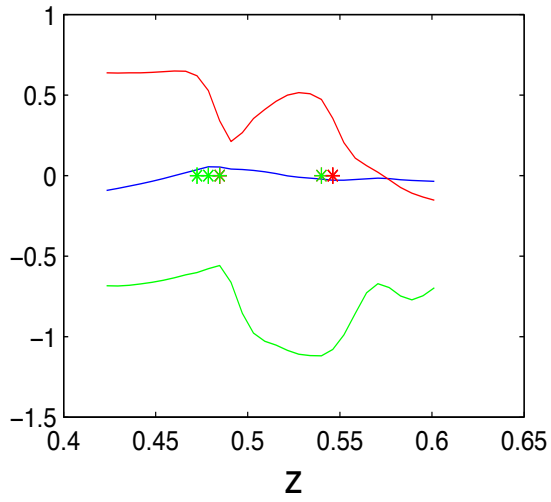

Velocity Field Rotated

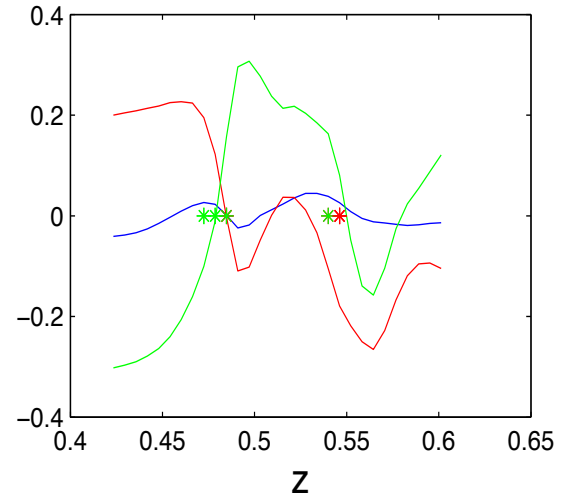

ns=32, cluster 8

(5.0744, 1.9819, 5.2616)

Magnetic Fields

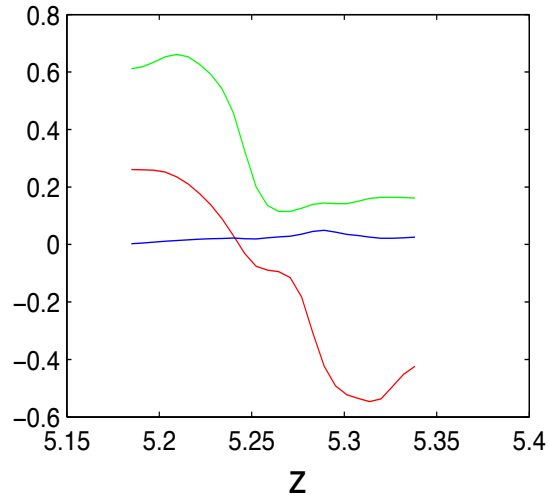

Velocity Fields

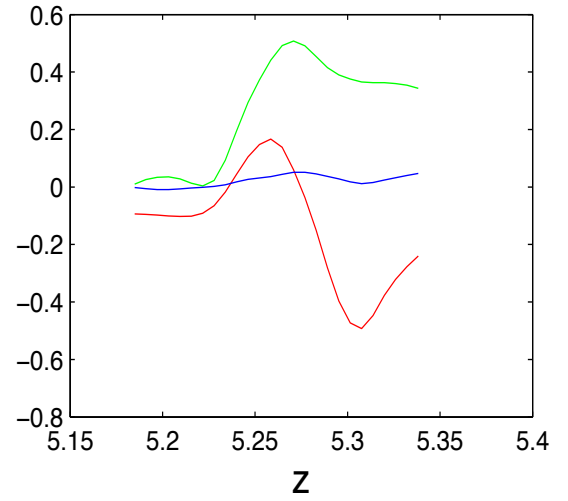

Magnetic Field Rotated

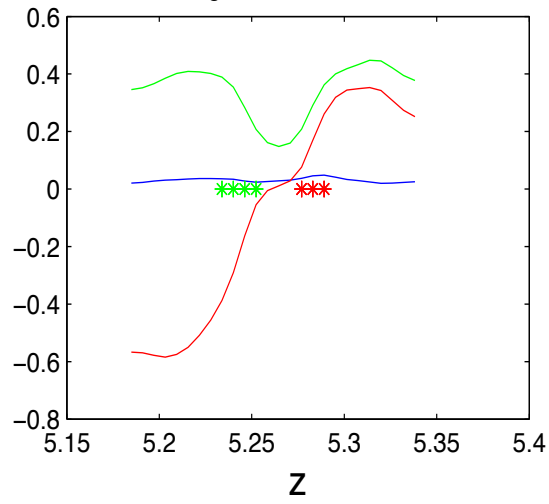

Velocity Field Rotated

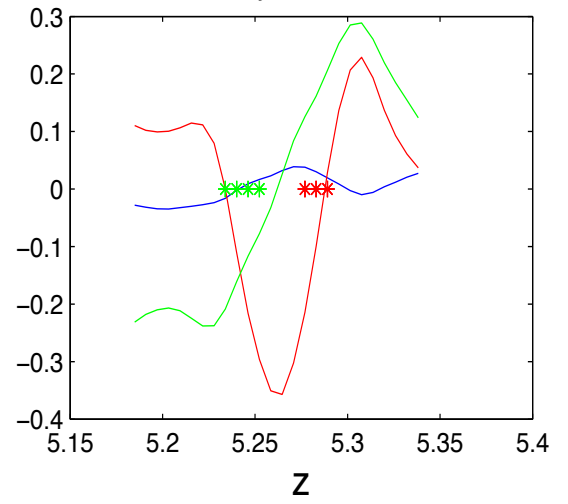

ns=32, cluster 9

(5.8414, 3.6263, 1.1965)

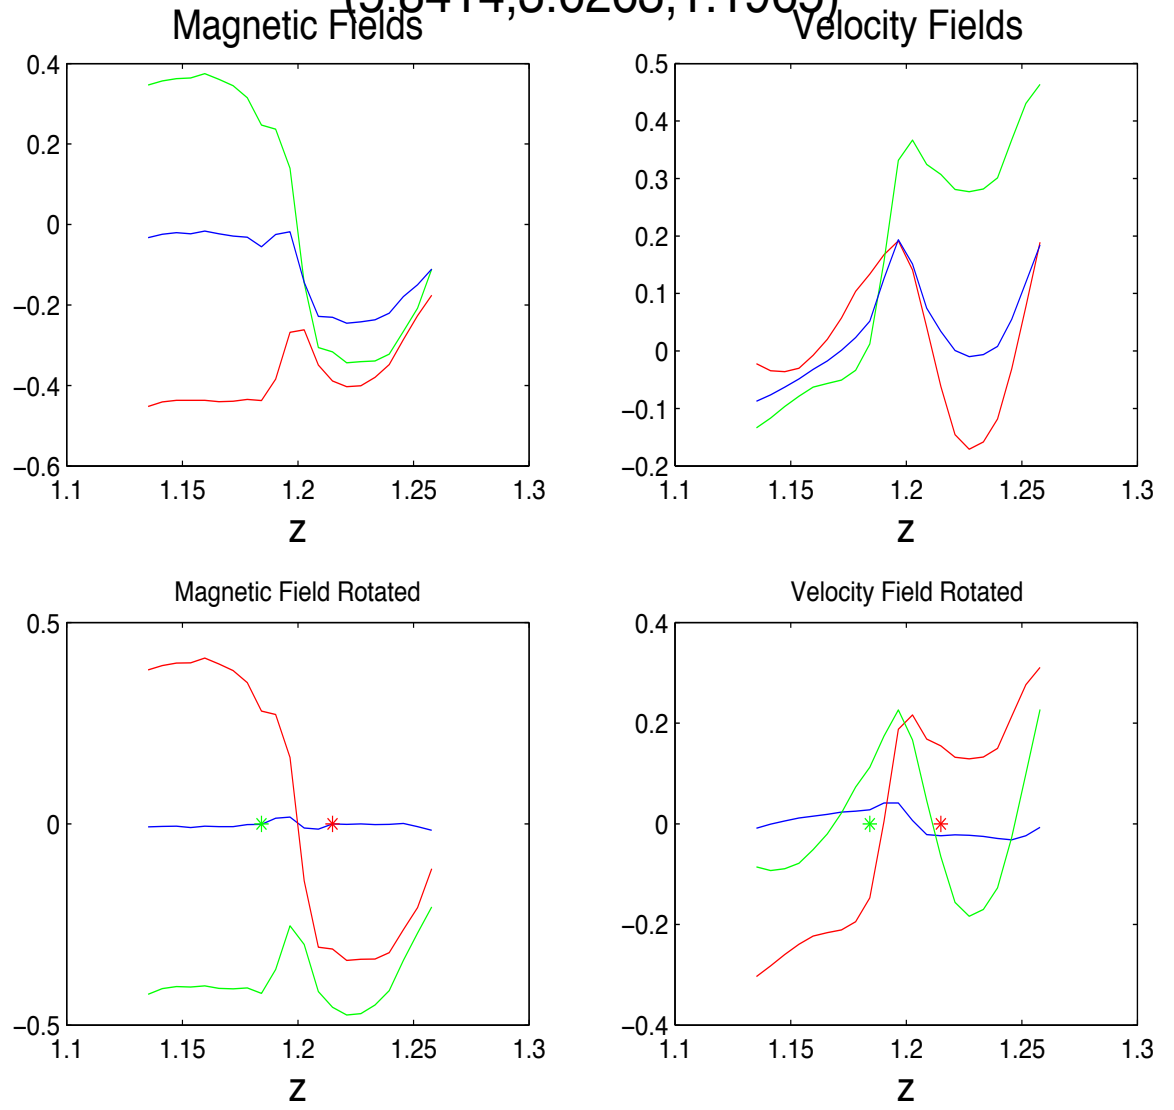

ns=32, cluster 10

(5.8414, 3.6263, 3.0465)

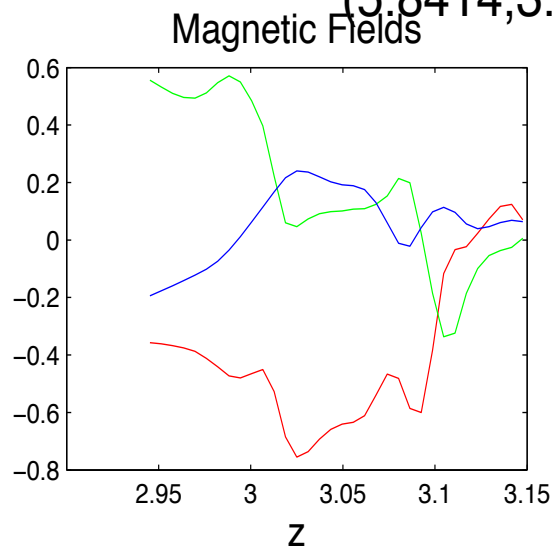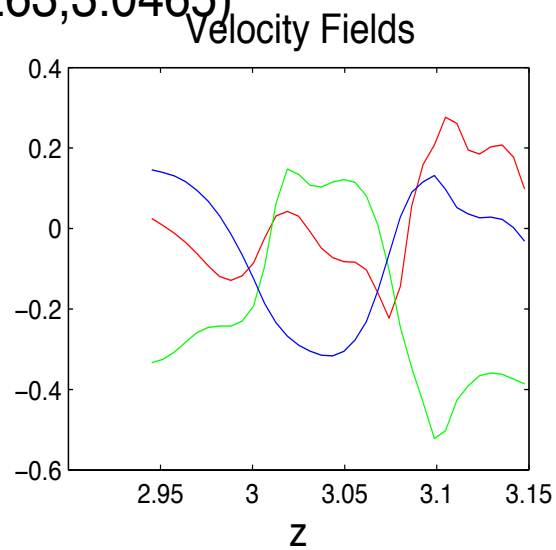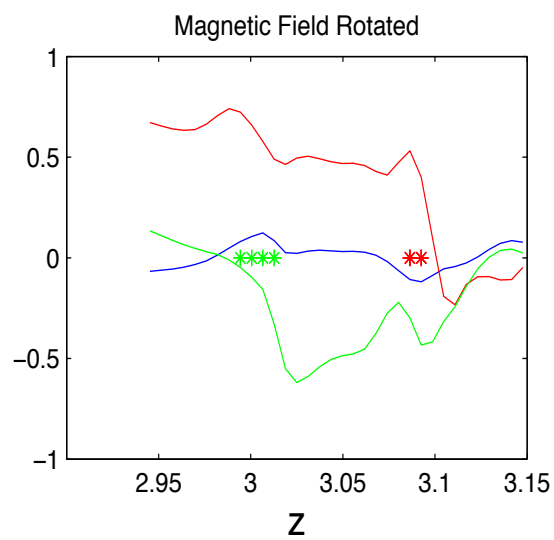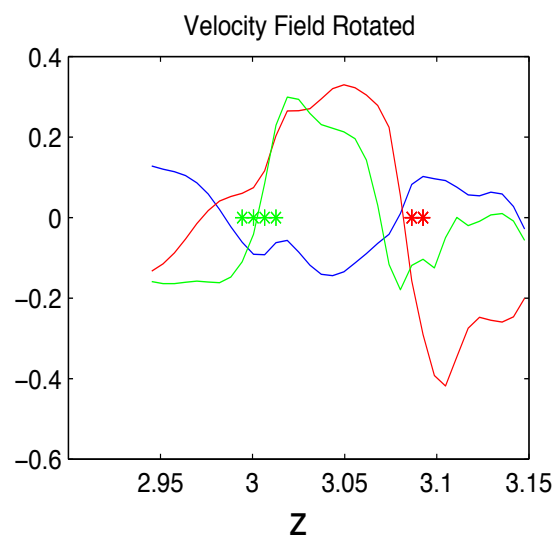

ns=32, cluster 11

(5.8414, 3.6263, 3.1477)

Magnetic Fields

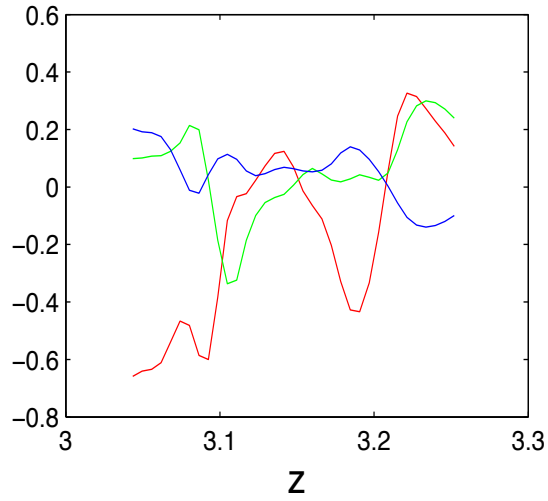

Velocity Fields

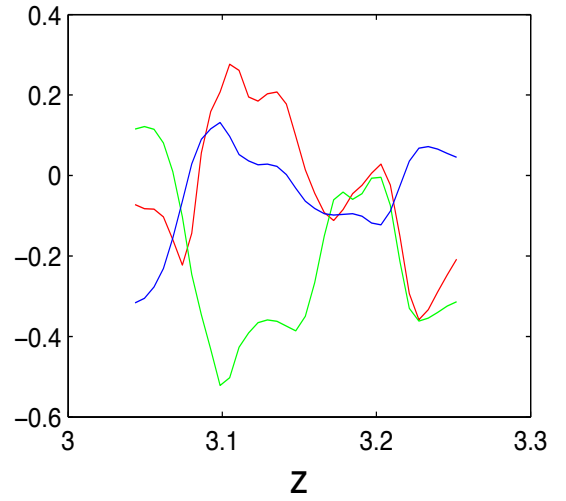

Magnetic Field Rotated

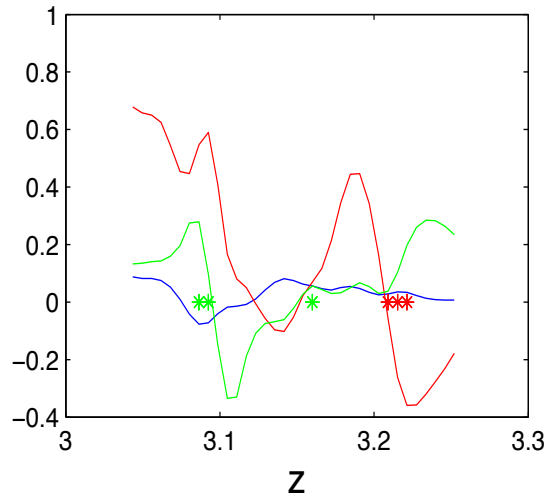

Velocity Field Rotated

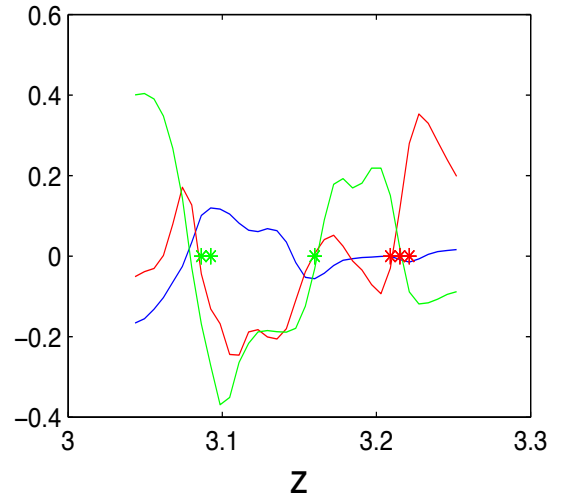

ns=32, cluster 12

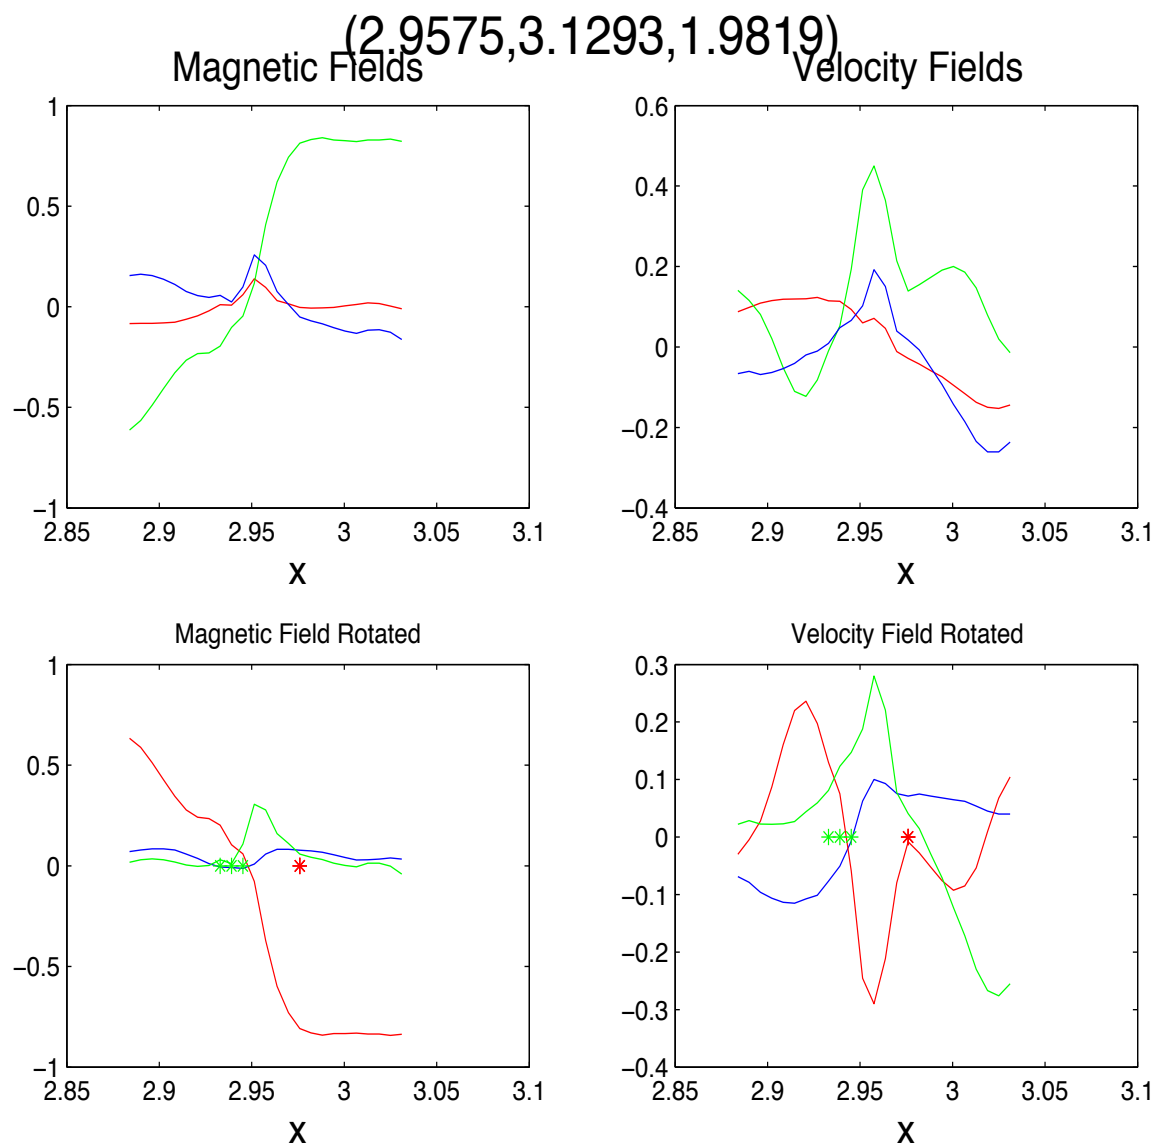

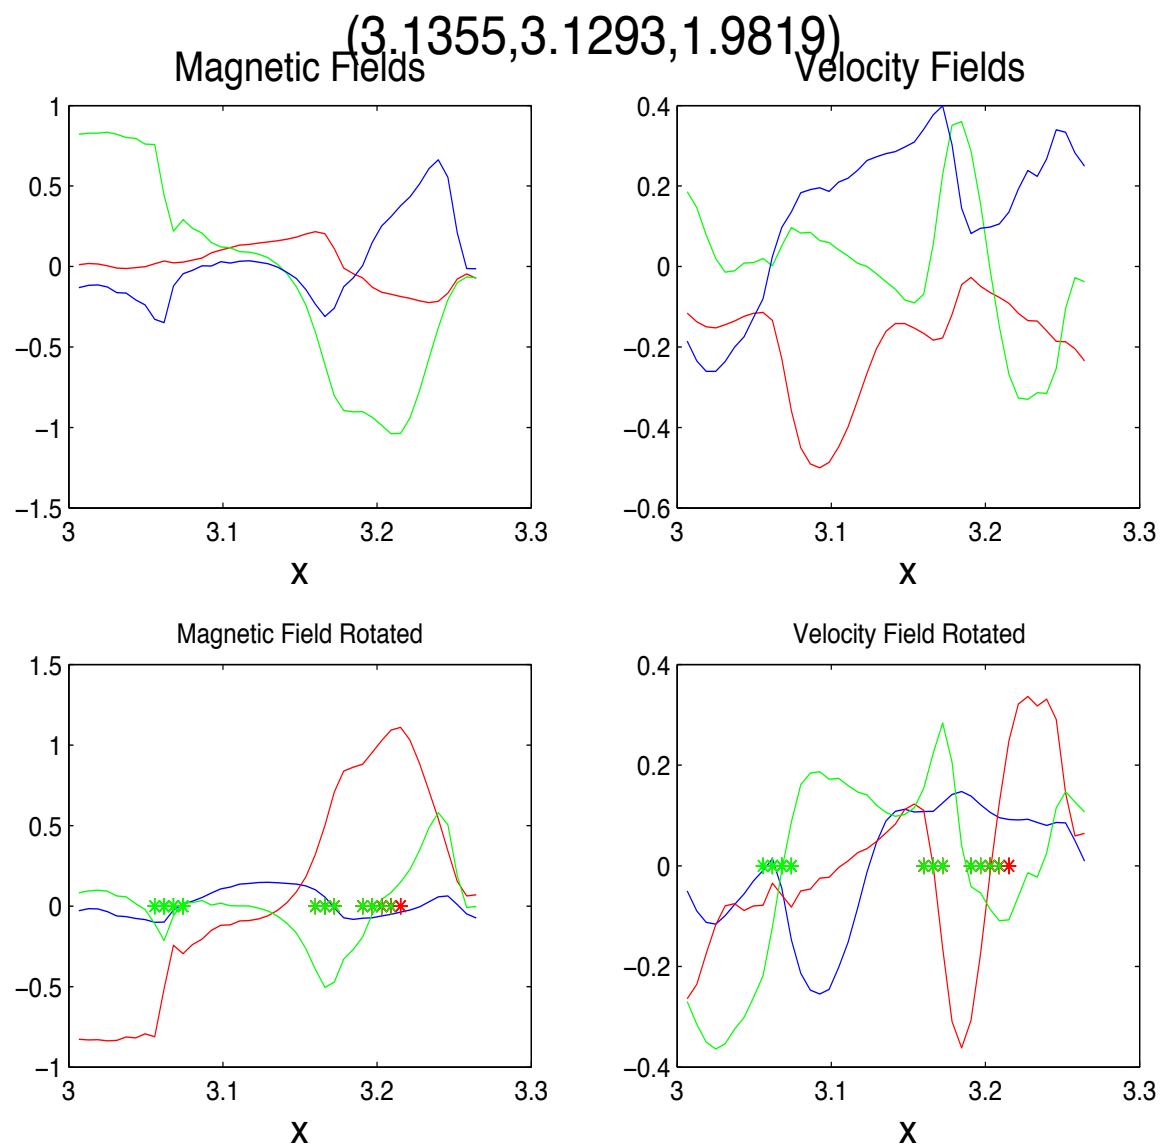

ns=32, cluster 14



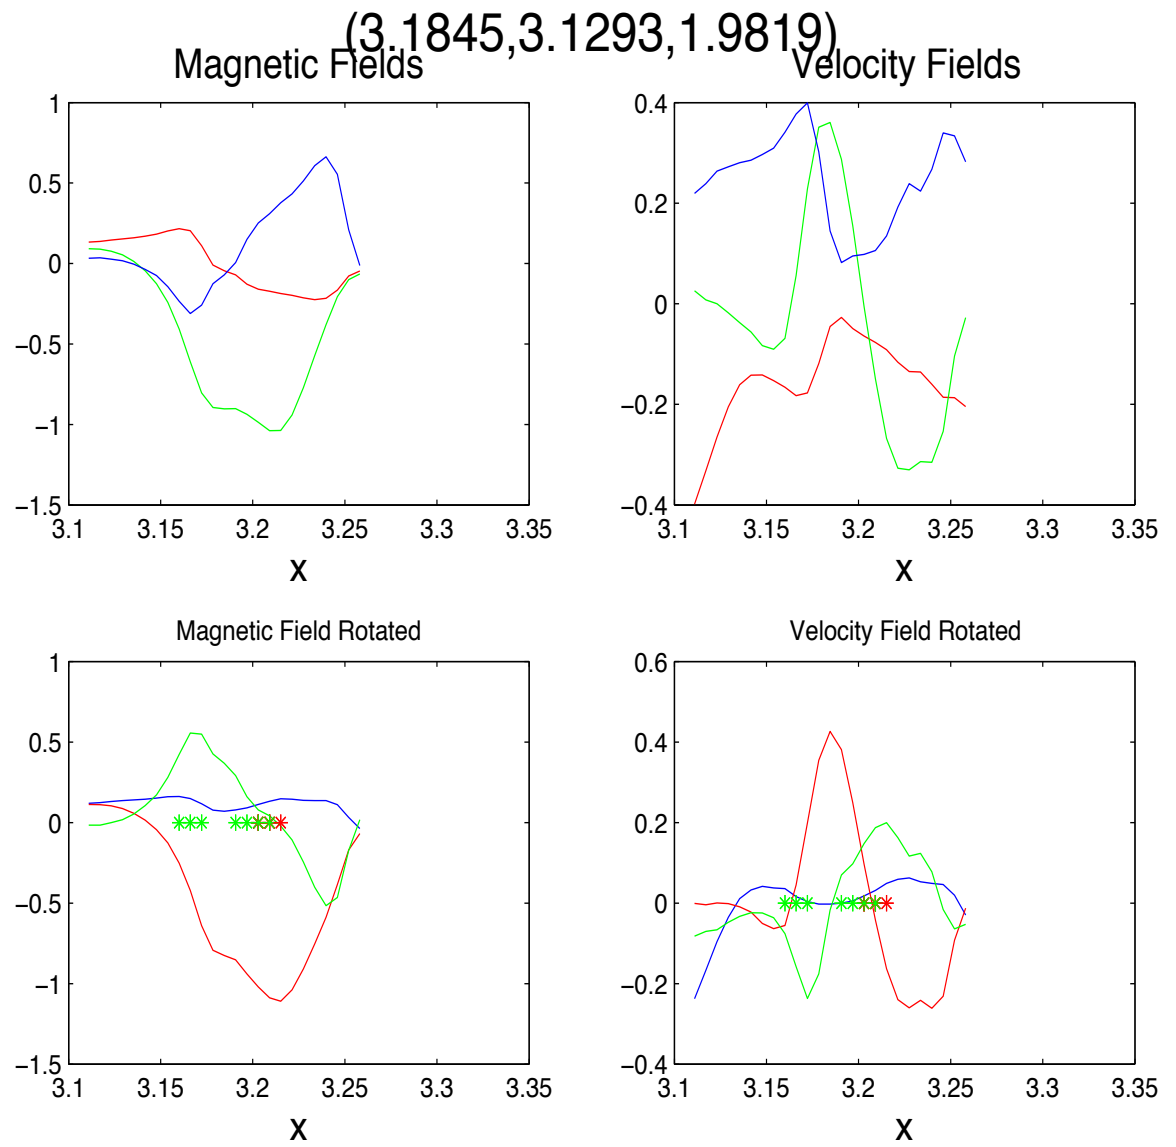

ns=32, cluster 15

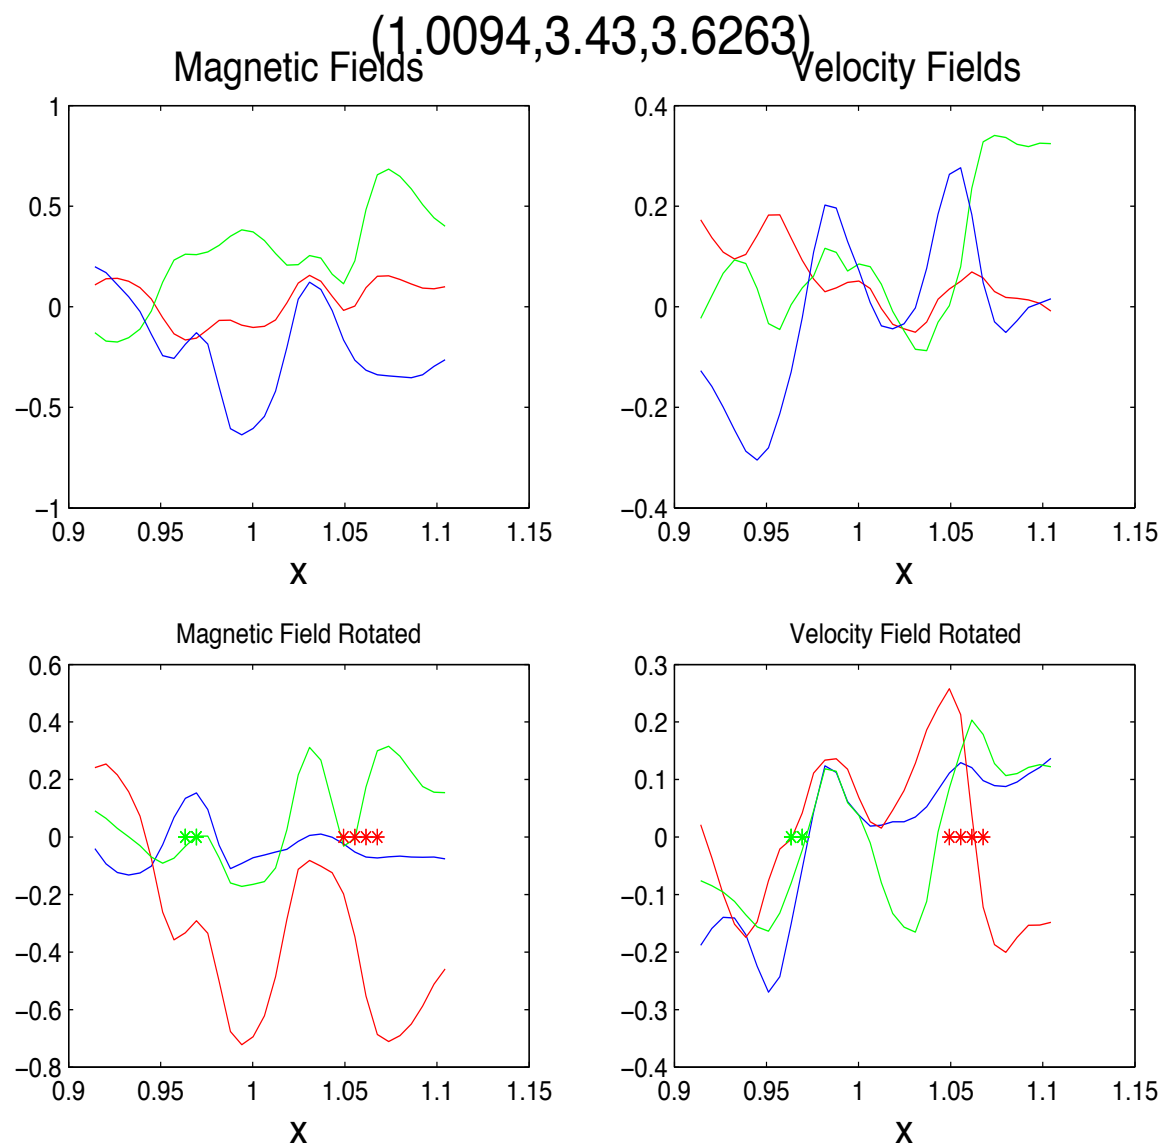

ns=32, cluster 16

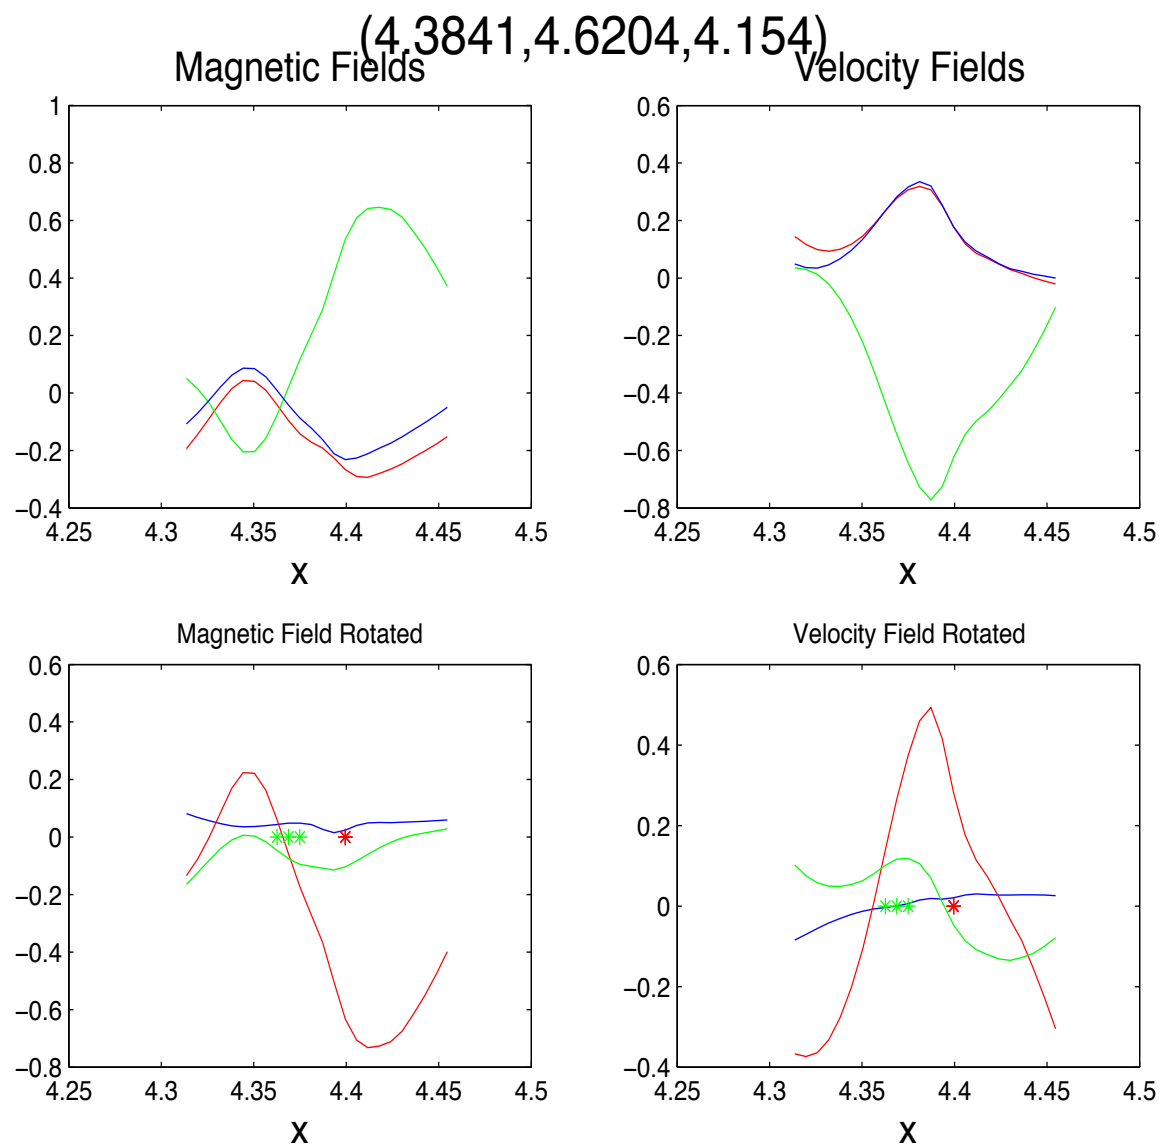

ns=32, cluster 17

(4.829, 5.0744, 3.6263)

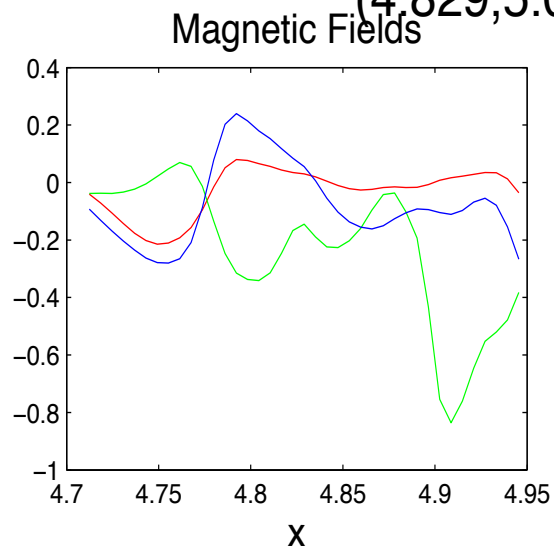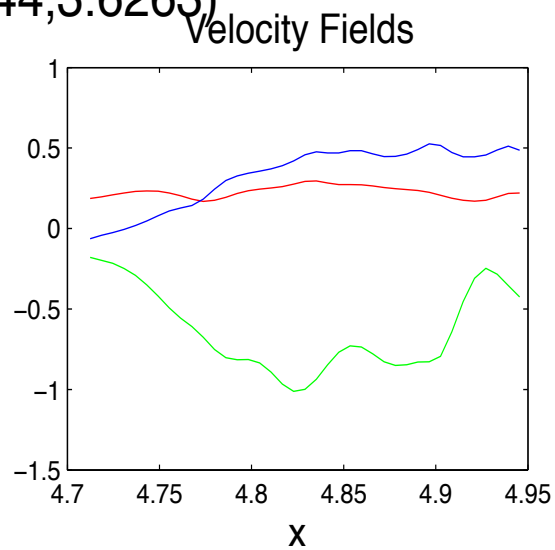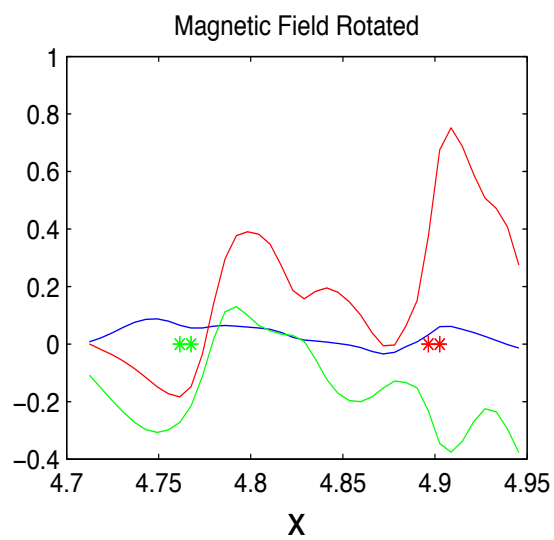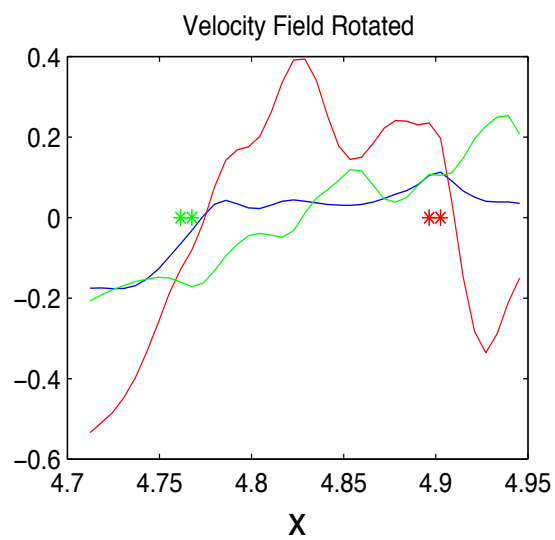

ns=32, cluster 18

(1.6598, 5.0744, 5.0253)

Magnetic Fields

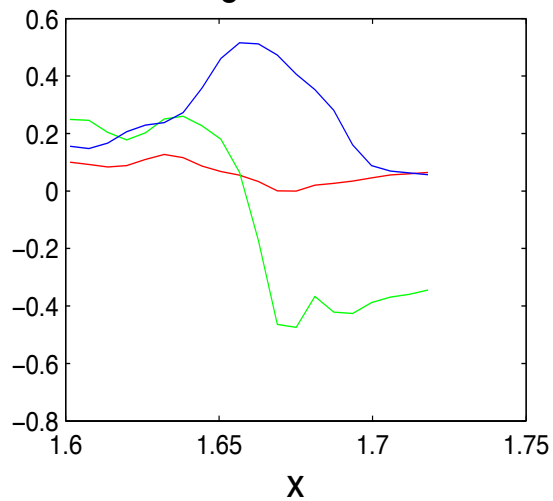

Velocity Fields

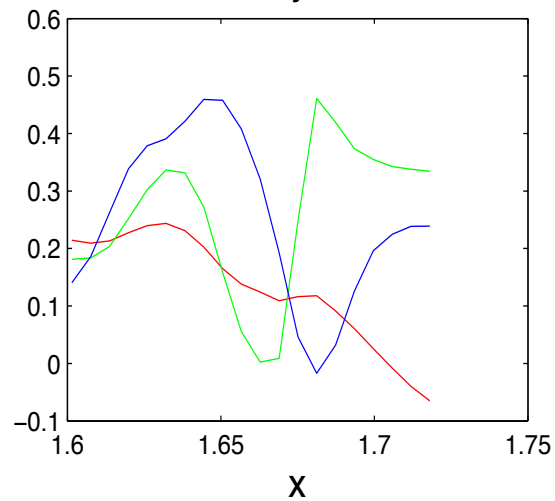

Magnetic Field Rotated

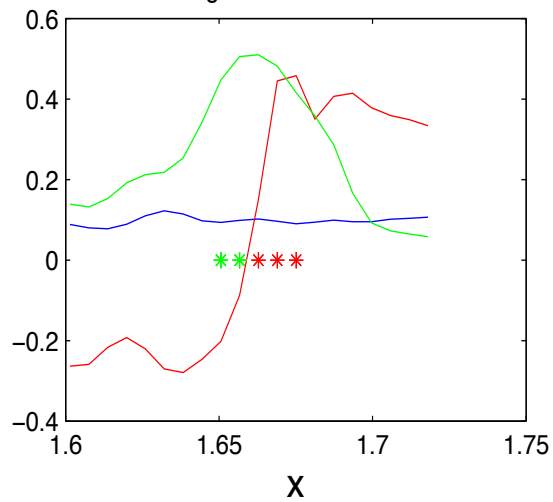

Velocity Field Rotated

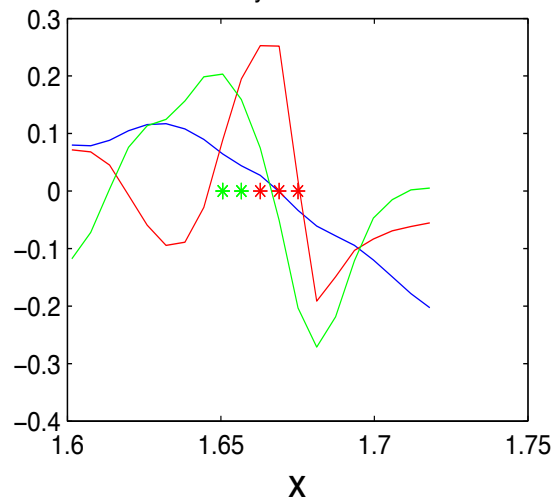

ns=32, cluster 19

(3.9024, 5.8414, 1.4419)

Magnetic Fields

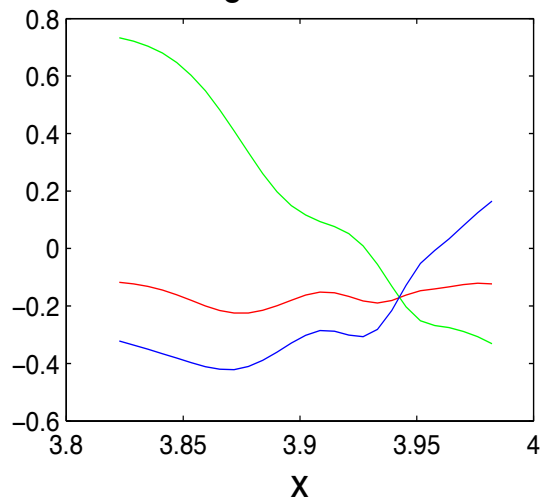

Velocity Fields

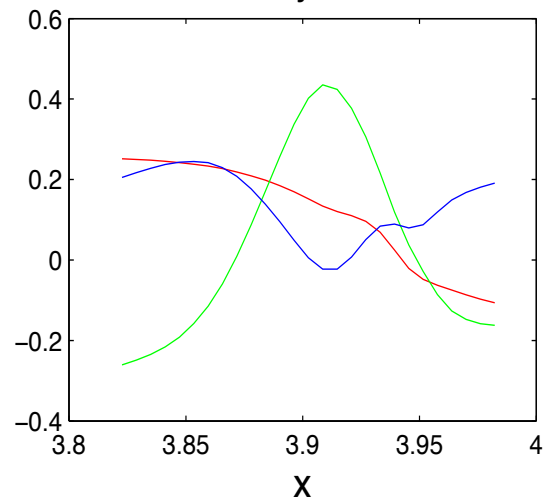

Magnetic Field Rotated

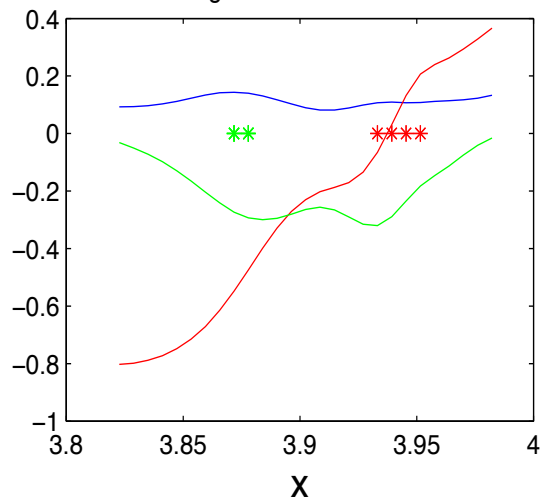

Velocity Field Rotated

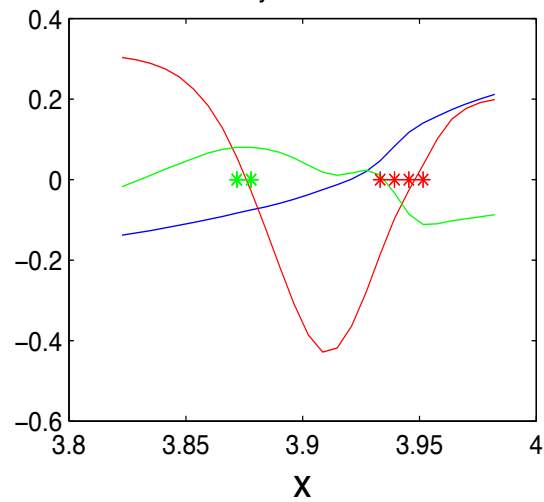

ns=32, cluster 20

(0.58905, 4.5498, 3.43)

Magnetic Fields

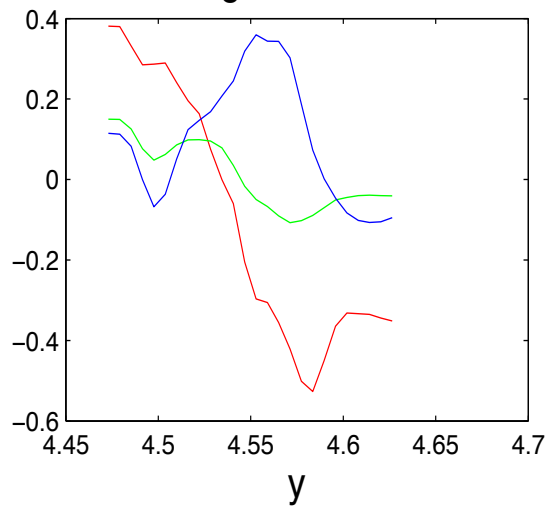

Velocity Fields

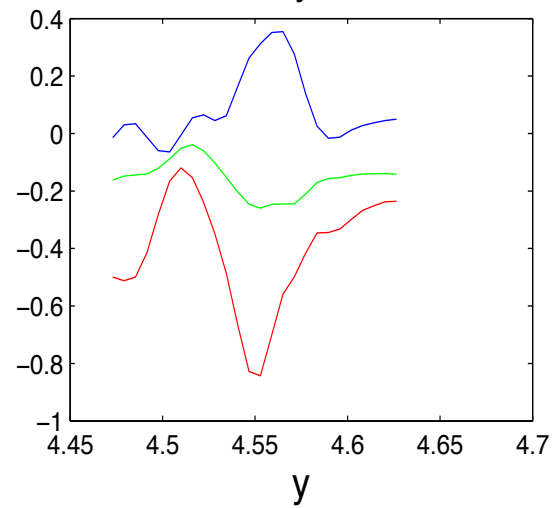

Magnetic Field Rotated

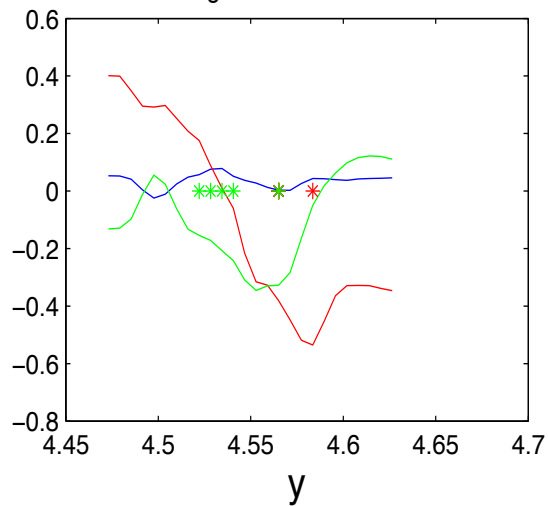

Velocity Field Rotated

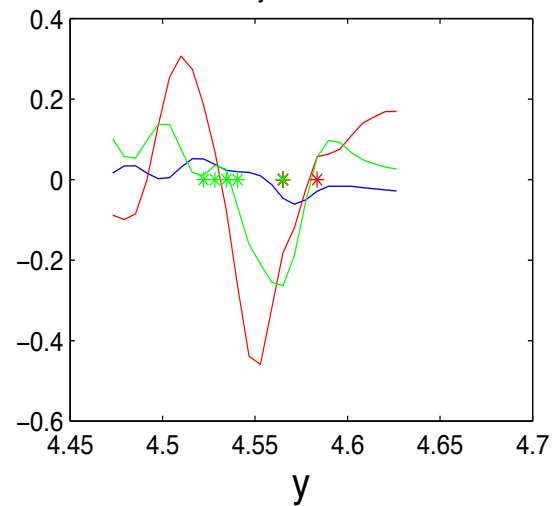

ns=32, cluster 21

(1.4419, 4.378, 3.43)

Magnetic Fields

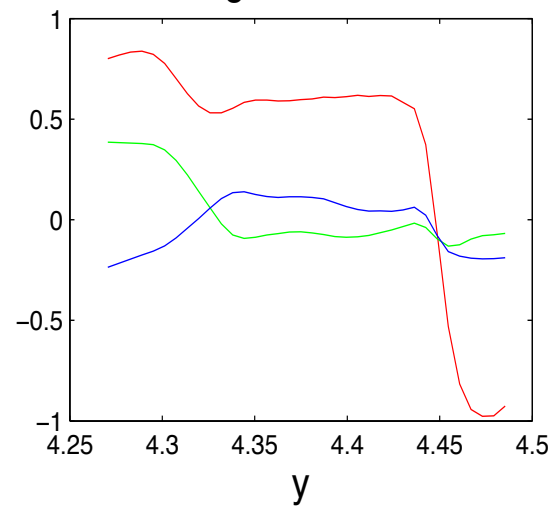

Velocity Fields

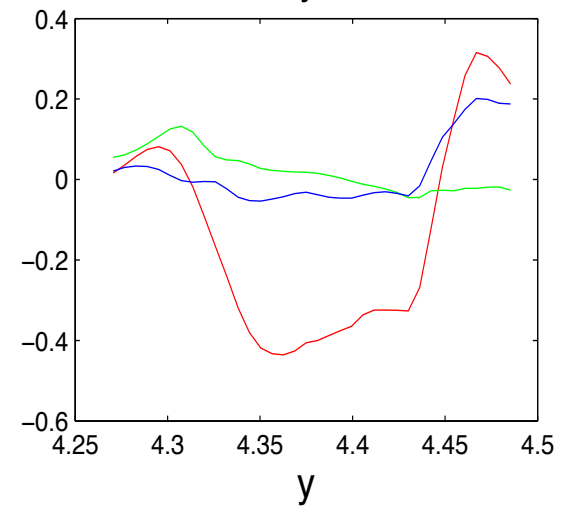

Magnetic Field Rotated

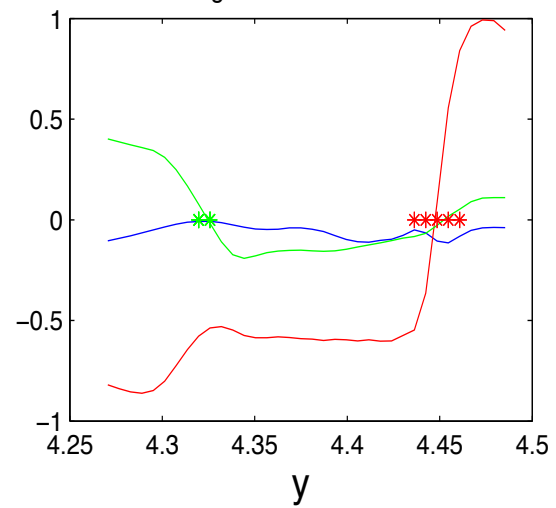

Velocity Field Rotated

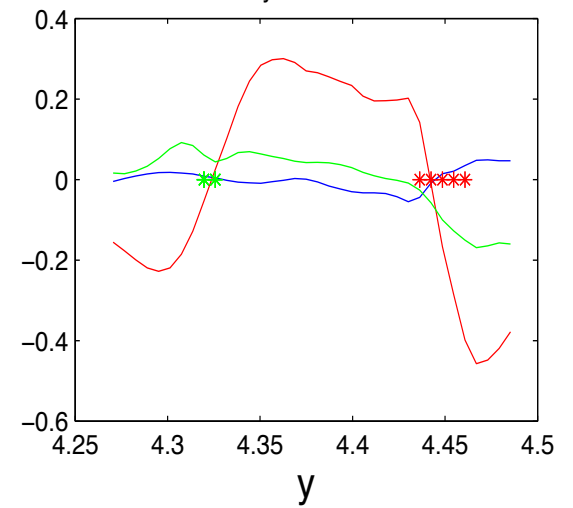

ns=32, cluster 22



(1.4419, 0.26691, 4.6204)

Magnetic Fields

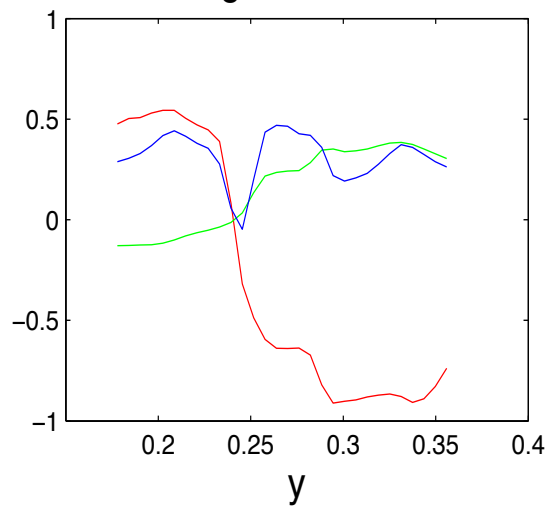

Velocity Fields

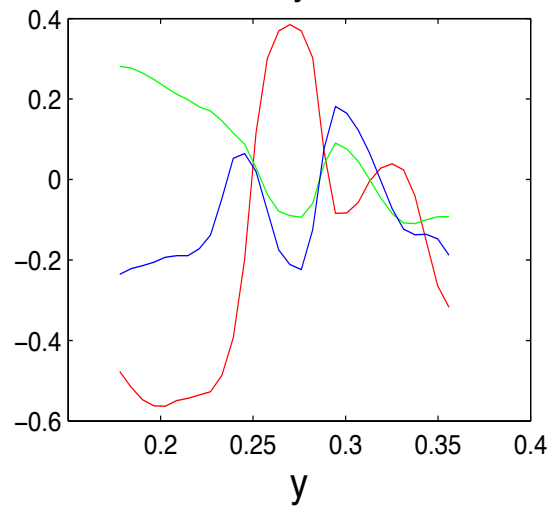

Magnetic Field Rotated

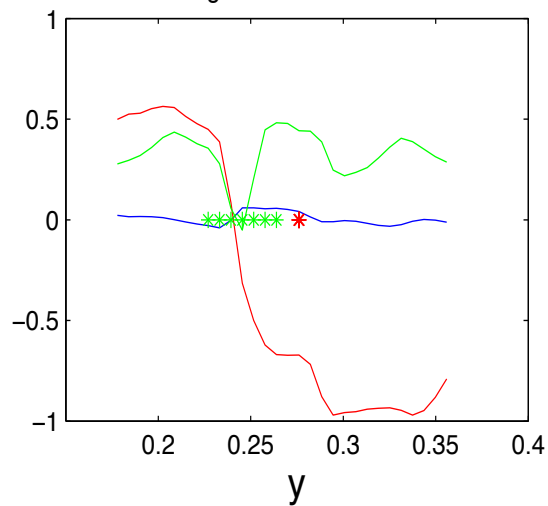

Velocity Field Rotated

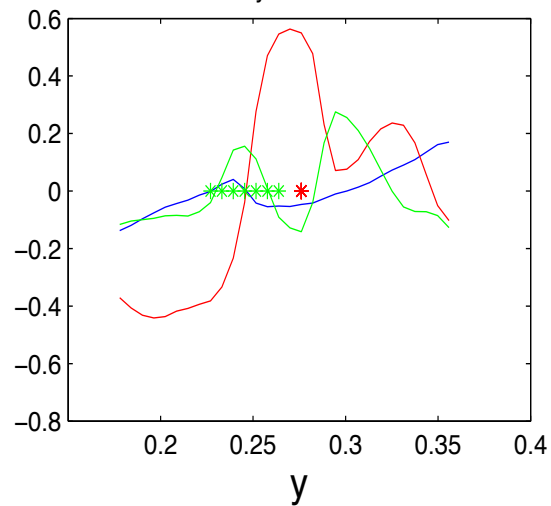

ns=32, cluster 23

(2.9637, 1.669, 4.6204)

Magnetic Fields

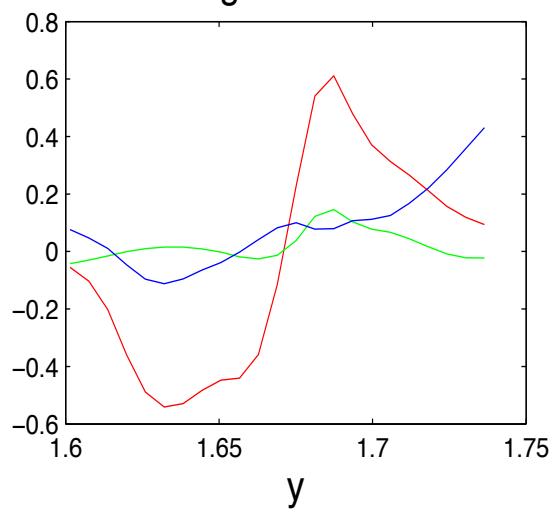

Velocity Fields

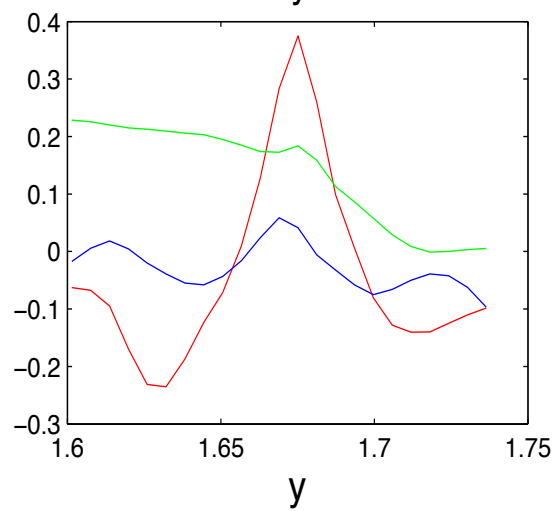

Magnetic Field Rotated

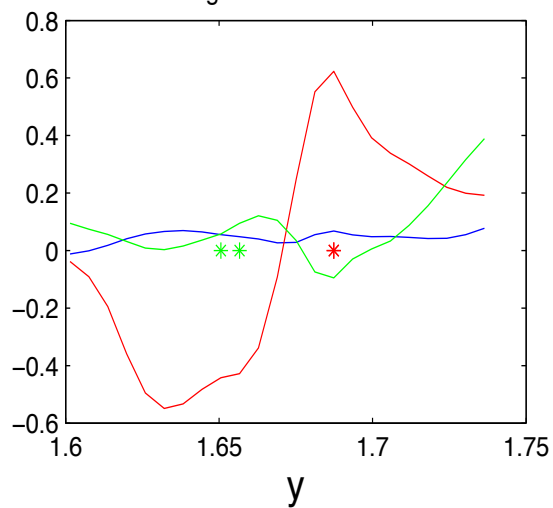

Velocity Field Rotated

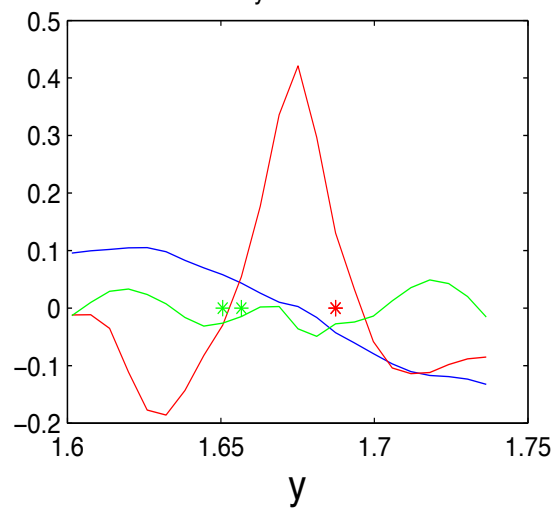

ns=32, cluster 24

(2.9637, 0.90812, 5.8414)

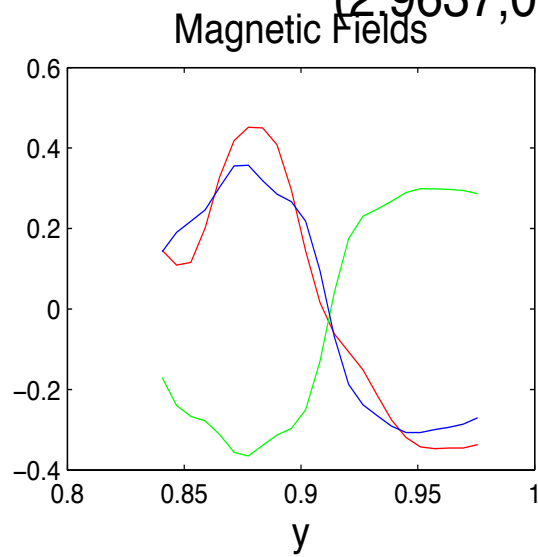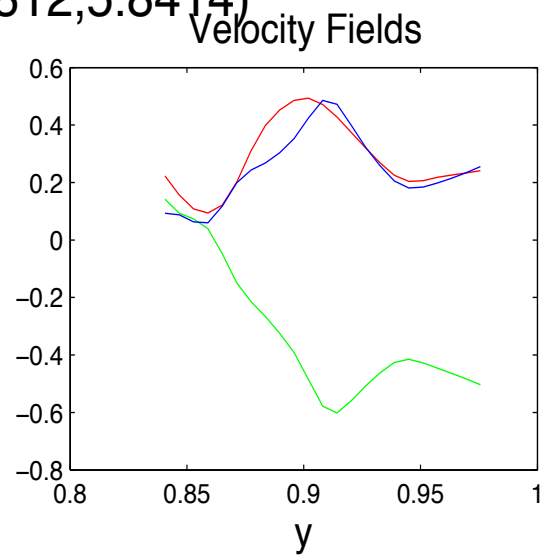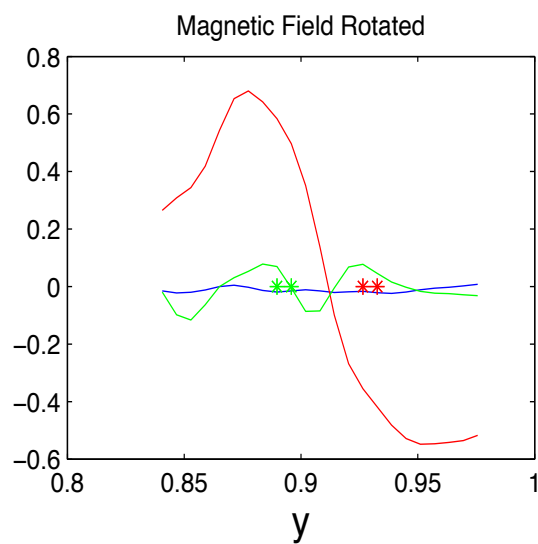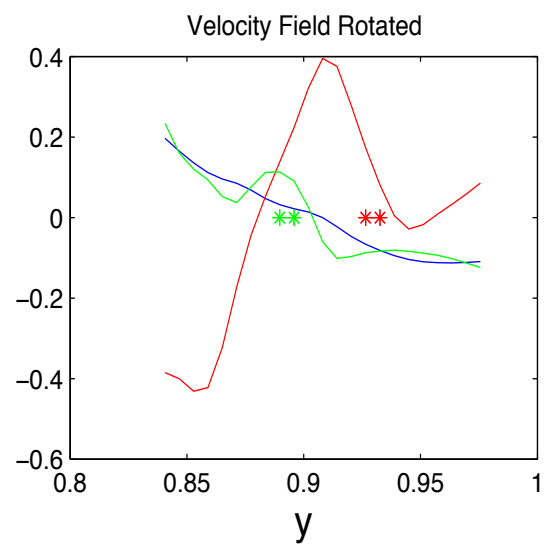

ns=32, cluster 25

(3.6263, 4.9486, 5.0744)

Magnetic Fields

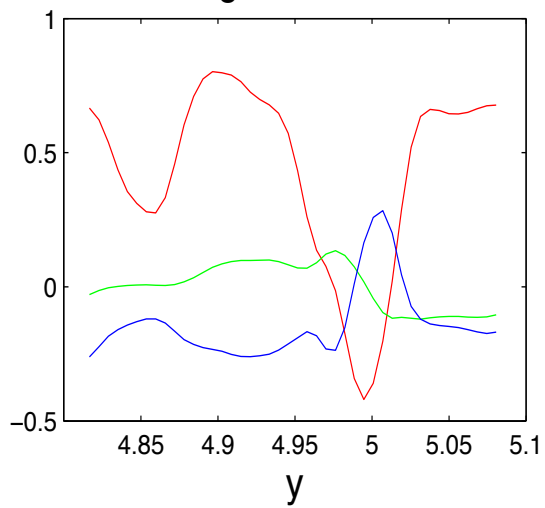

Velocity Fields

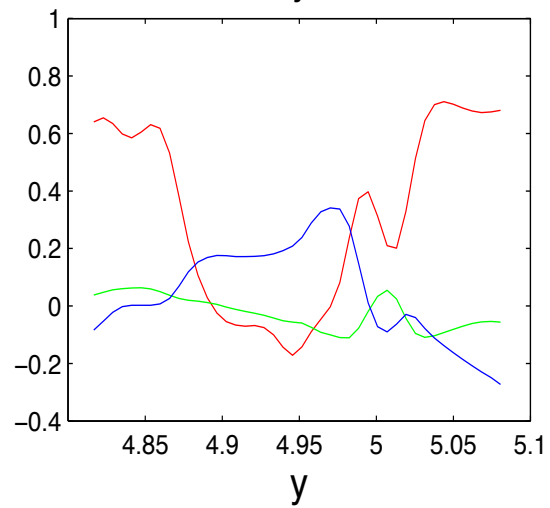

Magnetic Field Rotated

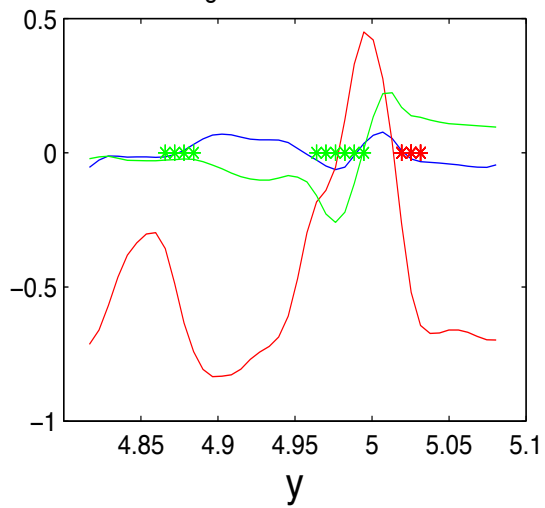

Velocity Field Rotated

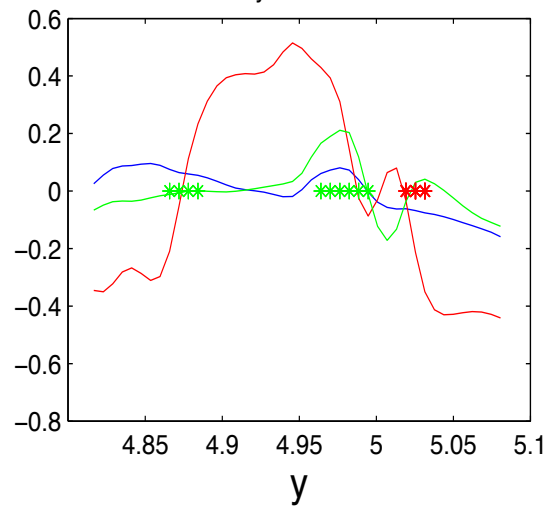

ns=32, cluster 26

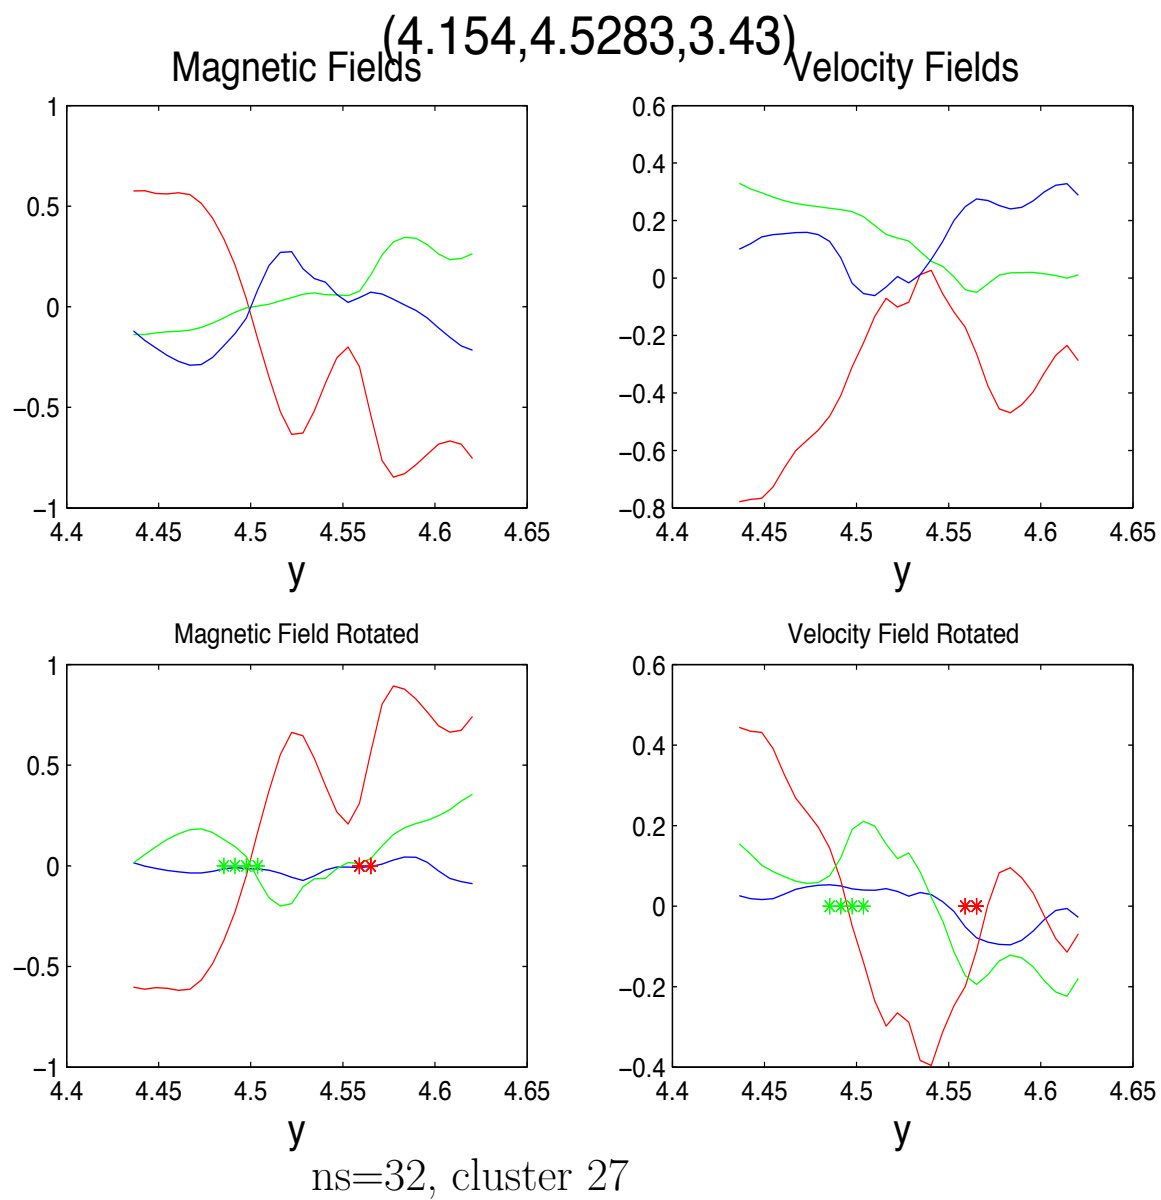

Supplement: Supplementary file 3 [file MHD_event_catalogue.pdf]
