# Supplementary material for: Inertial-Range Reconnection in Magnetohydrodynamic Turbulence and in the Solar Wind
Source: arXiv:1503.00509 ancillary file (2015-03-02)
Supplement: Supplementary file 4 [file Reconnection_Coarse_Movie-doc.pdf]

## Documentation for Reconnection Coarse Movie

Reconnection Coarse Movie illustrates the reconnection of coarse-grained magnetic field-lines. Specifically, it shows the process of “splitting” of a field-line of the coarse-grained magnetic field, whereby plasma elements initially lying on that single field-line, when evolved forward in time, come to reside on distinct “split” lines. In the example shown in the movie, the initial field-line at time  $t=0$  is an “incoming” line on the weak-field side of the reconnection zone, away from the strong flux-rope. The magnetic flux-rope is visualized by the half-maximum (0.3) isosurface of the magnitude of the coarse-grained magnetic field, in yellow. The “split” lines at later times have very different “topologies” and both outgoing, opposite plasma jets contain some of these lines.

As is well-known, magnetic field-line “motion” is a subjective and non-unique notion. Therefore, our procedure is instead to track plasma fluid elements and then trace the field-lines which instantaneously thread them, both of which operations are completely objective and uniquely defined. To track elements moving with the coarse-grained fluid velocity  $\bar{\mathbf{u}}$  (for filter length  $L$ , as in the Letter), we simply solve the ODE for the position  $\mathbf{x}(t)$  of the fluid element starting at  $\mathbf{x}_0$  at time  $t=0$ :

$$d\mathbf{x}/dt = \bar{\mathbf{u}}(\mathbf{x},t), \quad \mathbf{x}(0) = \mathbf{x}_0. \quad (*)$$

Then, to trace the field-line through the point  $\mathbf{x}(t)$  at time  $t$ , we solve the ODE for the position  $\xi(s; \mathbf{x}(t))$  at arclength  $s$  along the magnetic field-line starting at  $\mathbf{x}(t)$ :

$$d\xi/ds = \bar{\mathbf{b}}(\xi(s),t), \quad \xi(0) = \mathbf{x}(t) \quad (**)$$

where  $\bar{\mathbf{b}} = \bar{\mathbf{B}} / |\bar{\mathbf{B}}|$  is the versor field corresponding to the coarse-grained magnetic field  $\bar{\mathbf{B}}$  (also for filter length  $L$ ). We apply this procedure to a finite number  $n$  of plasma elements located at initial locations  $\mathbf{x}_k(0)$ ,  $k=1, \dots, n$  along an incoming line at time  $t=0$  and then trace the field-lines threading the elements located at  $\mathbf{x}_k(t)$ ,  $k=1, \dots, n$  for  $t>0$ .

For the movie we chose an incoming field-line of  $\bar{\mathbf{B}}$  reasonably close to the HFT at time  $t=0$ . Specifically, we found the line passing through point  $\mathbf{x}_0 = (2.7489, 1.3008, 5.6757)$  by solving (\*\*) for its location  $\xi_0(s)$  as a function of arc-length  $s$ . Other choices of the initial field-line gave similar results. We then “decorated” this initial line with  $n=11$  fluid elements evenly spaced by distance  $d$  along the line, at positions  $\mathbf{x}_k(0) = \xi_0((k-6)d)$  for  $k=1, \dots, 11$ . (Note thus that  $\mathbf{x}_6(0) = \mathbf{x}_0$  is the original point.) The first frame of the movie shows the initial field line and the 11 points along it as variously colored small cubes.

To obtain the subsequent frames of the movie, we integrated (\*) forward in time for each of the elements at initial positions  $\mathbf{x}_k(0)$ ,  $k=1, \dots, 11$  to find their positions at 8 times  $t_i = (0.32)(i-1)$ ,  $i=1, \dots, 8$ . For each location  $\mathbf{x}_k(t_i)$ , the equation (\*\*) was then integrated to find the corresponding field-line threading the plasma element at that point at time  $t_i$ . The  $i^{\text{th}}$  frame of the movie shows each of the 11 positions  $\mathbf{x}_k(t_i)$ ,  $k=1, \dots, 11$  represented by a small cube, with the same color for each  $k$ -value as at time  $t=0$ . Furthermore, the  $i^{\text{th}}$  frame of the movie shows through each of these 11 positions  $\mathbf{x}_k(t_i)$ ,  $k=1, \dots, 11$  the unique field-line of the coarse-grained magnetic field which instantaneously threads it, with color of line  $\#k$  identical that of the small cube  $\#k$  through which it passes.

## Documentation for Reconnection Coarse Movie

As can be seen in the movie, the 11 plasma elements which initially reside on the same line at time  $t=0$  are located on distinct lines at later times, i.e. the 11 plasma elements do not remain magnetically connected. This phenomenon appears as a “splitting” of the initial field-line into many field-lines. As time advances, the 11 field-lines threading the plasma elements become more and more separated in space and distinct in structure. This can occur because standard flux-freezing is violated in turbulent flows, even at arbitrarily high electrical conductivity. In fact, we observe this phenomenon to occur everywhere in the flow and not just in the vicinity of standard “reconnection events”, such as that illustrated in the movie.

In the vicinity of such a standard “reconnection event”, however, the “split” field-lines are further characterized by distinct “topologies”. This can be clearly observed in the 4<sup>th</sup> frame of the movie. In that frame, the dark **blue** field-line in the outflow on the far left (line #1) is now V-shaped and pointing into the screen, whereas the dark **red** field-line in the outflow on the far right (line #11) is V-shaped but pointing out of the screen. The transformation of these two field-lines from being approximately straight to V-shaped occurs by a characteristic process of “flipping” of one end of the line, with the tip of the line flipping for the **blue** line #1 on the left and the tail flipping for the **red** line #11 on the right. These two V-shaped lines in the 4<sup>th</sup> frame are now located within different “sectors” bounded by the sheets of the QSL and have very distinct magnetic connectivities. *This is the type of “topology change” in time which is usually viewed as the most characteristic feature of magnetic reconnection.*

As the movie proceeds, the plasma elements located in the outflow jets and the V-shaped lines “carried” by those elements move outward. New lines then undergo the same reconnection process by “flipping” their tips on the left and their tails on the right. For example, in the 7<sup>th</sup> frame, the **grey** line #6 on the left has flipped its tip and the brighter **red** line #10 on the right has flipped its tail. It is noteworthy that the process does not occur sequentially from the outer lines to the inner lines, since the **grey** line #6 “flips” prior in time to the lines #2-5 further to the left. The process is also not monotonic, since the **orange** line #9 on the right flips its tip (not its tail!) in the 5<sup>th</sup> frame but the tip then flips back in the final 8<sup>th</sup> frame of the movie, presumably prior to the tail flipping next as the plasma element exits with the outflow on the right.
