# Supplementary material for: Inertial-Range Reconnection in Magnetohydrodynamic Turbulence and in the Solar Wind
Source: arXiv:1503.00509 ancillary file (2015-03-02)
Supplement: Supplementary file 5 [file Reconnection_Fine_Movie-doc.pdf]

## Documentation for Reconnection Fine Movie

Reconnection Fine Movie illustrates the reconnection of fine-grained magnetic field-lines and the breakdown of standard flux-freezing in the MHD turbulence event analyzed in the Letter. Specifically, it shows the process of “merging” of fine-grained field-lines, whereby plasma elements initially lying on distinct field-lines, when evolved forward in time, come to reside on a single “merged” line. To identify a suitable outgoing field-line as the target for “merger”, an incoming line was chosen just entering the reconnection zone from the side of the strong magnetic flux-rope. This incoming line is shown as the solid **black** line in Figs. S1 and S2 on the following page, from two views. The half-max current isosurfaces are included in **green**, for context. This initial line was decorated with 11 fluid elements, represented by the variously **colored** blobs •, at regularly-spaced positions  $\mathbf{x}_n(0)$ ,  $n=1, \dots, 11$  along the line. The positions of these fluid elements were then evolved in time according to the ODE

$$d\mathbf{x}/dt = \mathbf{u}(\mathbf{x}(t), t) \quad (*)$$

to find the positions  $\mathbf{x}_n(t)$ ,  $n=1, \dots, 11$  at later times  $t>0$ . The positions at the time  $t=2$  are also shown by 11 **colored** blobs • in Figs. S1-S2, together with the field-lines in the corresponding color that thread each element at  $t=2$ . Both of these figures illustrate the process of “splitting” of initial magnetic field-lines: because field-lines are no longer “frozen to” fluid elements in a high-conductivity turbulent flow, the fluid elements initially lying on a single line at time  $t=0$  end up on distinct lines at times  $t>0$ . This is exactly the same “splitting” process illustrated in Reconnection Coarse Movie, but now for lines of the fine-grained magnetic field rather than of the coarse-grained magnetic field. The outgoing lines  $n=1-3$  from the bottom, colored **red**, **green**, **blue**, are in the downward reconnection jet and the remaining lines  $n=4-11$  are in the upward reconnection jet.

To illustrate the reverse process of “merging”, we chose as “target” one of the field-lines in the upward reconnection jet at time  $t=2$ , here, the **red** line at  $t=2$  corresponding to the middle red blob • on the initial **black** line (line  $n=6$ ). The movie illustrates how two plasma elements initially on distinct field-lines, come to reside on the “merged” **red** line at the final time  $t=2$ . To prepare this movie, we simply identified two fluid elements on the **red** line at time  $t=2$ , which have positions  $\mathbf{x}_m(2)$ ,  $m=1, 2$ . These two elements are represented by the two colored blobs • and • on the **red** line in the final frame of the movie. To find the earlier positions of these elements, we solved (\*) backward in time with final conditions  $\mathbf{x}_m(2)$ ,  $m=1, 2$  to obtain  $\mathbf{x}_m(t)$ ,  $m=1, 2$  for  $t<2$ . We wish also in the movie to show the ensemble of positions  $\mathbf{x}_m^*(t)$ ,  $m=1, 2$  satisfying

$$d\mathbf{x}^*/dt = \mathbf{u}(\mathbf{x}^*(t), t) + \sqrt{2\lambda} \boldsymbol{\eta}^*(t) \quad (**)$$

for a Gaussian white-noise process  $\boldsymbol{\eta}^*(t)$ , which arrive to the points  $\mathbf{x}_m(2)$ ,  $m=1, 2$  at time  $t=2$ . The Stochastic Flux-Freezing Theorem for resistive MHD (see ref.[18] in the Letter) states that these stochastic positions represent the points of origin at time  $t$  of the magnetic field  $\mathbf{B}(\mathbf{x}_f, t_f)$  at final position  $\mathbf{x}_f=\mathbf{x}_m(2)$ ,  $m=1, 2$  and final time  $t_f=2$ . We solve (\*\*) for 1024 independent realizations of  $\boldsymbol{\eta}^*(t)$  for both  $m=1, 2$  and represent the ensembles at each time  $t<2$  by clouds of 1024 colored dots :: and ::.

# Documentation for Reconnection Fine Movie

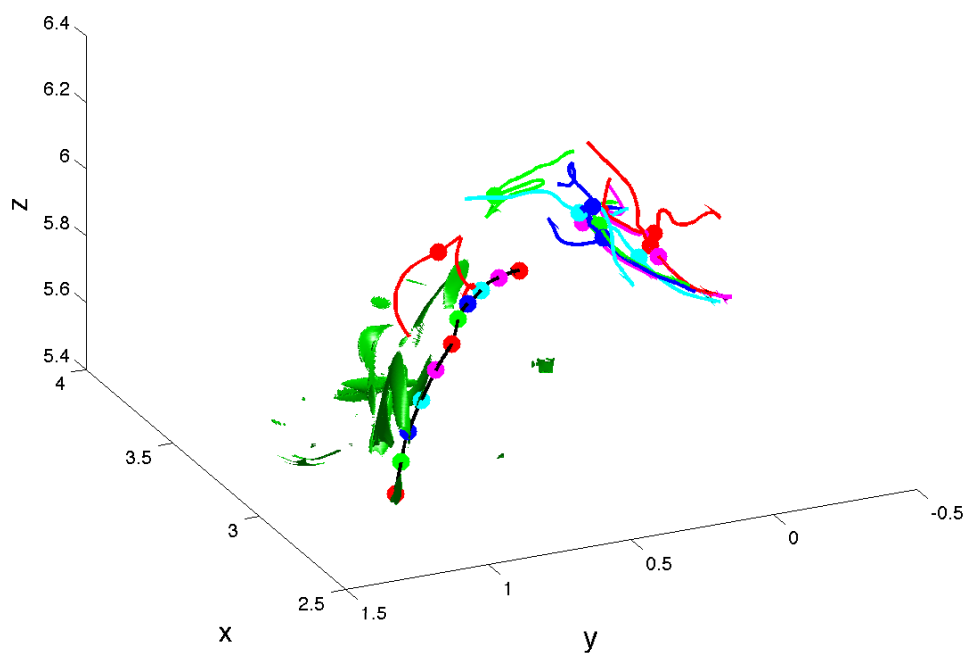

Fig. S1: Initial field-line and final “split” field-lines, viewed from the side of the flux rope.

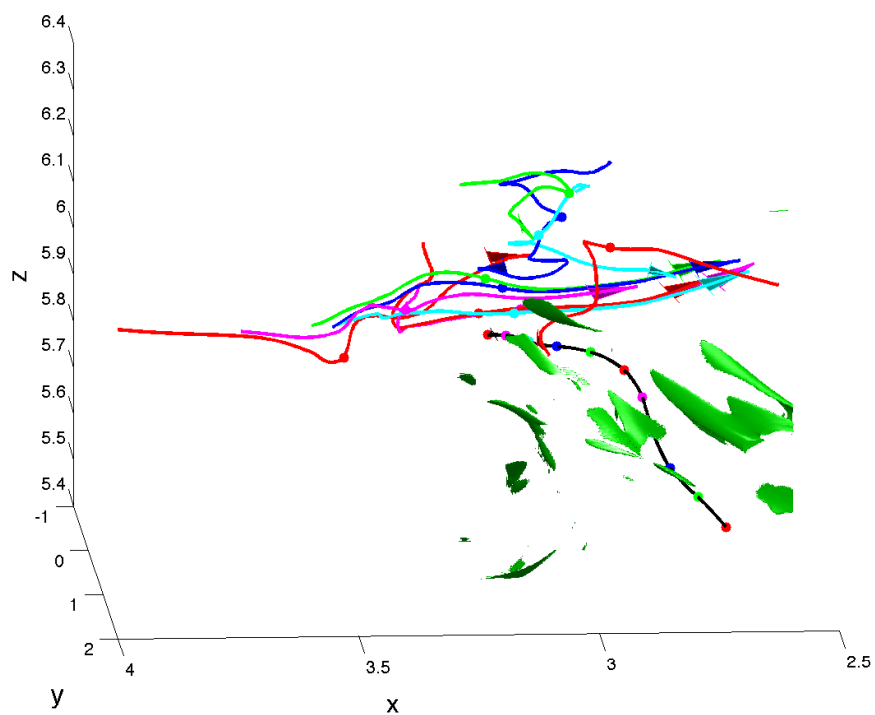

Fig. S2: Initial line and final lines, viewed from the side opposite to the flux rope.

## Documentation for Reconnection Fine Movie

Reconnection Fine Movie runs forward over time interval  $0 < t < 2$ , showing in each frame the positions  $\mathbf{x}_m(t)$ ,  $m=1,2$  as colored blobs  $\bullet$  and  $\bullet$ , the unique field-lines passing through these two elements  $\mathbf{x}_m(t)$ ,  $m=1,2$  as colored arrows  $\rightarrow$  and  $\rightarrow$ , and the cloud of 1024 stochastic positions  $\mathbf{x}_m^*(t)$ ,  $m=1,2$  as colored dots  $::$  and  $::$ . In the final frame at time  $t=2$  the “target” red field-line is also shown as an arrow  $\rightarrow$ . To give some additional perspective on the evolution, each frame also shows in yellow the isosurface  $|\mathbf{B}|=1.1072$ , the half-maximum field-strength value at  $t=0$ . The movie clearly shows the process of “merging” of the blue and cyan field-lines, which thread the fluid elements at  $\mathbf{x}_m(t)$ ,  $m=1,2$  for each  $0 < t < 2$ , into the single red field-line at time  $t=2$ .

Several features of the evolution are worth comment:

- 1) The two initial lines  $\rightarrow$  and  $\rightarrow$  through the points  $\mathbf{x}_m(0)$ ,  $m=1,2$  shown at time  $t=0$  are both on the same side of the reconnection zone, near the magnetic flux-rope. Thus, the two field-lines shown at time  $t=0$  are oriented in approximately the same direction.
- 2) As time proceeds, the plasma element at  $\mathbf{x}_m(t)$ ,  $m=1$ , marked with the blob  $\bullet$ , drifts to the opposite side of the reconnection zone. Correspondingly, the field-line indicated by  $\rightarrow$  slowly acquires an orientation opposite to the orientation of the line  $\rightarrow$  through the second plasma element  $\mathbf{x}_m(t)$ ,  $m=2$ .
- 3) Near the final time, the blue field-line  $\rightarrow$  undergoes a characteristic rapid “flipping”, first at the tip and then at the tail, in order to “merge” with the line  $\rightarrow$  and yield the selected “target” line  $\rightarrow$  at  $t=2$ .
- 4) This process of “splitting” and “merging” of field-lines tagged by particular fluid elements is typical of MHD turbulence and occurs throughout the simulation domain, not merely in the vicinity of extreme “reconnection” events such as shown here. However, near these extreme “reconnection” events “splitting” and “merger” are more commonly accompanied by “flipping” and “topology change” of the field-lines.
- 5) The ensembles of stochastic positions  $\mathbf{x}_m^*(t)$ ,  $m=1,2$  represented by colored dots  $::$  and  $::$  gradually converge to the final blobs  $\bullet$  and  $\bullet$  at  $t=2$ , the time-reverse of the Richardson dispersion studied in Fig.5b of the Letter. Note that the initial ensembles at  $t=0$  are very elongated along the L-direction and considerably less dispersed along the orthogonal M- and N-directions. The latter process, however, is responsible for the “turbulent mixing” of magnetic fields across the reconnection zone.

REMARK: The red dots  $::$  in Fig.5a of the Letter are the stochastic points at time  $t=0$  which arrive to the extreme tail of the red field-line  $\rightarrow$  at time  $t=2$  in this movie.
