# Supplementary material for: Inertial-Range Reconnection in Magnetohydrodynamic Turbulence and in the Solar Wind
Source: arXiv:1503.00509 ancillary file (2015-03-02)
Supplement: Supplementary file 6 [file Wind_event_catalogue.pdf]

## Wind Event Catalogue Documentation

In the Wind Event Catalogue we analyze two periods containing streams of high-speed solar wind. We used data from both these streams to have a longer range of high-speed solar wind in which to search for candidate reconnection events. In what follows, we define “high-speed” solar wind as a condition on the largest (in magnitude) component of the velocity:  $\max_k |v_k| > 600$  km/sec. In each data set, we report the equivalent number of “days” of high-speed wind by counting the duration of all occurrences of the high-speed condition being met, even if the occurrences are brief and not part of a larger stream of high-speed data. The first dataset is a 7 day period from 2008 January 14 04:40:00 to January 21 03:20:00 which contains approximately 6.7 days of high-speed wind. The second dataset is an approximately 1.5 year period from 2005/10/01 00:00:00 – 2007/05/01 00:00:00, which contains the equivalent of about 62.4 days of high-speed wind. The years 2005-2008, the range of the data streams, are near minimum in the solar activity cycle and the *Wind* spacecraft orbit is at low to moderate solar latitudes.

As reported in the main body of the Letter, we made a careful comparison of the probability density functions (PDFs) of magnetic-field increment magnitudes from the JHU MHD database and from the *Wind* spacecraft data for 2008 January 14 04:40:00 to January 21 03:20:00. We found that the PDF's of  $|\delta \mathbf{B}|$  at space-separations  $r=n \, dx$  in the MHD database compare quite well to the same PDFs for the *Wind* data at time-separations  $\tau = n$  (0.18 sec) for the same choice of  $n$ , with values of  $n$  corresponding to the inertial-range of both flows. Thus, the grid spacing  $dx$  in the database is in good statistical relation to 0.3 minutes (18 seconds) in the solar wind time series. This same correspondence of statistics also works well for the fast regions of the other dataset spanning 2005/10/01 00:00:00 – 2007/05/01 00:00:00. With this correspondence, the turbulent outer time-scale  $T$  of the solar wind stream of the 2008 dataset is estimated to be approximately 17.1 minutes. This determination of  $T$  also agrees well with the upper limit of the time range where the 2/3rd power-law in the structure-function of magnetic-field increments is observed in the *Wind* data.

We now detail the criterion we use to identify candidate reconnection events in the high-speed wind, which is essentially the same as in the MHD database. As there, we define magnetic and velocity increments at instant  $p$  for a time separation  $r$  by the symmetric differences:

$$\delta \mathbf{u}(r; p) = \mathbf{u}(p - r/2) - \mathbf{u}(p + r/2), \quad \delta \mathbf{B}(r; p) = \mathbf{B}(p - r/2) - \mathbf{B}(p + r/2)$$

We also define the magnetic field  $\mathbf{b}$  in Alfvén velocity units by  $\mathbf{b} = \mathbf{B}/\sqrt{4\pi\langle\rho\rangle}$ , where  $\langle\rho\rangle$  is the average plasma mass density. Ignoring for simplicity the small component of alpha particles and other more massive ions in the solar wind, we take  $\langle\rho\rangle = m_p \langle n \rangle$  where  $m_p$  is the proton mass and  $\langle n \rangle$  is the mean ion number density. To formulate our criterion, we first fix a number  $r$  called the duration of increment, a number  $R$  called the reversion interval and two pure numbers  $T_B$  and  $T_U$ , the magnetic and velocity thresholds. We then identify an interval

## Wind Event Catalogue Documentation

$[p - r/2, p + r/2 + R^*]$ . in the *Wind* time-series as a possible reconnection event if the following criteria are all satisfied:

- (i) There is a point  $p$  such that
  - a.  $[p - r/2, p + r/2]$  is a high-speed interval
  - b.  $|\delta \mathbf{u}(r; p)| \geq T_U |\delta \mathbf{b}(r)|_{\text{rms}}$
  - c.  $|\delta \mathbf{B}(r; p)| \geq T_B |\delta \mathbf{B}(r)|_{\text{rms}}$
- (ii) There is an  $R^* \leq R$  such that
  - a.  $[p - r/2, p + r/2 + R^*]$  is a high-speed interval
  - b.  $|\delta \mathbf{u}(r; p + R^*)| \geq T_U |\delta \mathbf{b}(r)|_{\text{rms}}$
  - c.  $|\delta \mathbf{B}(r; p + R^*)| \geq T_B |\delta \mathbf{B}(r)|_{\text{rms}}$
- (iii)  $\delta \mathbf{B}(r; p) \cdot \delta \mathbf{B}(r; p + R^*) > 0$
- (iv)  $\delta \mathbf{u}(r; p) \cdot \delta \mathbf{u}(r; p + R^*) < 0$
- (v)  $(\delta \mathbf{u}(r; p) \cdot \delta \mathbf{B}(r; p)) \times (\delta \mathbf{u}(r; p + R^*) \cdot \delta \mathbf{B}(r; p + R^*)) < 0$

We applied the above algorithm to the *Wind* data using  $r = 1.8 \text{ min} \approx L/10$ ,  $R = 8.55 \text{ min} \approx L/2$ ,  $T_B = T_U = 1.5$ . After sifting through the data with this algorithm, we selected by eye from among the output events which appeared to be reasonable candidates for reconnection, which we present in the catalogue.

On the first page of this document, we record the values of physically important quantities for each of the datasets used (calculated from only high speed wind), including mean  $B$ , rms  $b$ , rms  $u$ , max  $|\delta \mathbf{b}|$ , max  $|\delta \mathbf{u}|$ , rms  $|\delta \mathbf{b}|$ , rms  $|\delta \mathbf{u}|$ , ion gyroradius, plasma beta, mean Alfvén speed  $V_A$ , equivalent number of days of high speed wind. Note here that we always use the notation  $\mathbf{u} = \mathbf{v} - \langle \mathbf{v} \rangle$  to denote the fluctuating part of the ion plasma velocity  $\mathbf{v}$ . The rms values for the increment magnitudes  $|\delta \mathbf{b}(r)|$  and  $|\delta \mathbf{u}(r)|$  are calculated for the fixed separation  $r = 1.8$  minutes used in selecting the reconnection events in the algorithm. The mean Alfvén speed  $V_A$  is calculated using the mean magnetic field and density over the entire high-speed streams.

From the second page on, each page of the catalogue presents a candidate reconnection event picked out by our criteria. The first two subplots show the components of the magnetic and velocity fields, rotated to the minimum variance frame (MVF) of the magnetic field over the duration of the event. MVF components are identified as L/maximum variance (red), M/median variance (green) and N/minimum variance (blue). We also identify the points which triggered our criteria. Keeping the notation above, the points “ $p$ ” are marked with green stars ★ and points “ $p + R^*$ ” are marked with red stars ★. The remaining three plot on each page show the proton number density, the proton temperature, and the magnetic field strength.

Event 1 is the event mentioned in the Letter. This and a number of others, such as Events 3, 9 and 11, look similar to the event from the MHD database analyzed in detail in the Letter. Others resemble more the types of events Gosling often

## Wind Event Catalogue Documentation

selects, in that the magnetic fields exhibit rotational “discontinuities” at the edges of the event and plateaus with intermediate field orientations inside. Some such “Gosling-like” events are Events 2, 4, and 7 in the catalogue. However, the rotations at the edges are often not very well described as “discontinuities”, e.g. the rotation at the beginning of Event 4 occurs over a 2 min interval. (The rotation of magnetic fields on intervals much larger than the ion skin depth is also true at the edges of many events identified by Gosling as reconnection.) The other events in the catalogue are more complex, although each could be plausibly argued to be an instance of magnetic reconnection. We note that there is often a noticeable increase in ion density and temperature at the location of the putative reconnection exhaust, a feature also often observed by Gosling.

It is worth making a final remark about the frequency of the events located by our “large-scale Gosling criterion.” We identify with this criterion approximately 1.3 such large-scale events per week. In Gosling’s own search of the same high-speed solar-wind data as our second dataset, i.e. that taken by the *Wind* spacecraft from 2005 October through 2007 June, he reported a frequency of reconnection events of about 0.6 per day. These different frequencies are not inconsistent, since Gosling’s selection criterion mainly identifies smaller-scale events (see Fig.7 in Gosling, 2007). It is to be expected that there will be many fewer intense large-scale reconnection events than small-scales ones in a turbulent inertial-range. On the other hand, we note that there appear to be distinctly fewer large-scale reconnection events identified by our criterion in the high-speed wind, relatively speaking, than in the MHD database. Our catalogue of the *Wind* observations contains 13 events from 5819 integral times  $T$  of data, whereas our catalogue for the MHD simulation contains 27 events from 3447 integral lengths  $L$  of data. This discrepancy may be in part explained by the fact that the catalogue for the MHD database contains all events identified by the criterion, some of which are not obviously reconnection at all (e.g. clusters 5,16), whereas the catalogue for the *Wind* observations is a selection of the most promising events from many more which satisfied the criterion. On the other hand, the catalogue of the events from the *Wind* observations used a threshold value  $T_U = T_B = 1.5$ , whereas the catalogue of events for the MHD simulation set a higher threshold  $T_U = T_B = 2.0$ . This lower threshold for the *Wind* data should have permitted a greater frequency of events there, but it did not. If there is any statistical significance to the apparent smaller frequency of events in the *Wind* data, it may be due to the strong Alfvénicity/imbalance of the high-speed solar wind stream which reduces the strength of the nonlinear interactions.

# Catalogue of Events from *Wind* Spacecraft

## Selection Criteria:

Duration of increment = 1.8 minutes

Reversion interval = 8.55 minutes

Threshold for  $\delta B$  and  $\delta u = 1.5$

Data from: 2008/01/14 04:40:00 – 2008/01/21 03:20:00

$\langle |\mathbf{B}| \rangle = 4.25$  nT  
rms  $\mathbf{b} = 61.80$  km/sec  
 $\langle |\mathbf{v}| \rangle = 645.79$  km/sec  
rms  $\mathbf{u} = 54.11$  km/sec  
max  $|\delta \mathbf{b}| = 165.76$  km/sec  
max  $|\delta \mathbf{u}| = 136.16$  km/sec  
 $|\delta \mathbf{b}|$  rms = 28.59 km/sec  
 $|\delta \mathbf{u}|$  rms = 18.61 km/sec  
ion gyroradius = 152.04 km  
plasma beta = 1.05  
mean density =  $2.35 \text{ cm}^{-3}$   
mean  $V_A = 60.30$  km/sec  
high speed wind = 6.7 days

Data from: 2005/10/01 00:00:00 – 2007/05/01 00:00:00

$\langle |\mathbf{B}| \rangle = 3.83$  nT  
rms  $\mathbf{b} = 60.60$  km/sec  
 $\langle |\mathbf{v}| \rangle = 655.53$  km/sec  
rms  $\mathbf{u} = 109.87$  km/sec  
max  $|\delta \mathbf{b}| = 389.62$  km/sec  
max  $|\delta \mathbf{u}| = 684.98$  km/sec  
 $|\delta \mathbf{b}|$  rms = 29.01 km/sec  
 $|\delta \mathbf{u}|$  rms = 24.02 km/sec  
ion gyroradius = 188.90 km  
plasma beta = 1.48  
mean density =  $2.15 \text{ cm}^{-3}$   
mean  $V_A = 56.91$  km/sec  
high speed wind = 62.4 days

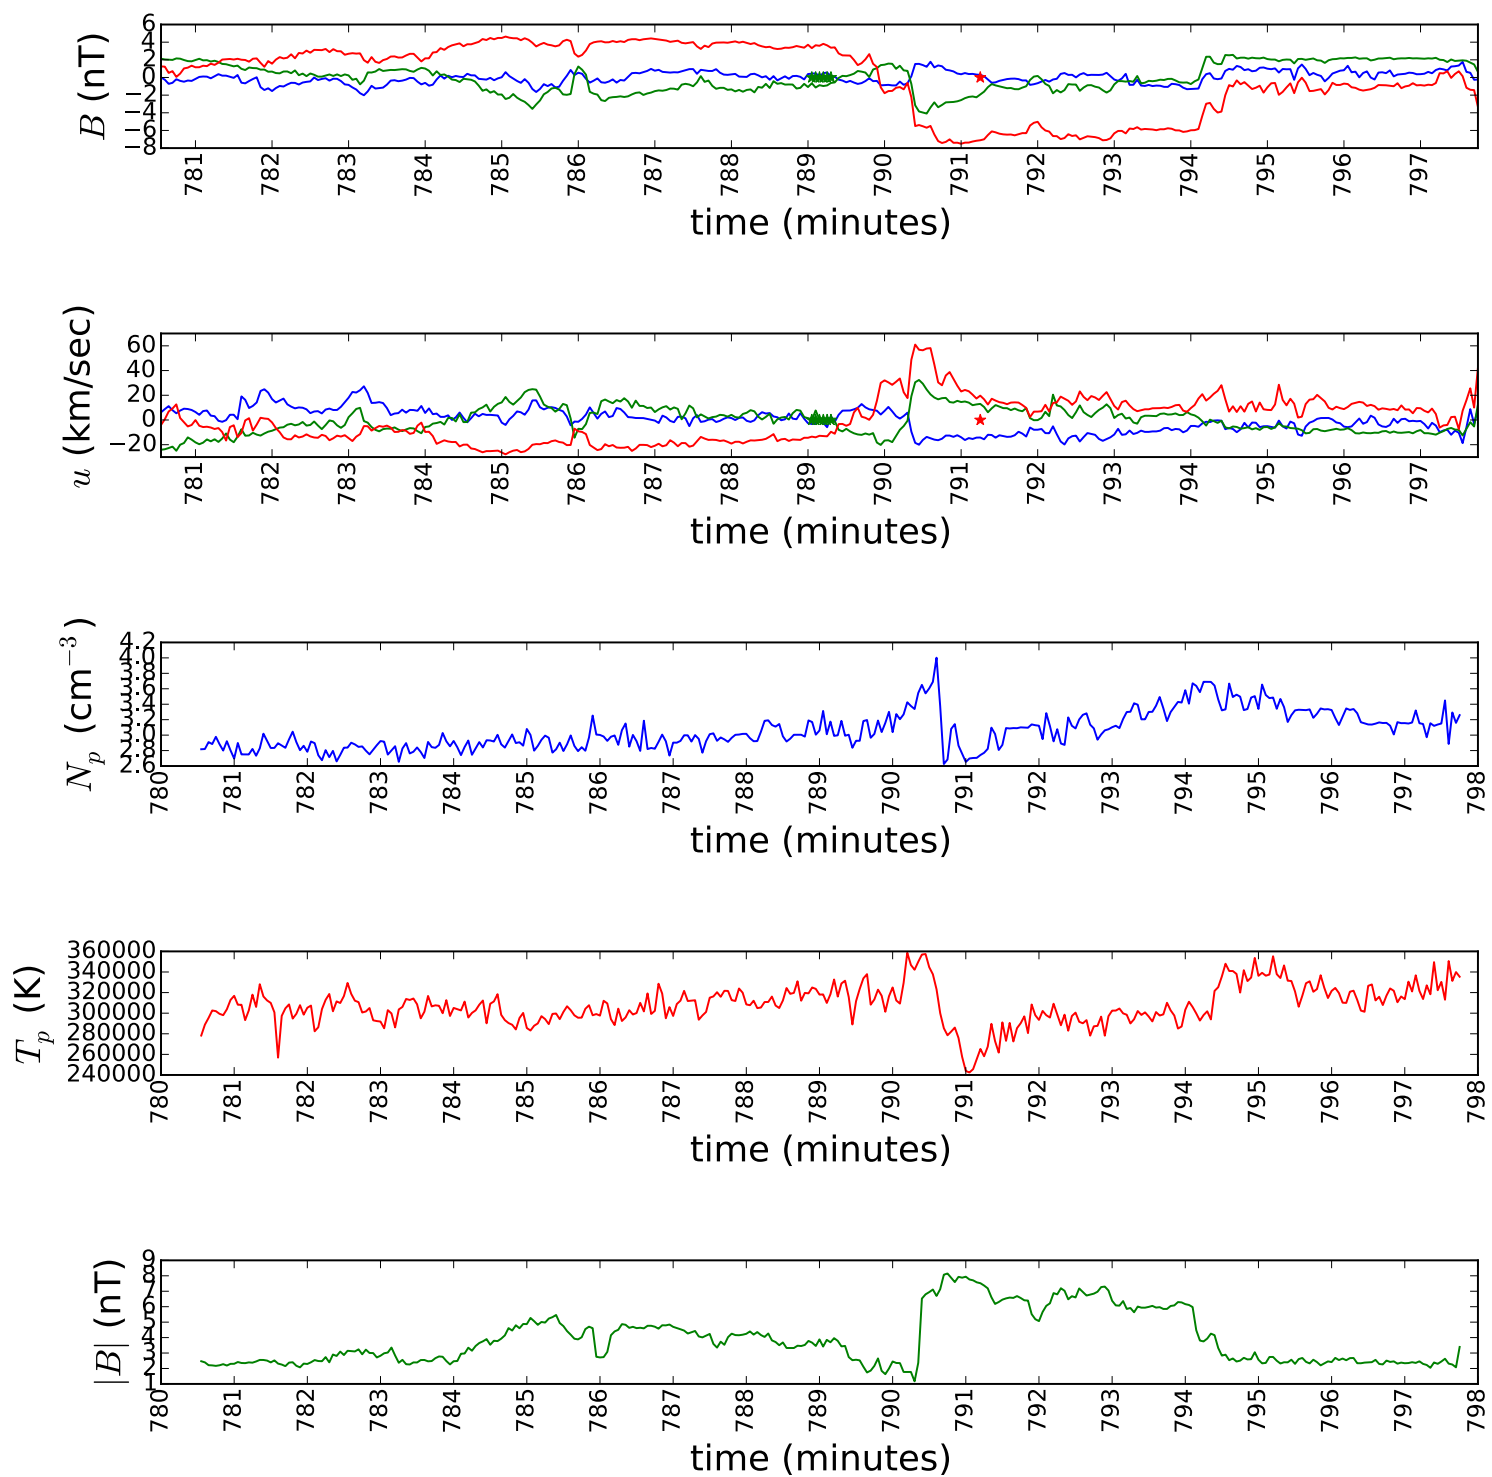

**Event 1:** January 14, 2008, 13:50

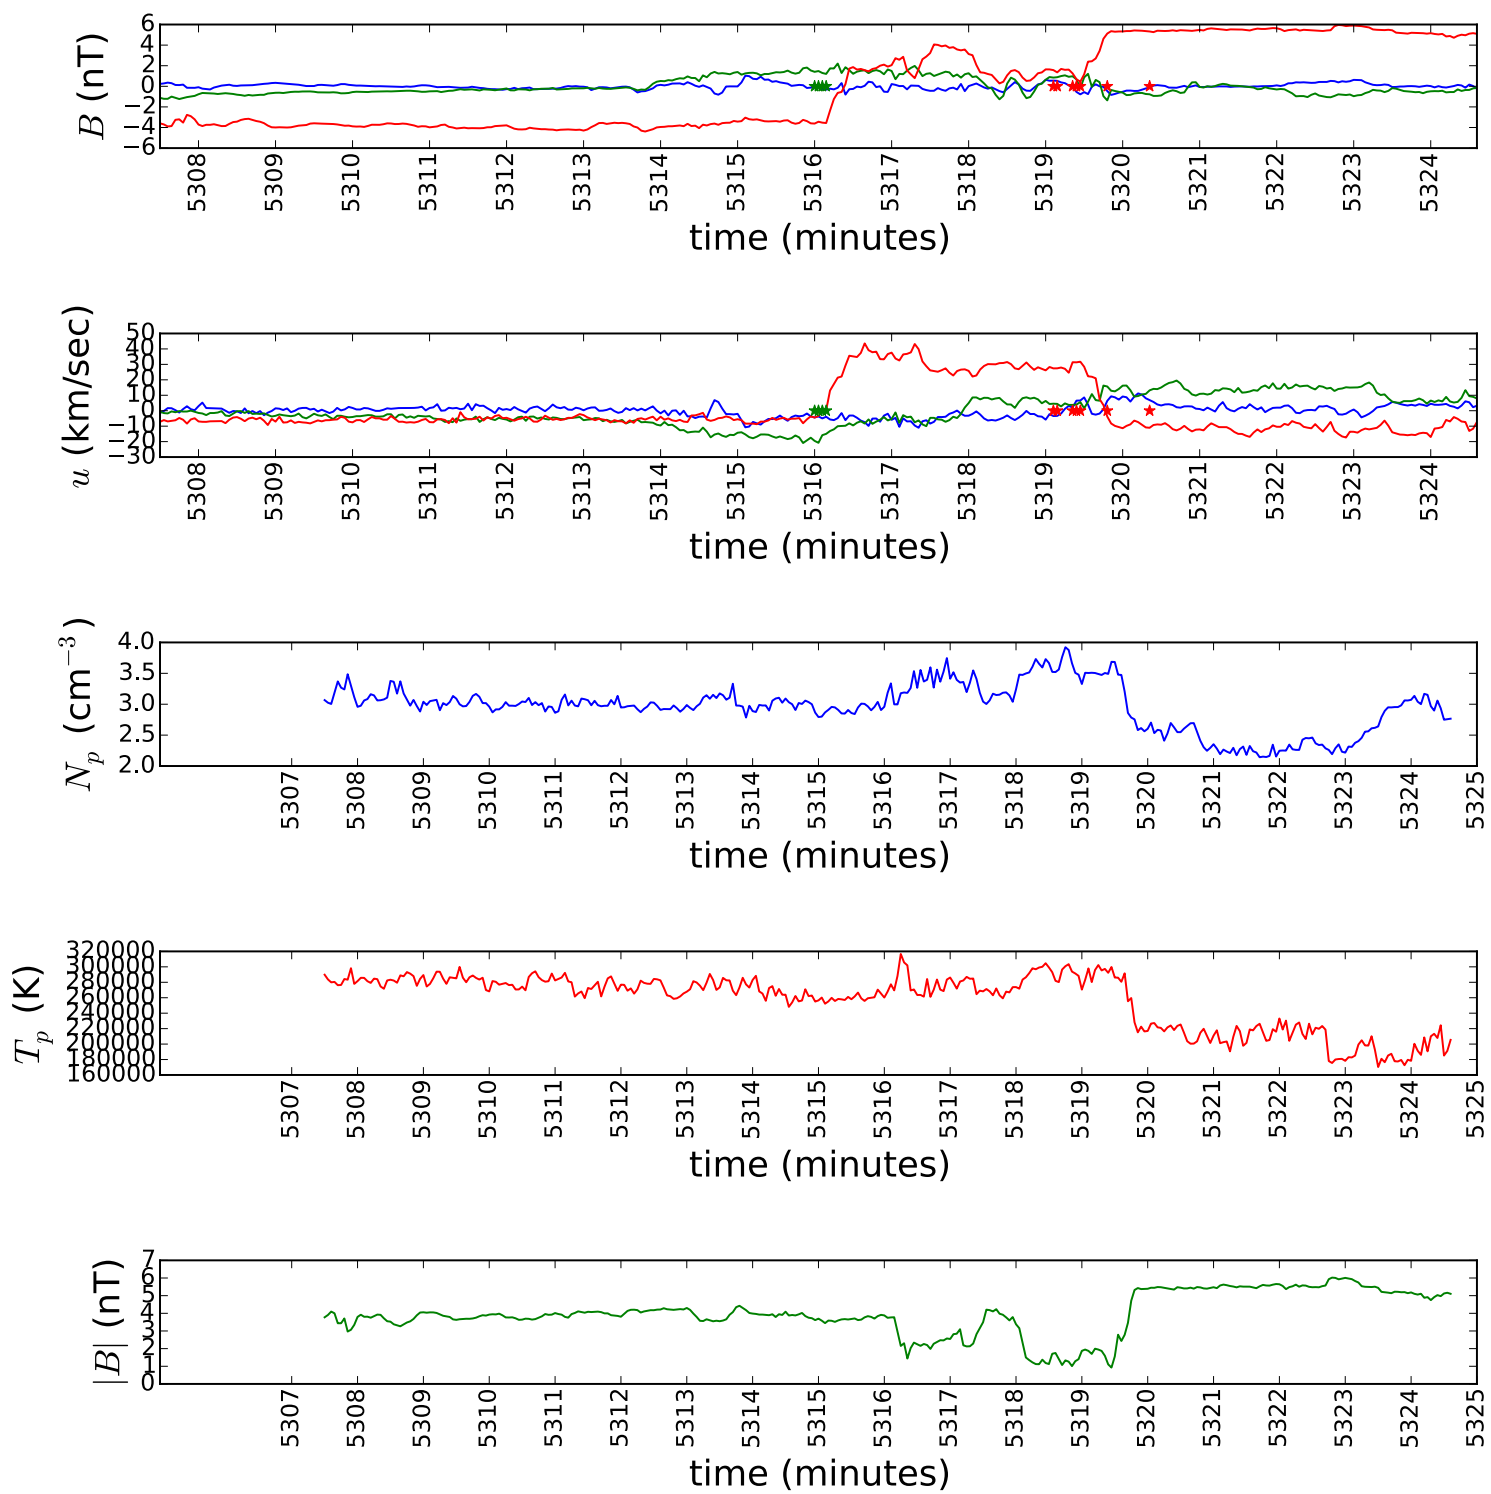

**Event 2:** January 14, 2008, 16:36

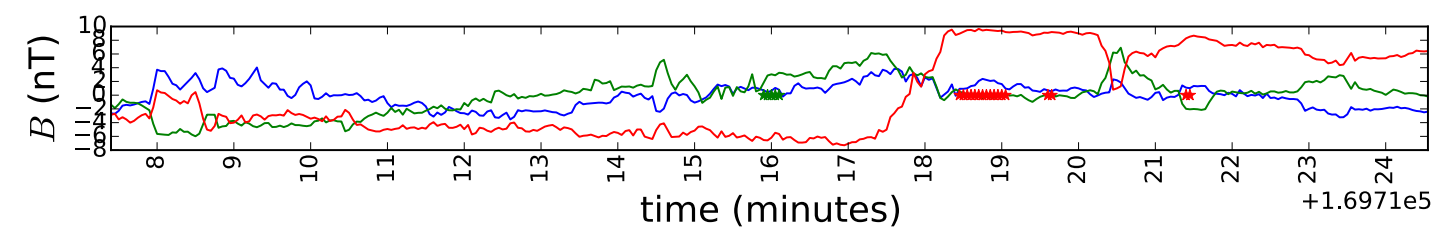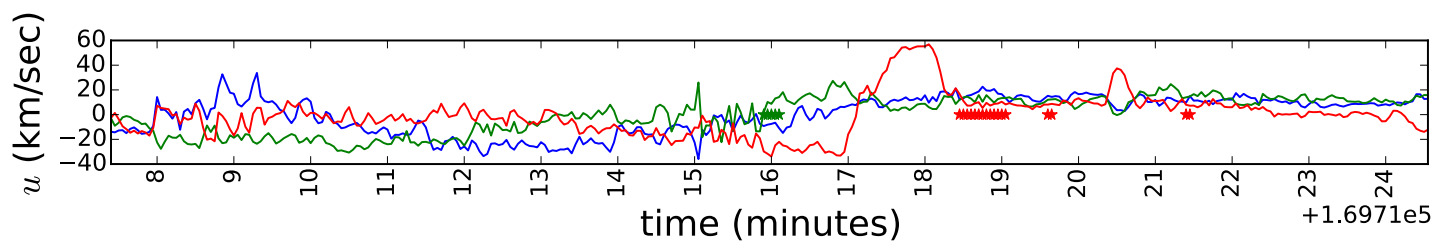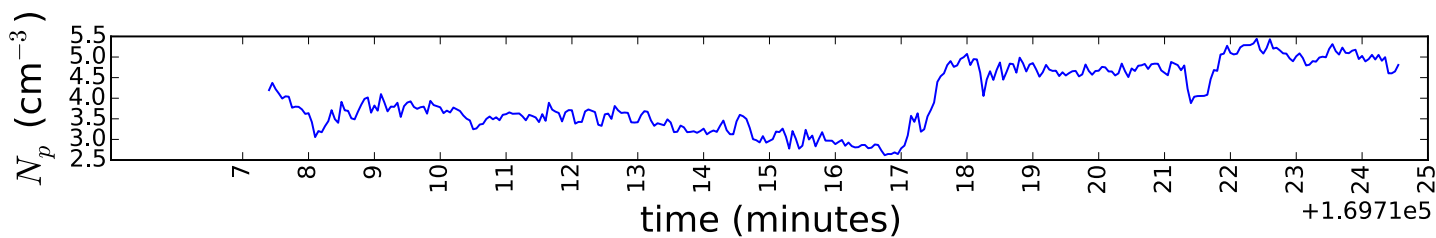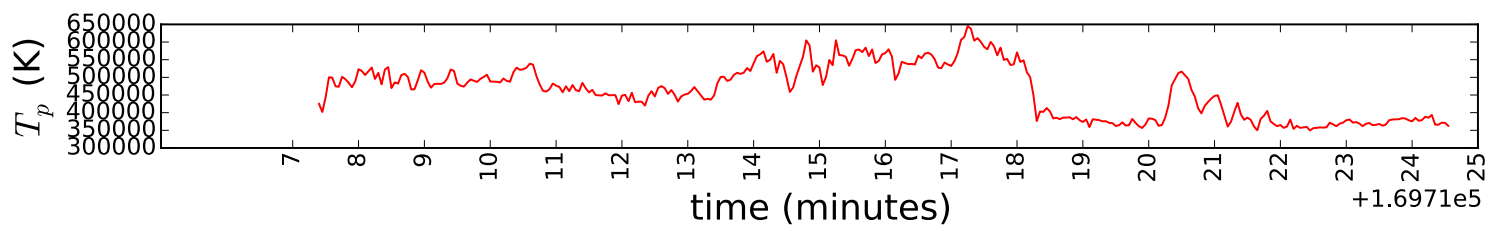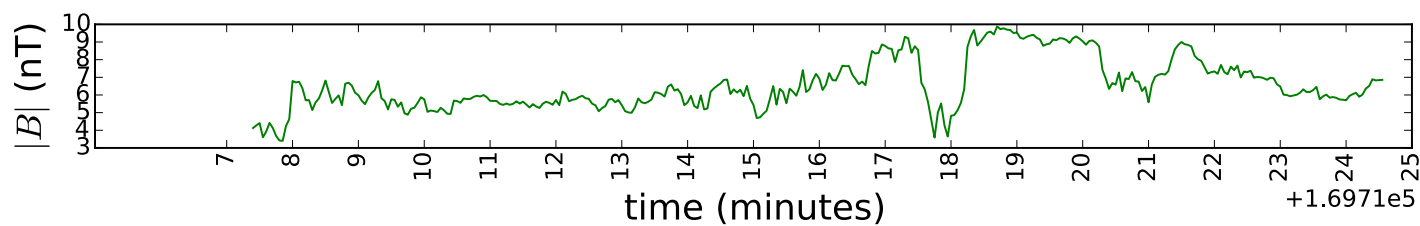

**Event 3:** January 26, 2006, 20:45

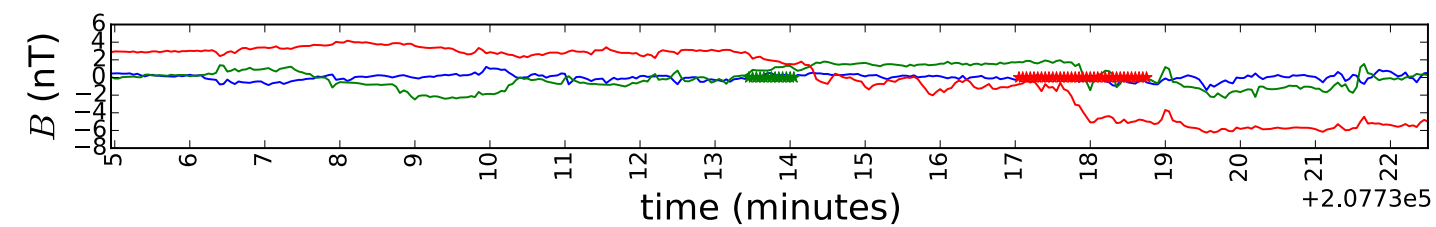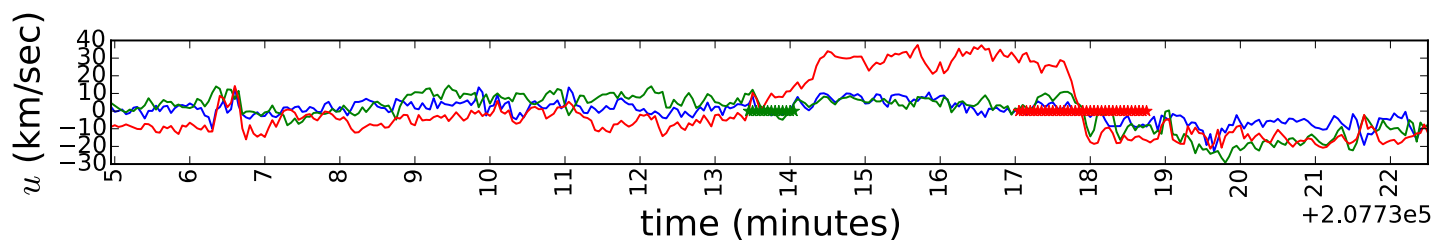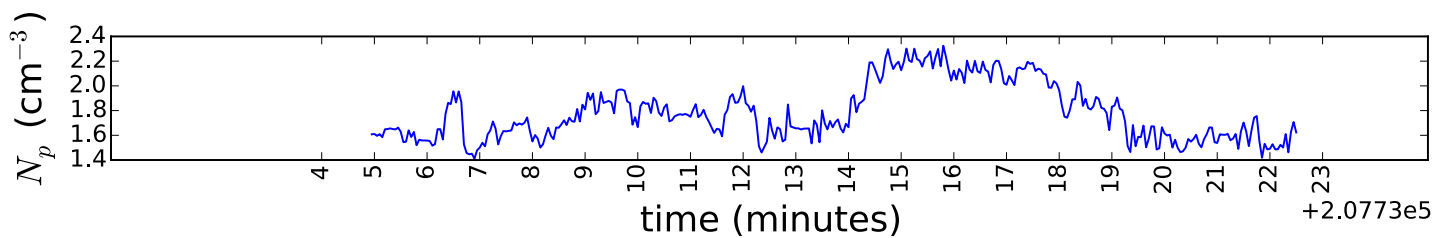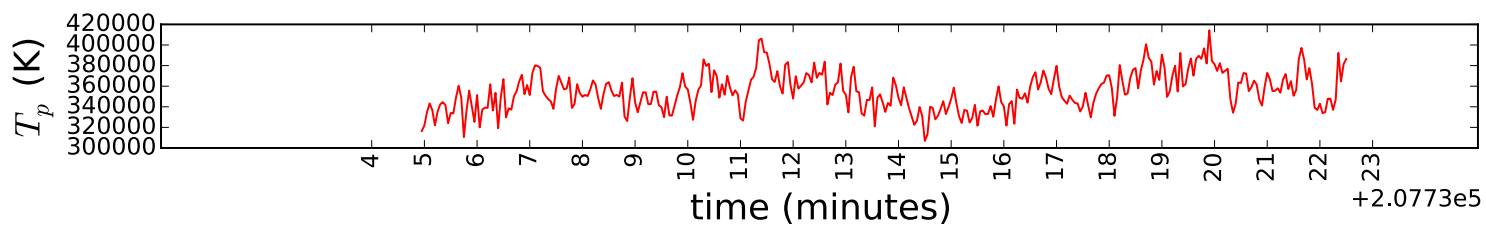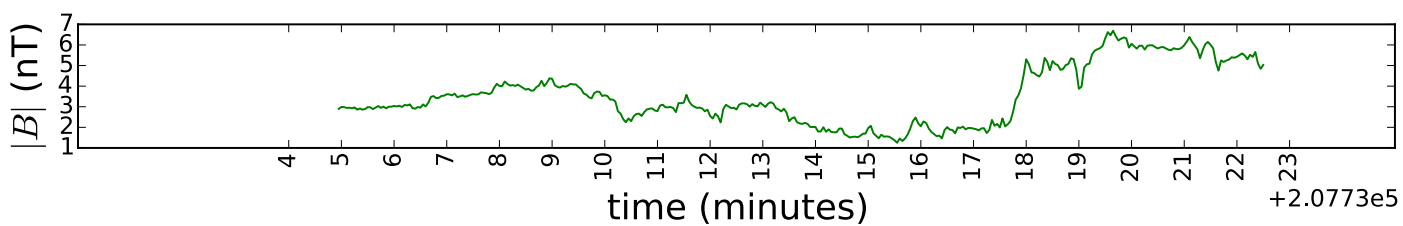

**Event 4:** February 22, 2006, 06:24



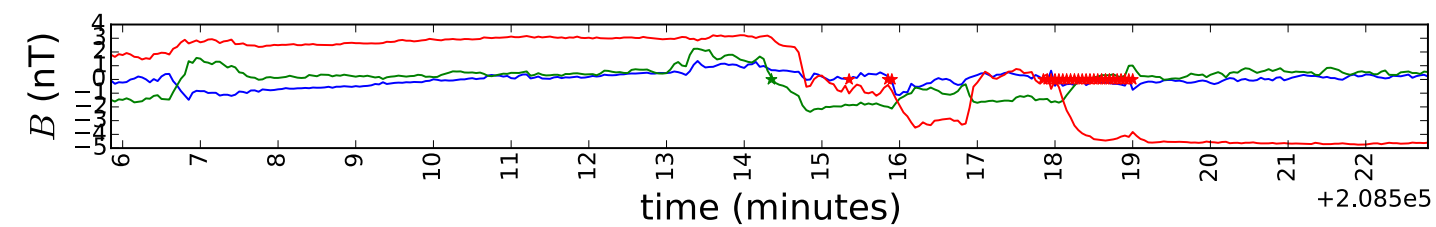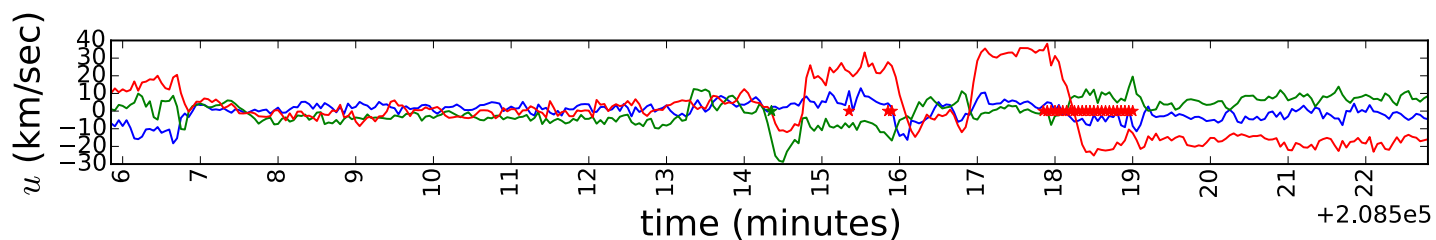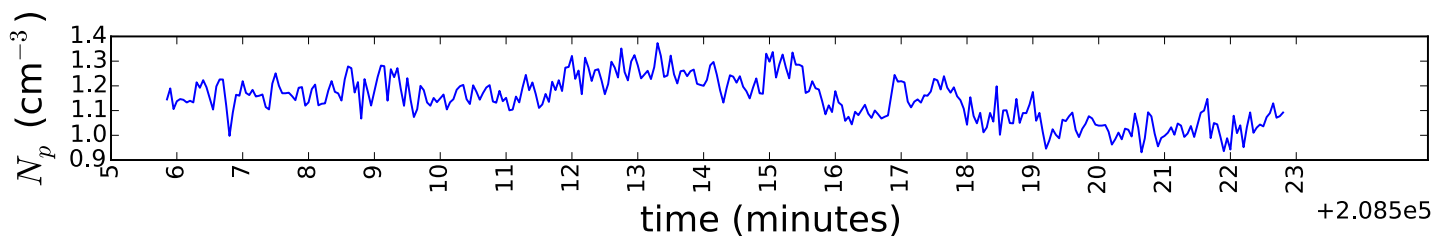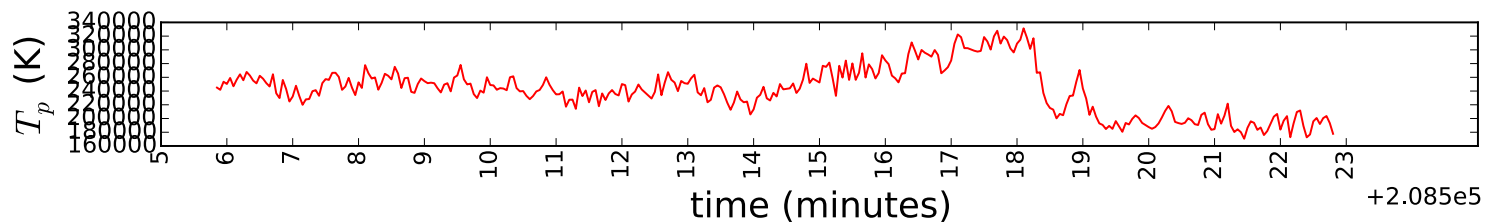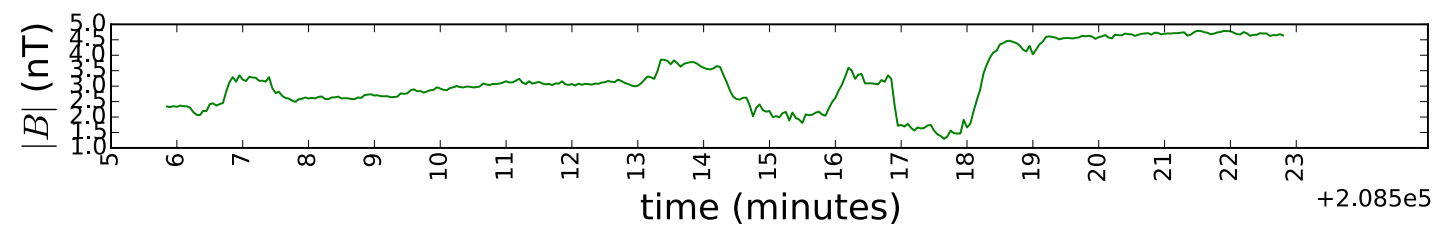

**Event 5:** February 21, 2006, 19:15

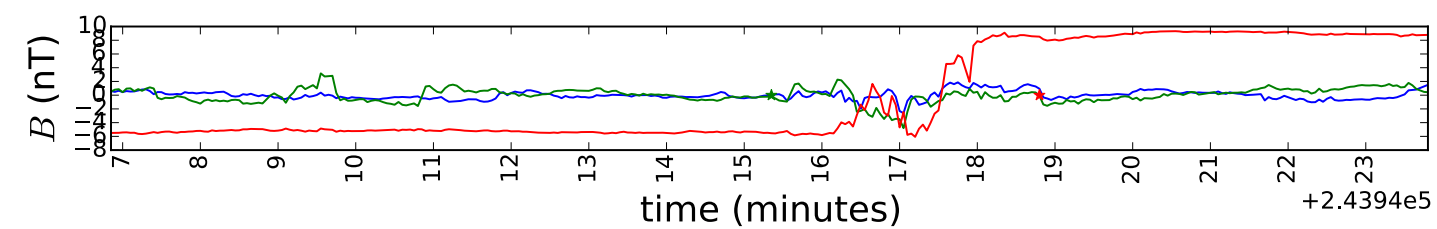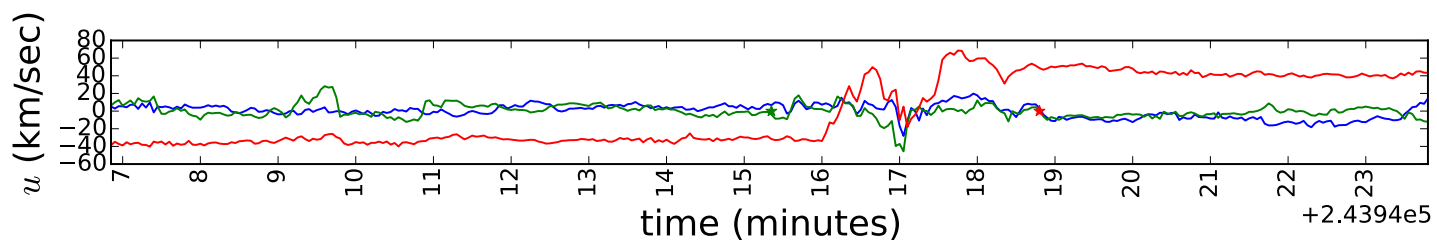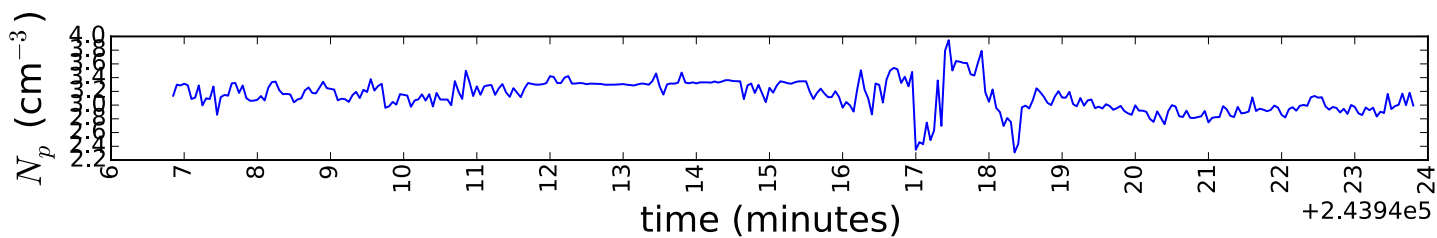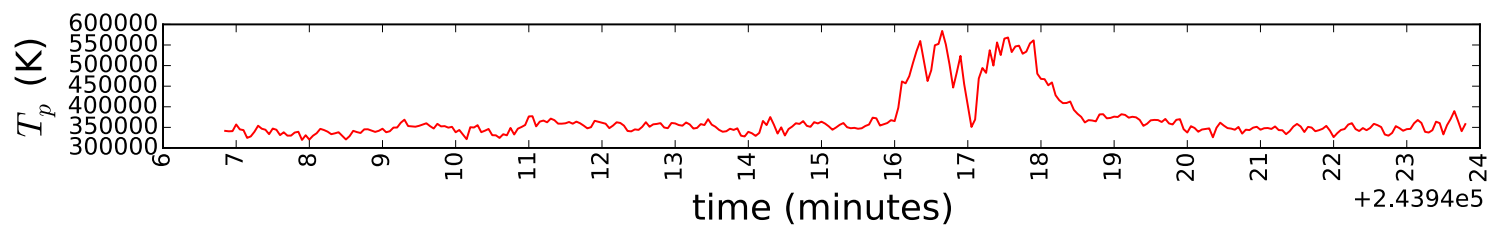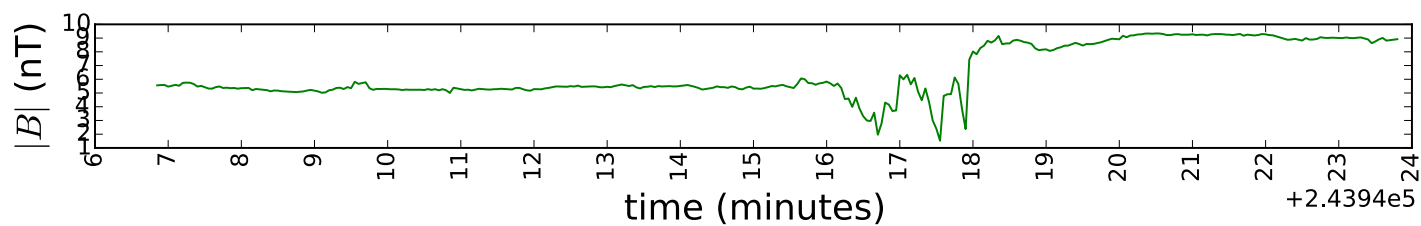

**Event 6:** March 19, 2006, 09:55

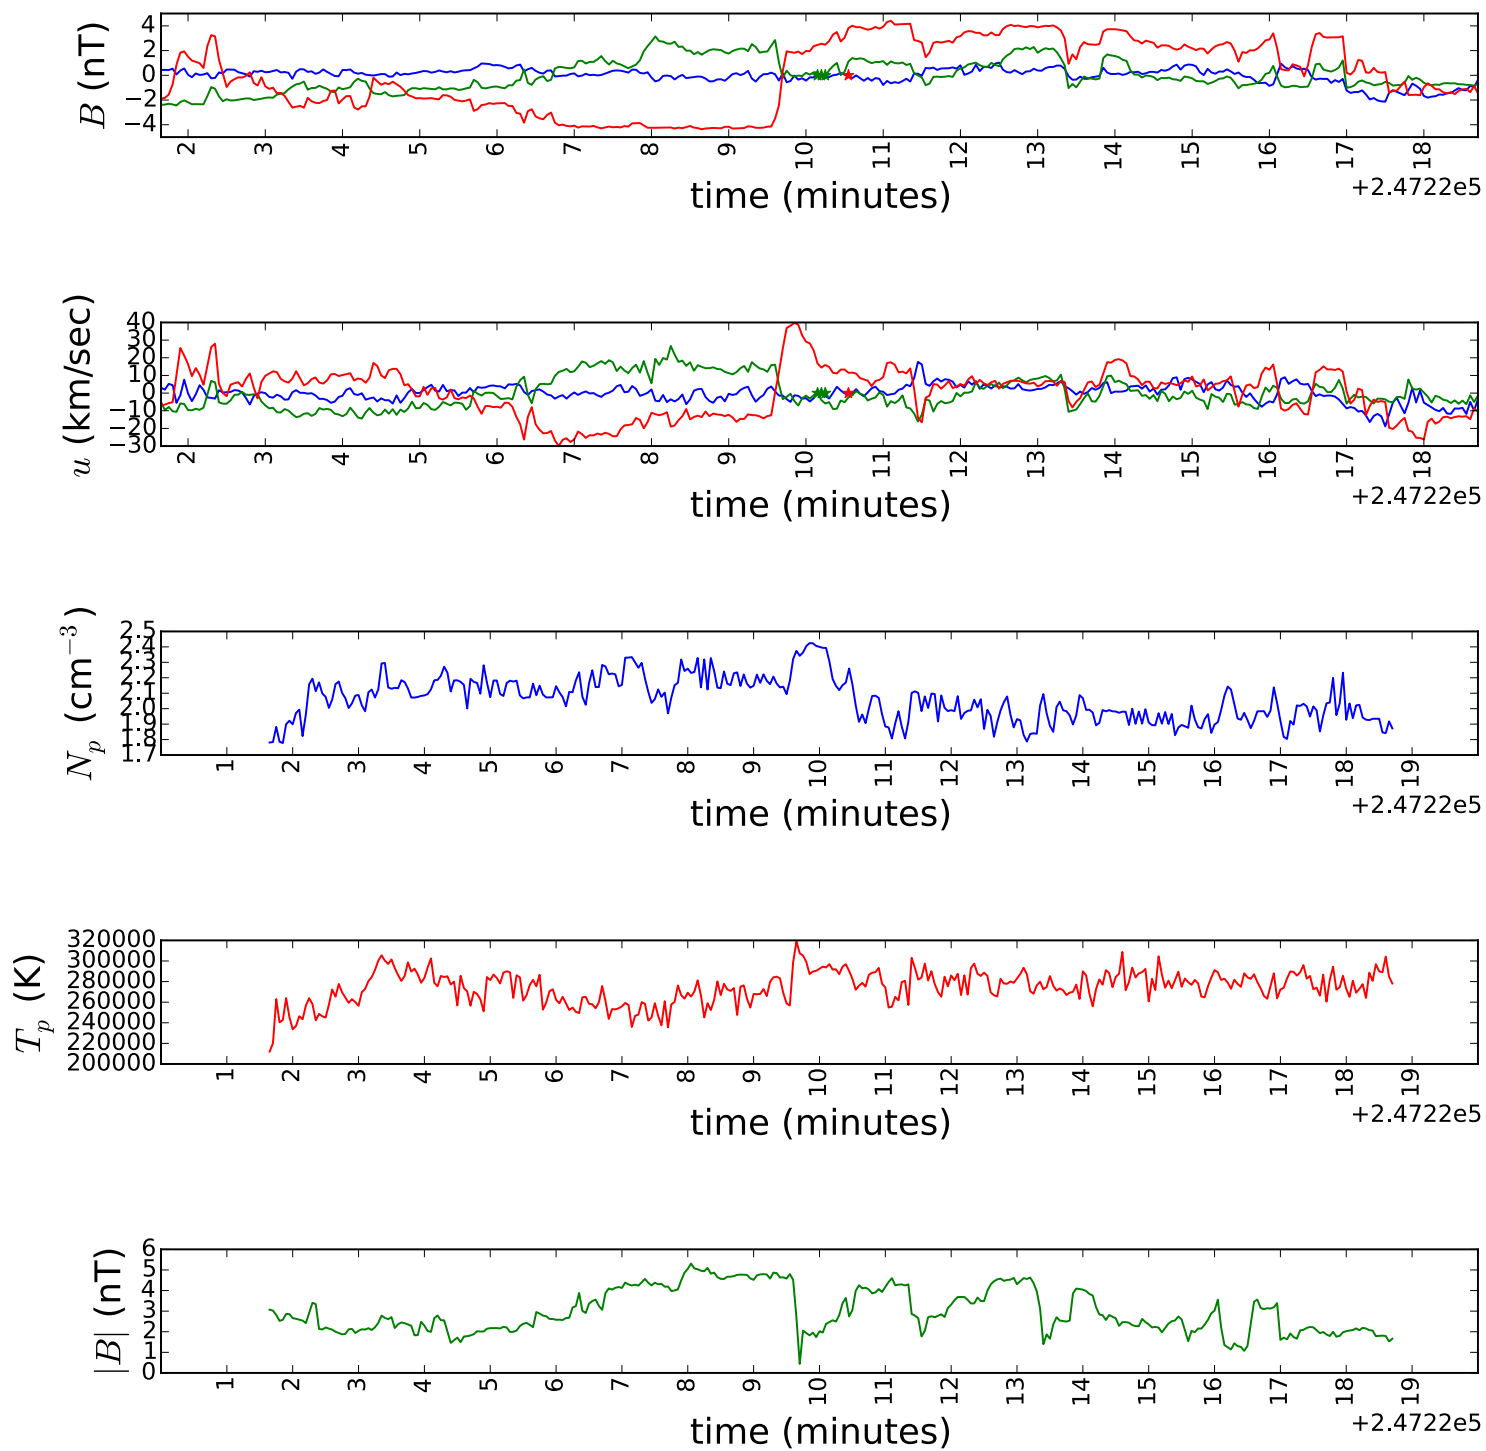

**Event 7:** March 21, 2006, 16:28

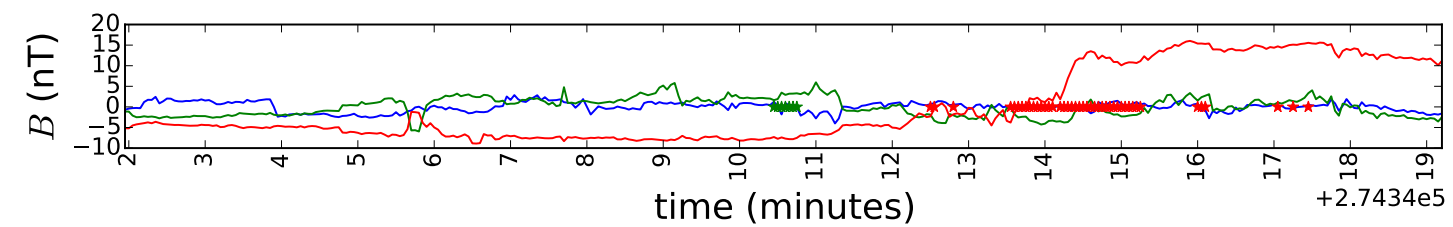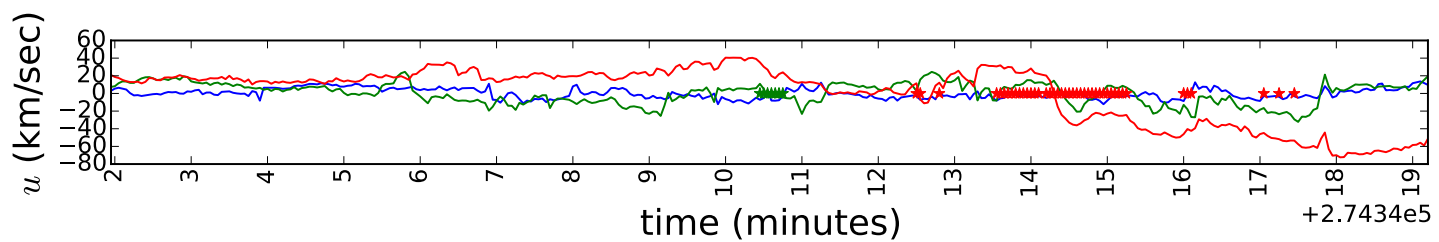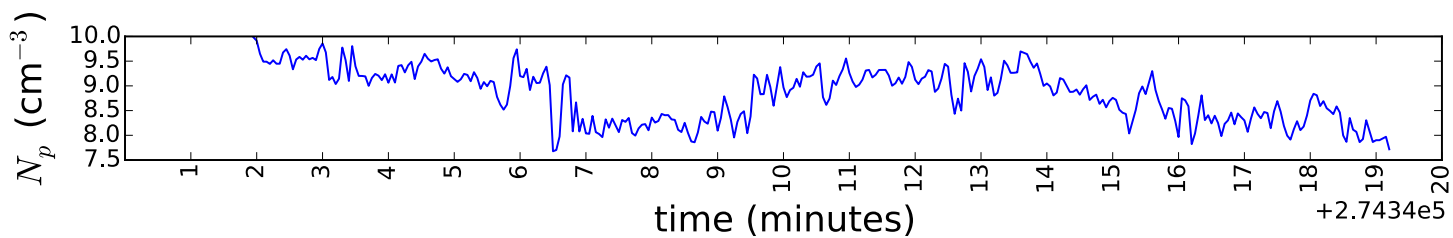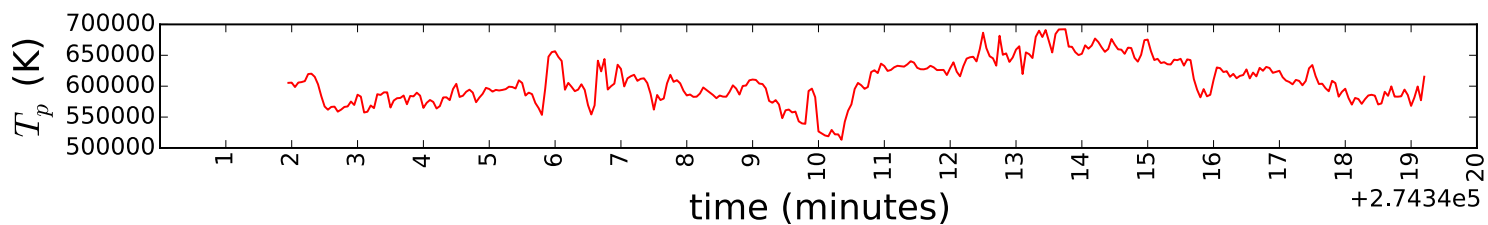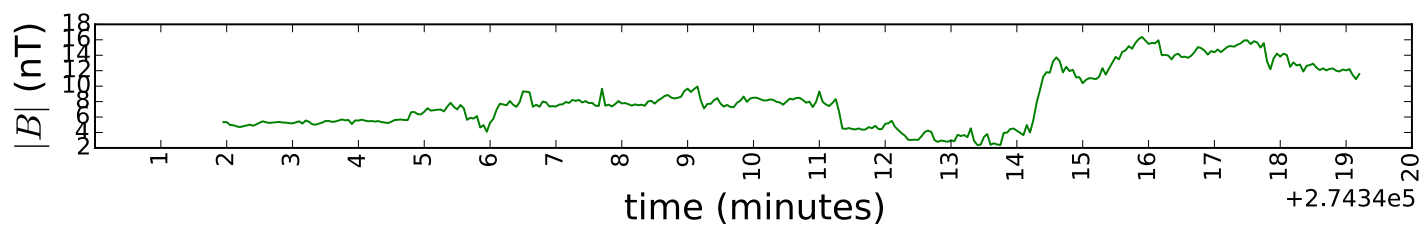

**Event 8:** April 09, 2006, 12:30

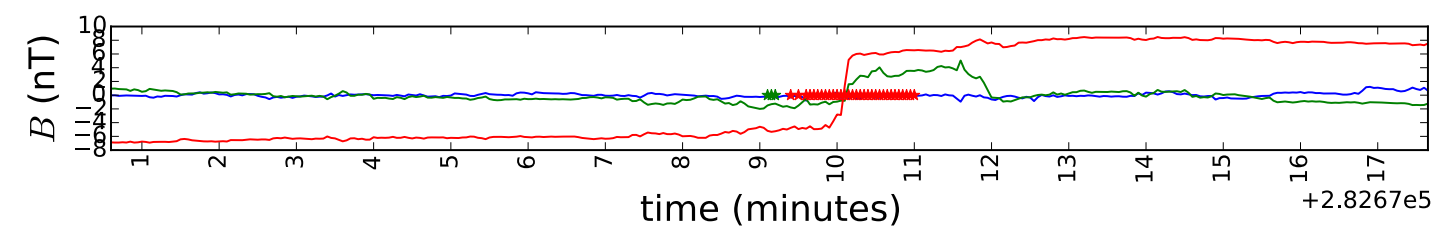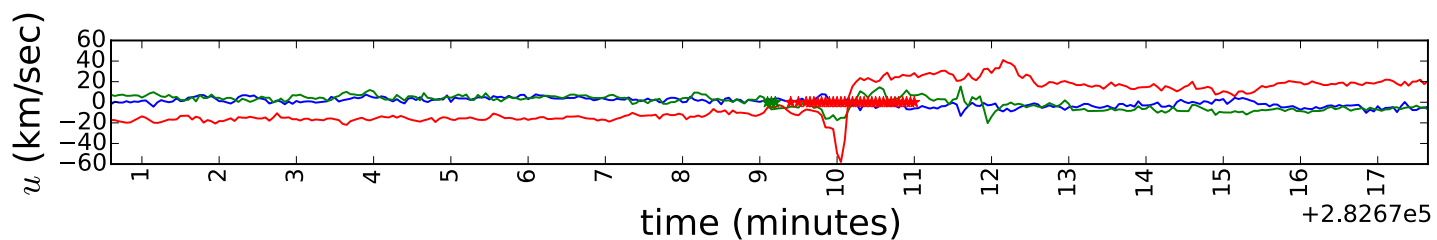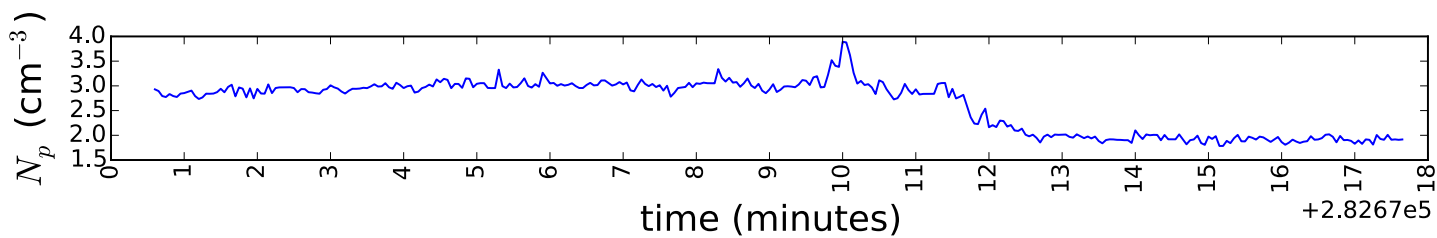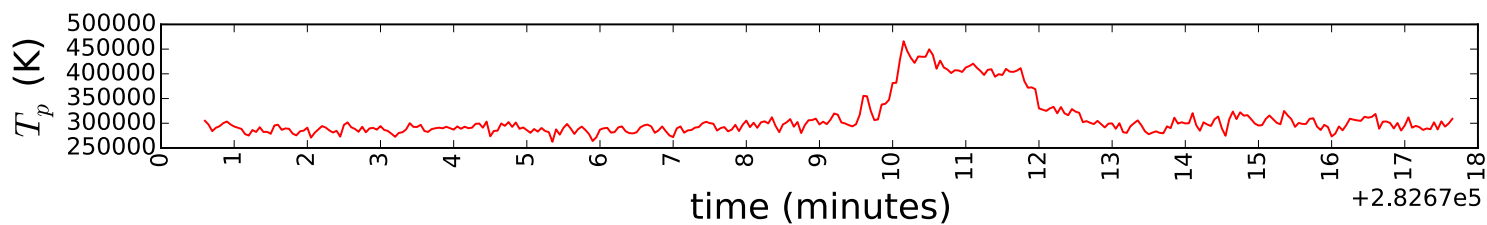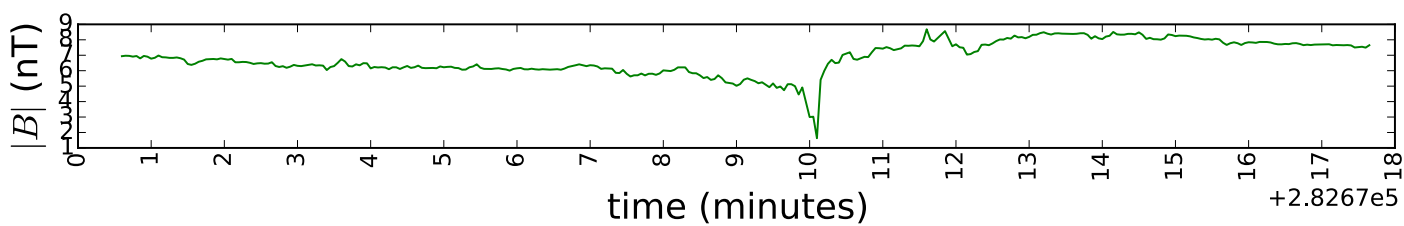

**Event 9:** April 15, 2006, 07:19

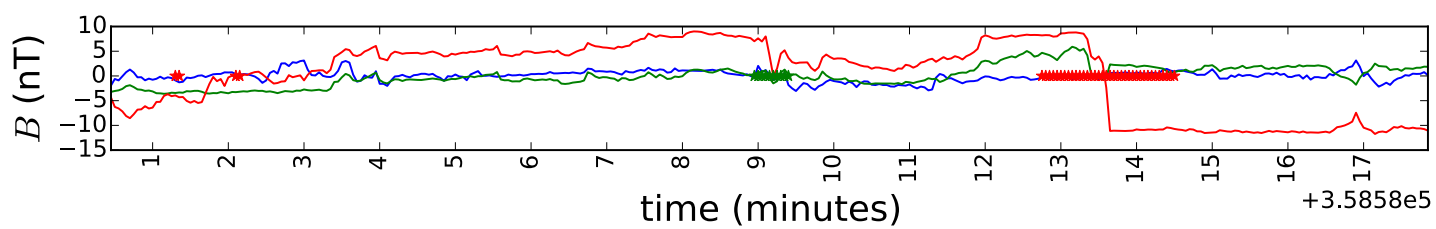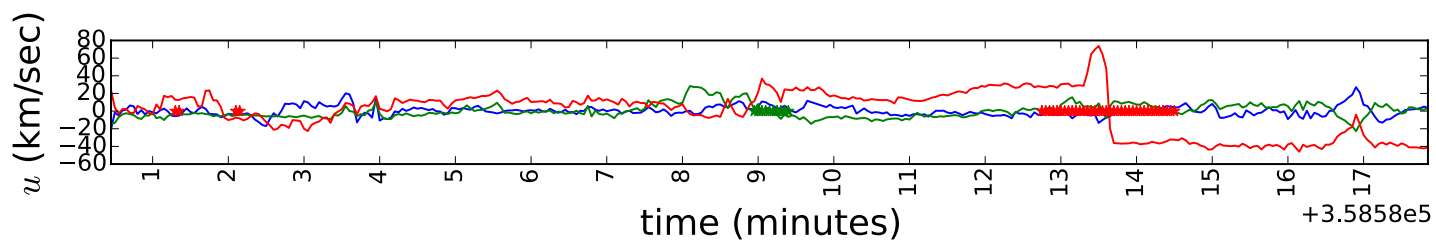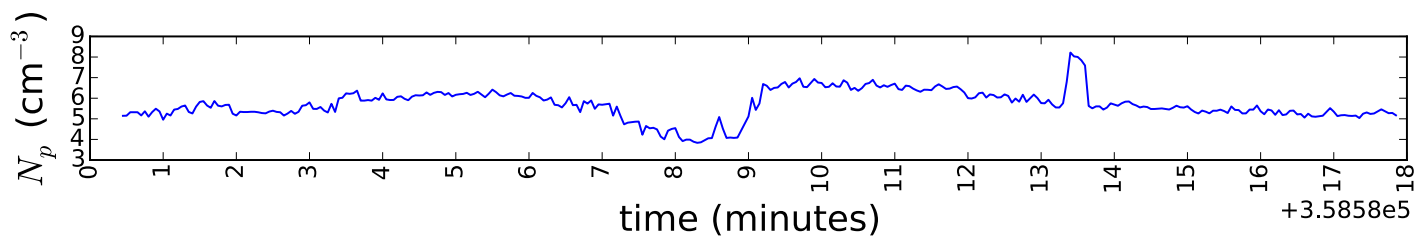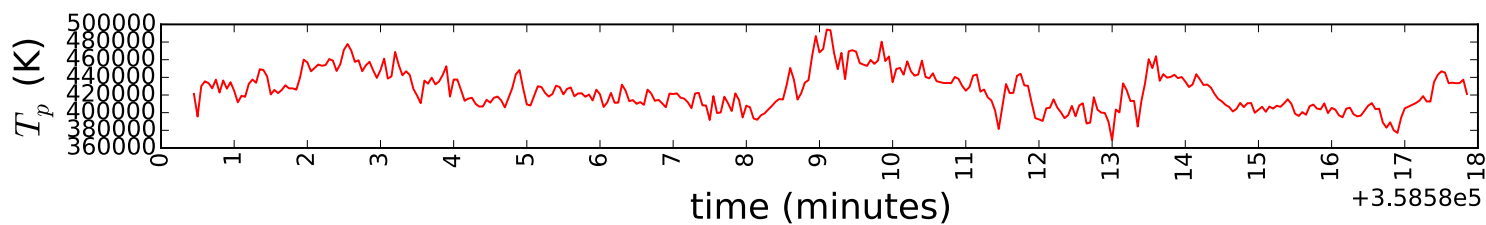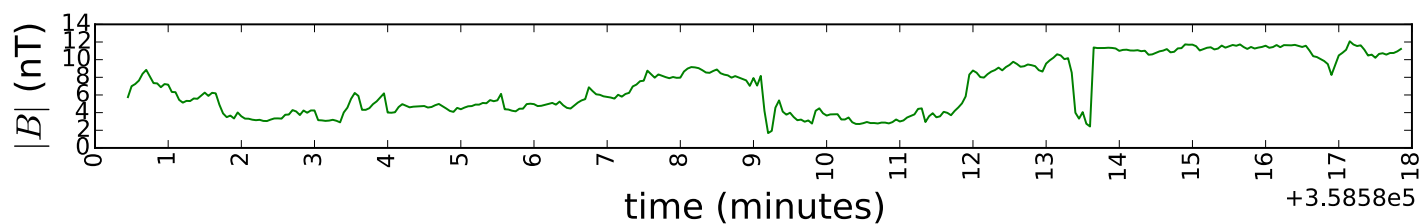

**Event 10:** June 07, 2006, 00:28

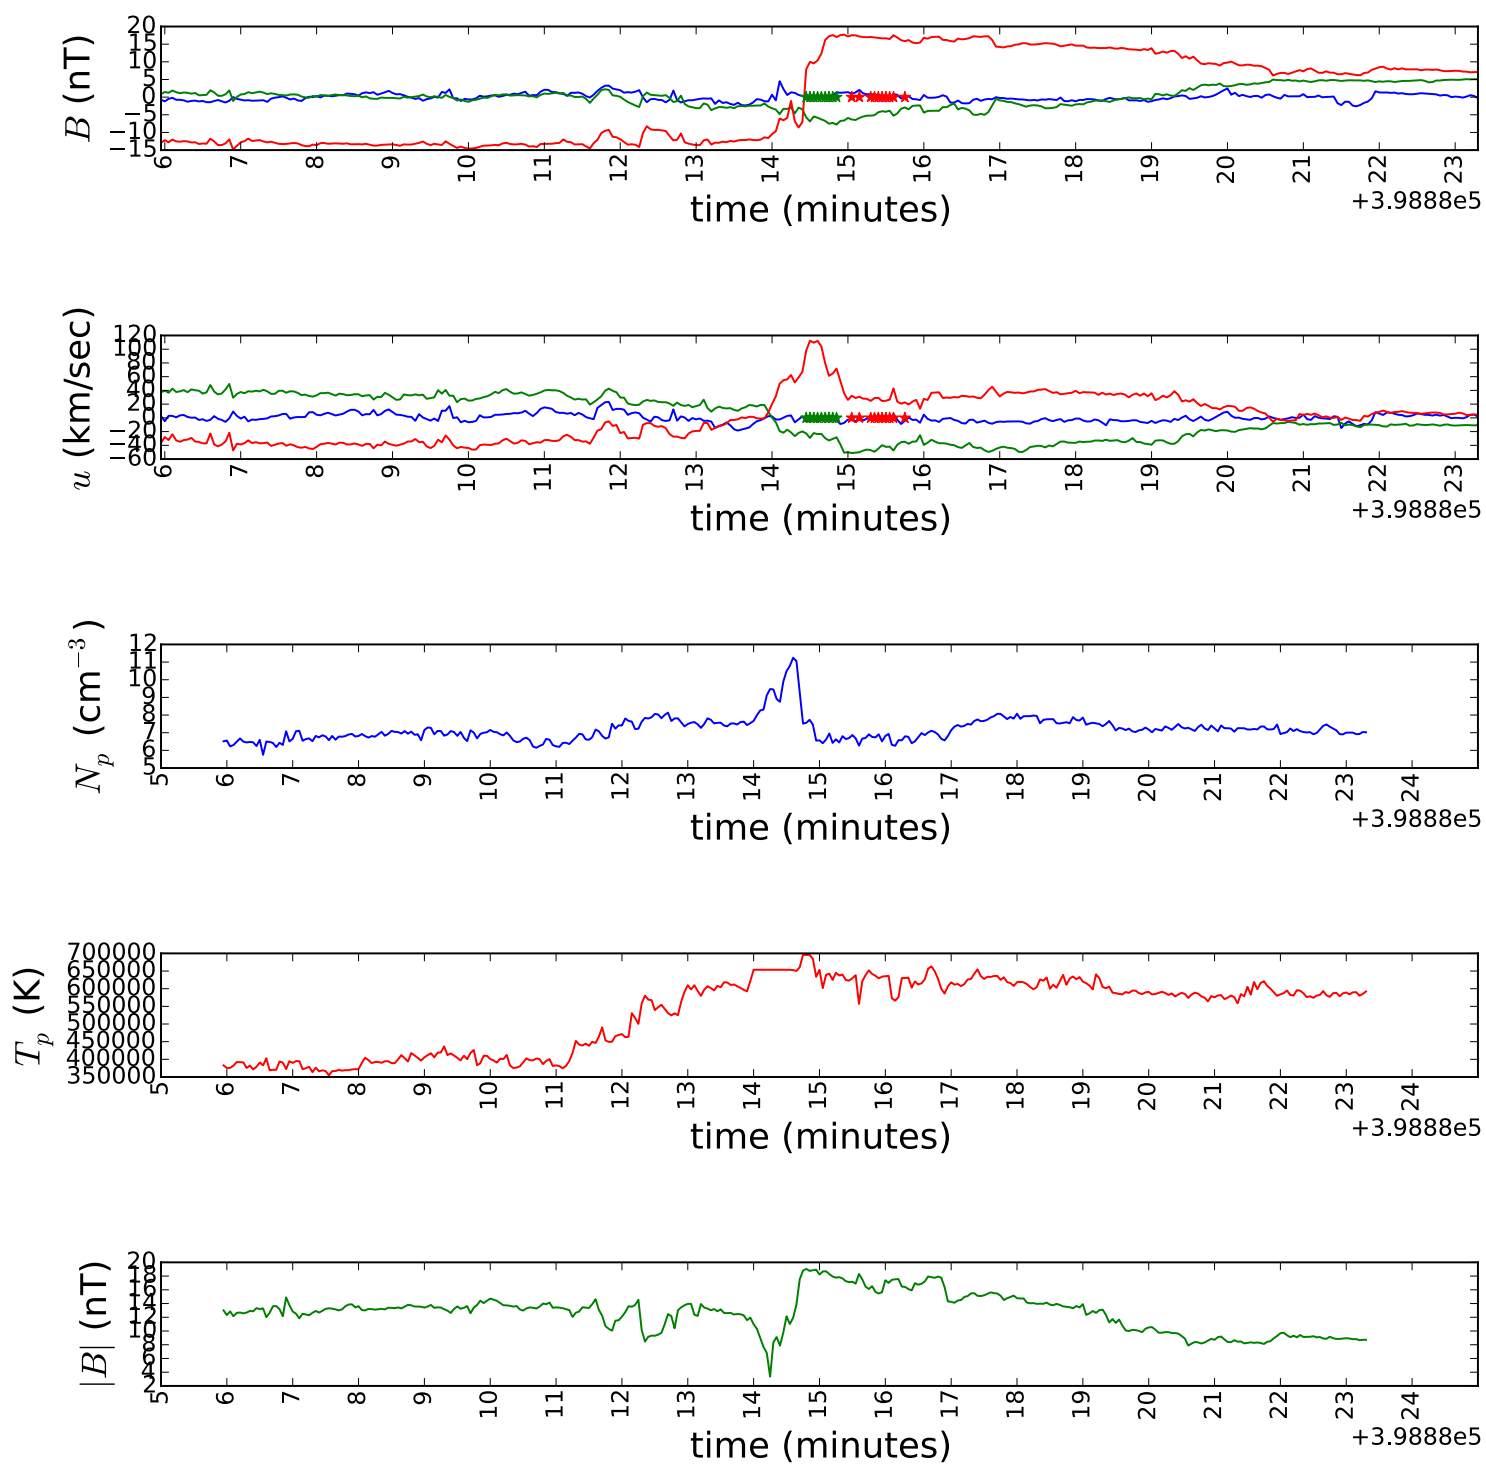

**Event 11:** July 05, 2006, 00:14

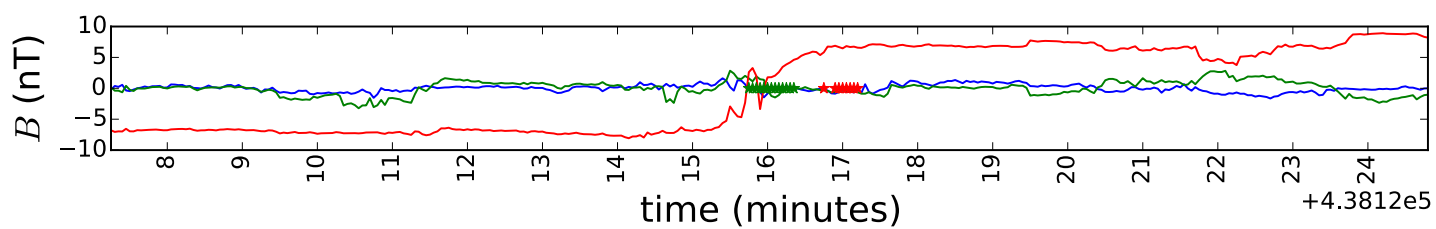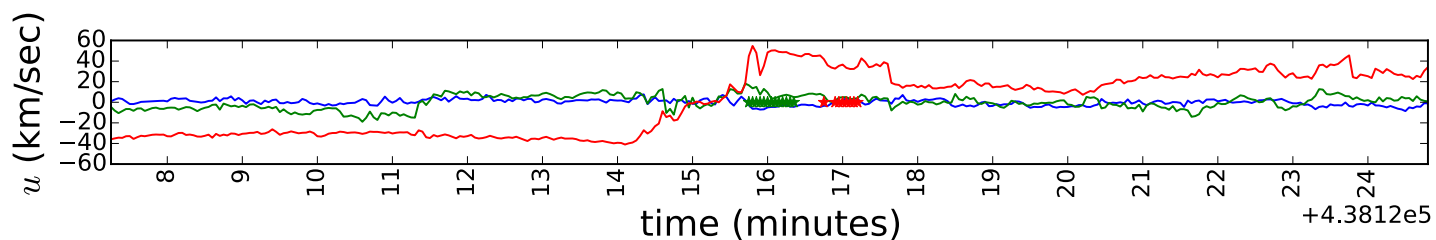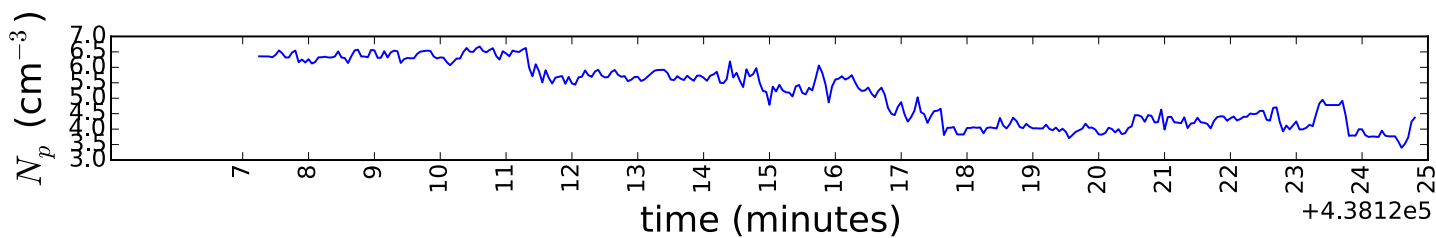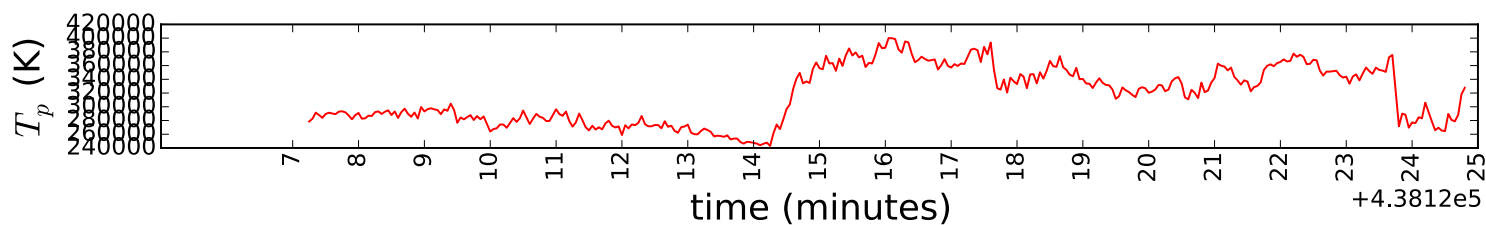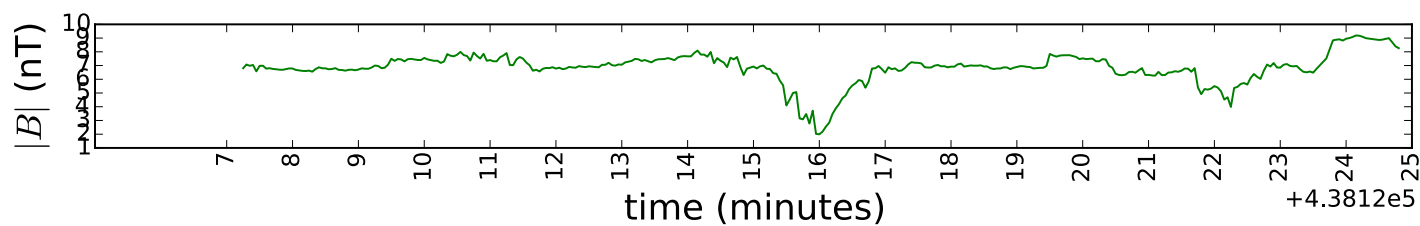

**Event 12:** August 01, 2006, 06:15



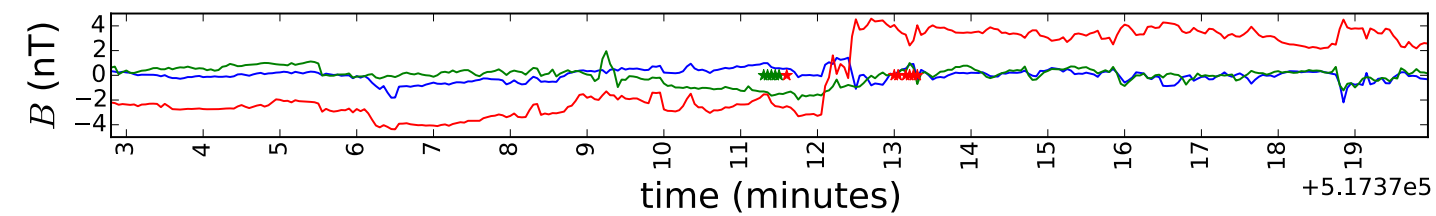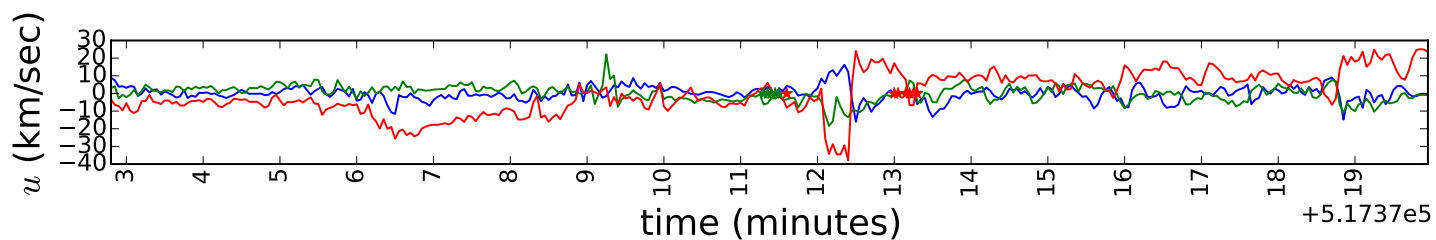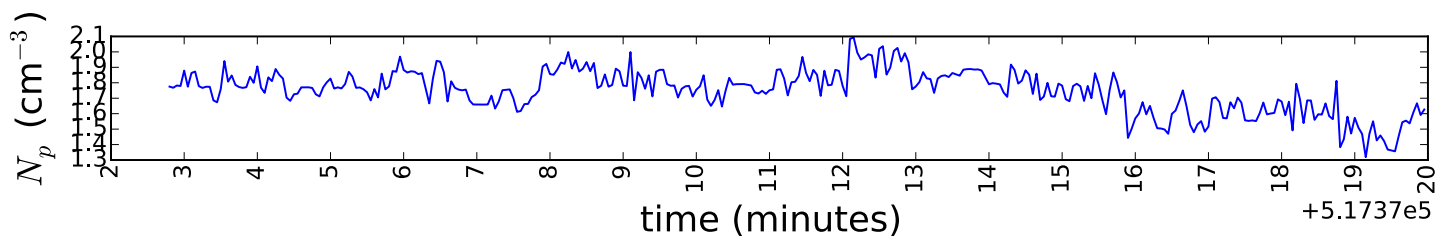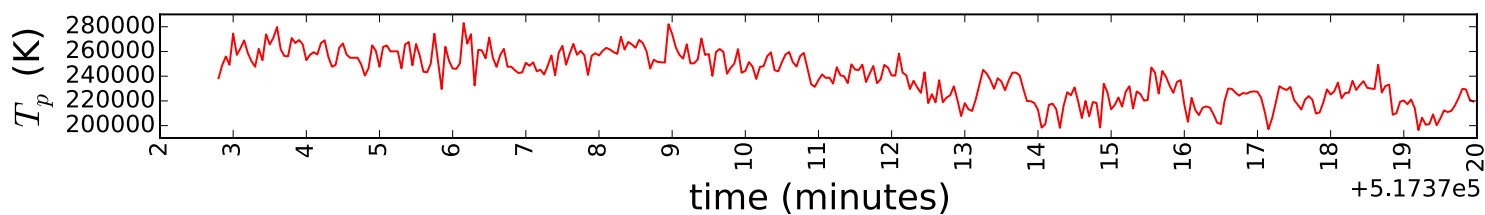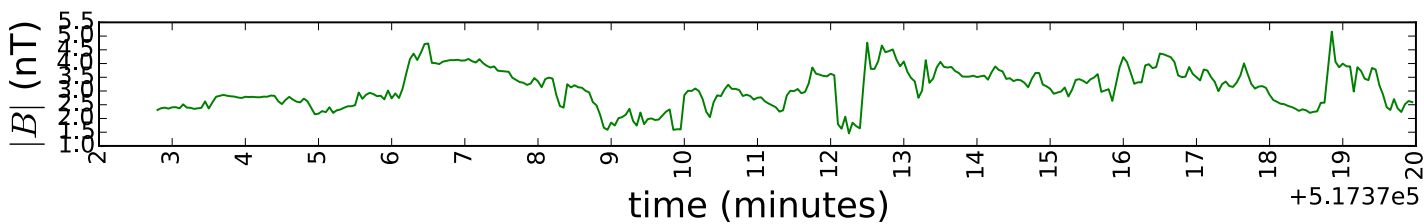

**Event 13:** September 25, 2006, 07:01
