# Supplementary material for: Inertial-Range Reconnection in Magnetohydrodynamic Turbulence and in the Solar Wind
Source: arXiv:1503.00509 ancillary file (2015-03-02)
Supplement: Supplementary file 7 [file increment_comparison.pdf]

## Increment Comparison Documentation

Our selection criterion for “large-scale reconnection events” involves conditions on the magnetic and velocity increments across specified time-separations, in the case of the *Wind* spacecraft observations, and specified space-separations, in the case of the MHD simulation. In order to apply precisely analogous selection criteria to the two datasets, we had to identify a statistical correspondence between these types of separations in the two datasets. As reported in the main body of the Letter, our approach was to make a careful comparison of the probability density functions (PDFs) of magnetic-field increment magnitudes  $|\delta \mathbf{B}|$  from the MHD simulation and from the *Wind* spacecraft data for 2008 January 14 04:40:00 to January 21 03:20:00. We also compared cumulative distribution functions (CDF’s) or, rather, the co-CDF’s defined by

$$1-\text{CDF}(x) = \int_x^\infty dy \text{ PDF}(y).$$

These co-CDF’s are especially useful to determine whether probabilities of large fluctuations (“tail events”) are the same for two different distributions.

We found that the PDF’s and co-CDF’s of  $|\delta \mathbf{B}|$  at space-separations  $r=n \, dx$  in the MHD database compare quite well to the corresponding PDFs and co-CDF’s for the *Wind* data at time-separations  $\tau = n \times (0.18 \text{ sec})$  for the same choice of  $n$ , with values of  $n$  corresponding to the inertial-range of both flows. Thus, the grid spacing  $dx$  in the database is in good statistical relation to 0.3 minutes (18 seconds) in the solar wind time series. On pp.1-7 of the document “increment-comparison.pdf” are plotted the PDF’s and co-CDF’s of these corresponding magnetic-field increment magnitudes in the MHD simulation and in the *Wind* observations for  $n=6,10,16,24,32, 44, 57$  and also for the velocity-increment magnitudes  $|\delta \mathbf{u}|$  in these two datasets at the same separations. Since the correspondence  $dx \sim 0.18 \text{ sec}$  was optimized for the magnetic increments, it is not surprising that PDF’s and co-CDF’s agree best for  $|\delta \mathbf{B}|$ . However, the agreement is quite good, especially for small  $r, \tau$ , where the agreement between MHD simulation and solar-wind statistics is good up to 4 rms, but generally good up to 2 rms even for  $r=L, \tau=T$ . The correspondence  $dx \sim 0.18 \text{ sec}$  also works reasonably well for PDF’s and c-CDF’s of  $|\delta \mathbf{u}|$ , with these quantities in the MHD simulation and the solar-wind dataset agreeing rather well up to at least 2 rms. Although we do not show the results here, we have found that the same correspondence of statistics also works well for the fast regions of the other solar-wind dataset spanning 2005/10/01–2007/05/01.

With the correspondence  $dx \sim 0.18 \text{ sec}$  and given the (magnetic) integral-scale  $L=0.35$  in the MHD simulation, the turbulent outer time-scale  $T$  of the 2008 solar wind dataset is estimated to be approximately 17.1 minutes. This determination of  $T$  also agrees well with the upper limit of the time range where the 2/3rd power-law in the structure-function of magnetic-field increments is observed in the *Wind* data. The structure functions of  $\mathbf{u}$  and  $\mathbf{B}$  are plotted on the final page of the catalogue, for both the MHD simulation and for the entire set of *Wind*

## Increment Comparison Documentation

spacecraft data of high-speed wind. All of the structure functions are presented as functions of separations normalized by integral scales ( $\tau/T$  for the Wind data and  $r/L$  for the MHD simulation) and the structure-functions are also normalized by their values at integral-scale separations. For completeness, these values are recorded here:

Wind observations:  $S_2^B(T) = (2.151 \text{ nT})^2$ ,  $S_2^u(T) = (18.28 \text{ km/sec})^2$

MHD simulation:  $S_2^B(L) = 0.2600$ ,  $S_2^u(L) = 0.1694$

The simulation and solar-wind datasets both show inertial-ranges which extend up to the identified integral scales, but also show several differences in their inertial-range behavior. As is common for high-speed solar wind at 1 AU, especially at solar minimum, the magnetic-field structure-function satisfies a 2/3-law scaling in the inertial-range, whereas the the velocity structure-function satisfies better a 1/2-law scaling (corresponding to -5/3 and -3/2 power-laws for the energy spectra of magnetic and velocity fields, respectively). In the MHD simulation, somewhat surprisingly, the structure-functions of both fields satisfy better a 2/3-law scaling than a 1/2-law, although the Fourier energy spectra of both fields appear closer to a -3/2 power-law. The inertial-range for the solar wind appears to extend to substantially smaller scales than the inertial-range for the MHD simulation. The two datasets show roughly similar behavior at scales greater than the inertial-range, with the magnetic energy spectrum flattening and the kinetic energy spectrum rising to greater values. However, the solar-wind contains a much larger range of such scales, corresponding to the so-called “1/f-range” of the solar-wind spectra. This range is generally thought to consist of very large-scale, weakly-interacting force-free structures and Alfvén wave trains originating from the solar atmosphere. The MHD simulation completely lacks this super-structure of very large-scale features with lengths much greater than inertial-range scales, which can be subject to magnetic reconnection.

# PDFs and 1-CDFs for $B$ and $u$ increments: Comparison between JHUTB & Solar Wind

*Wind* data: 2008/01/14 04:40:00 – 2008/01/21 03:20:00

Showing correspondence between 1  $dx \approx .3$  minutes

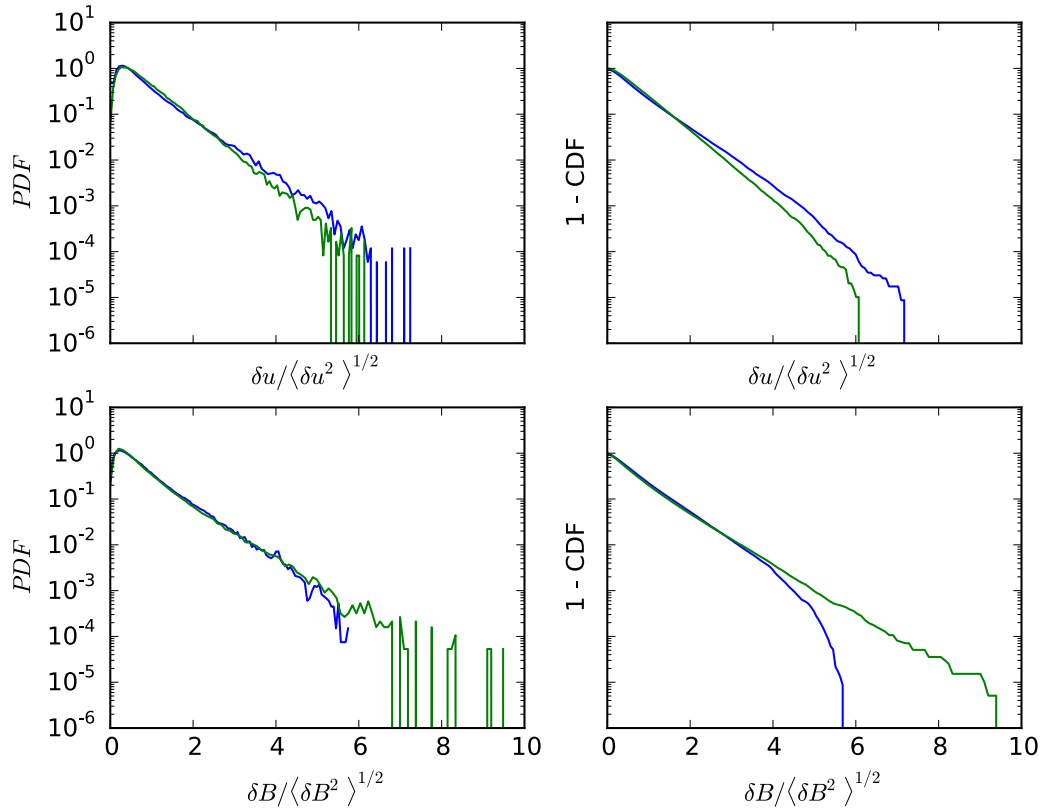

**Figure 1:** Database increments of 6  $dx$  (in green) and *WIND* increments of 1.8 minutes (in blue).

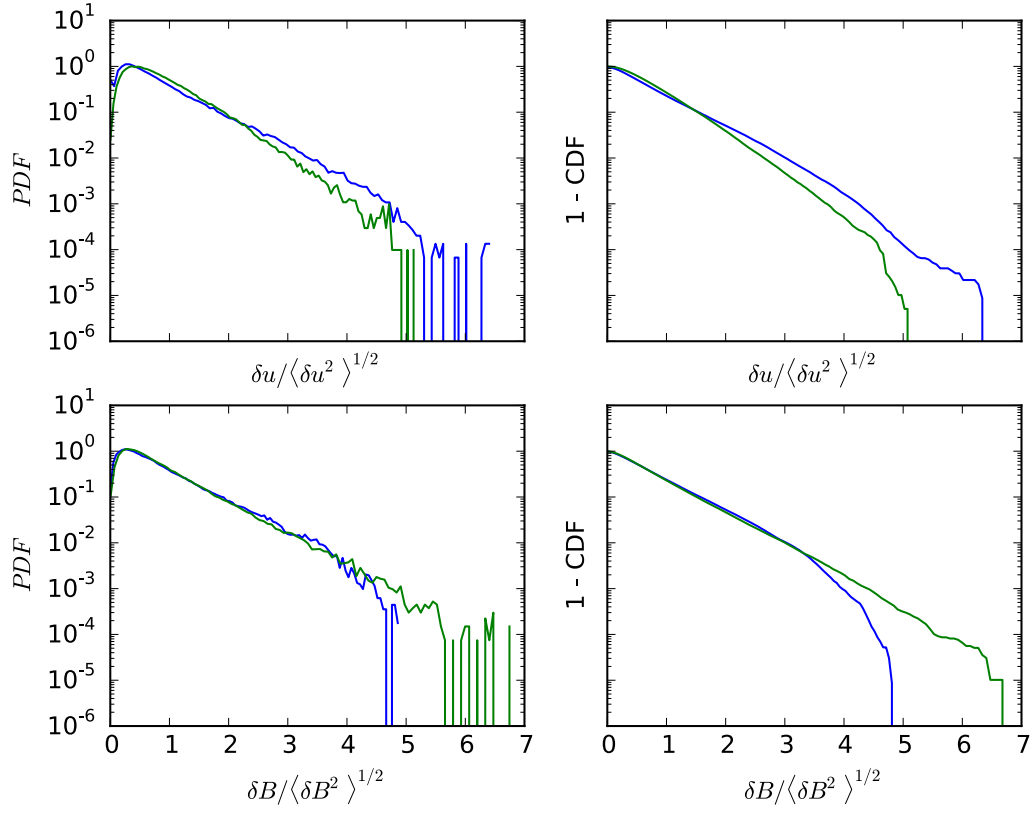

**Figure 2:** Database increments of 10  $dx$  (in green) and WIND increments of 3.0 minutes (in blue).

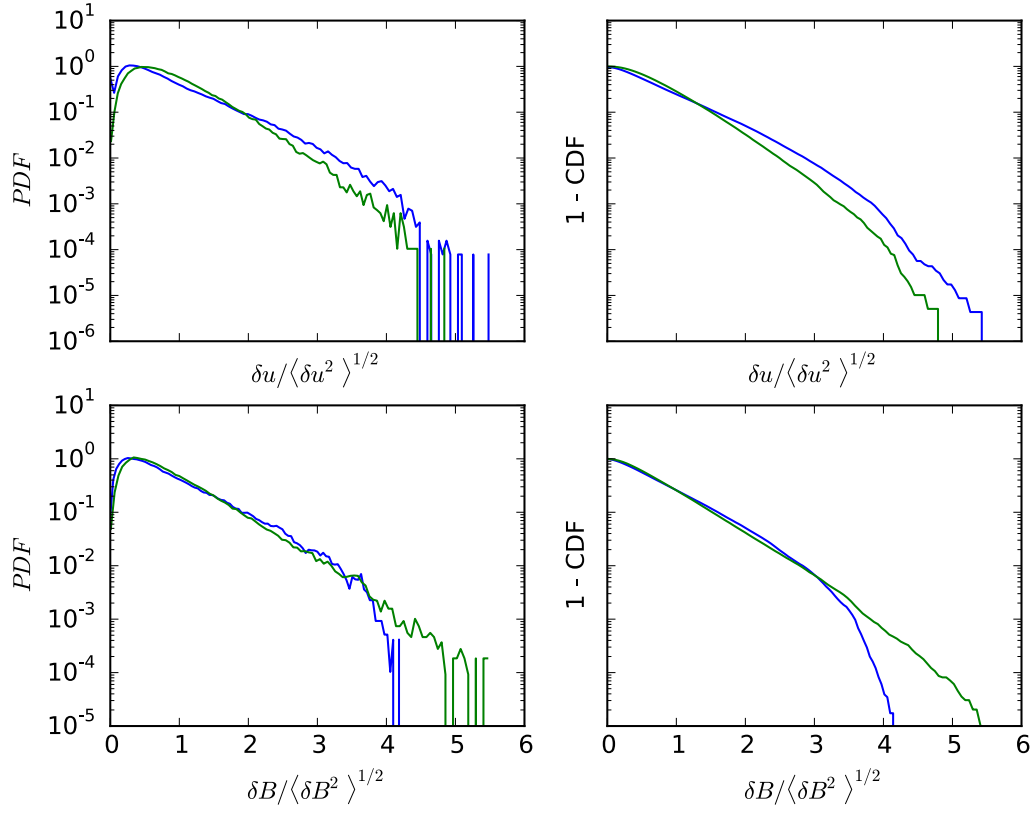

**Figure 3:** Database increments of 16  $dx$  (in green) and WIND increments of 4.8 minutes (in blue).

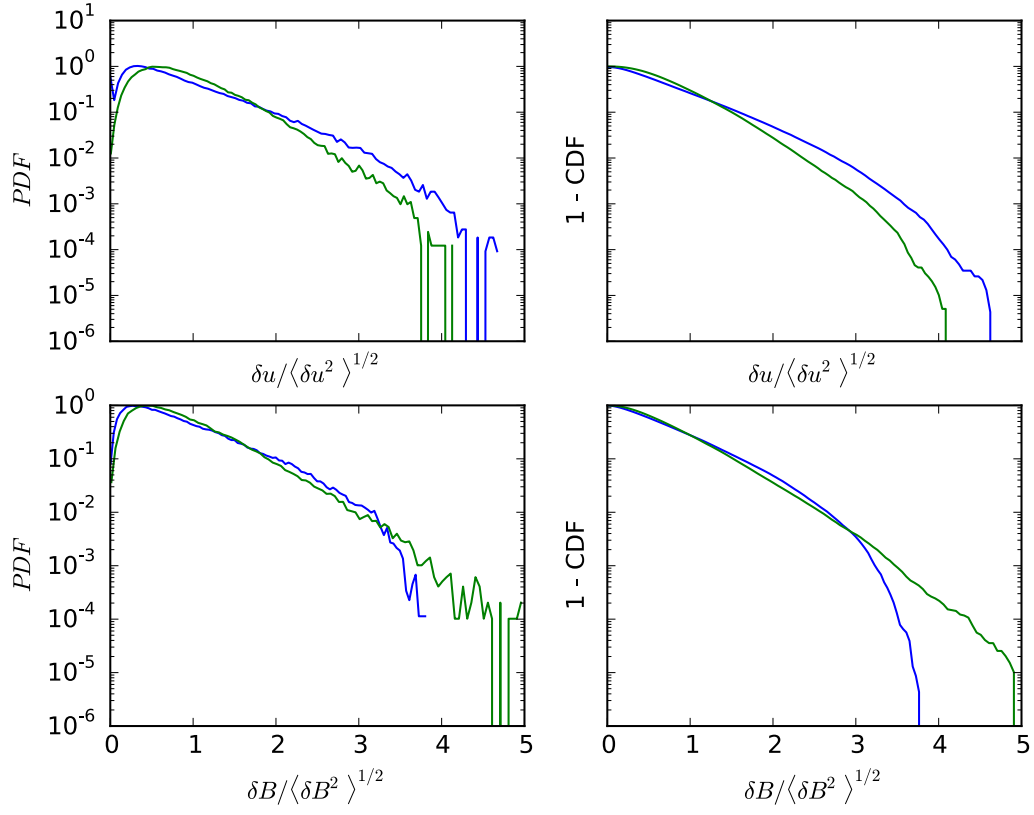

**Figure 4:** Database increments of 24  $dx$  (in green) and WIND increments of 7.1 minutes (in blue).

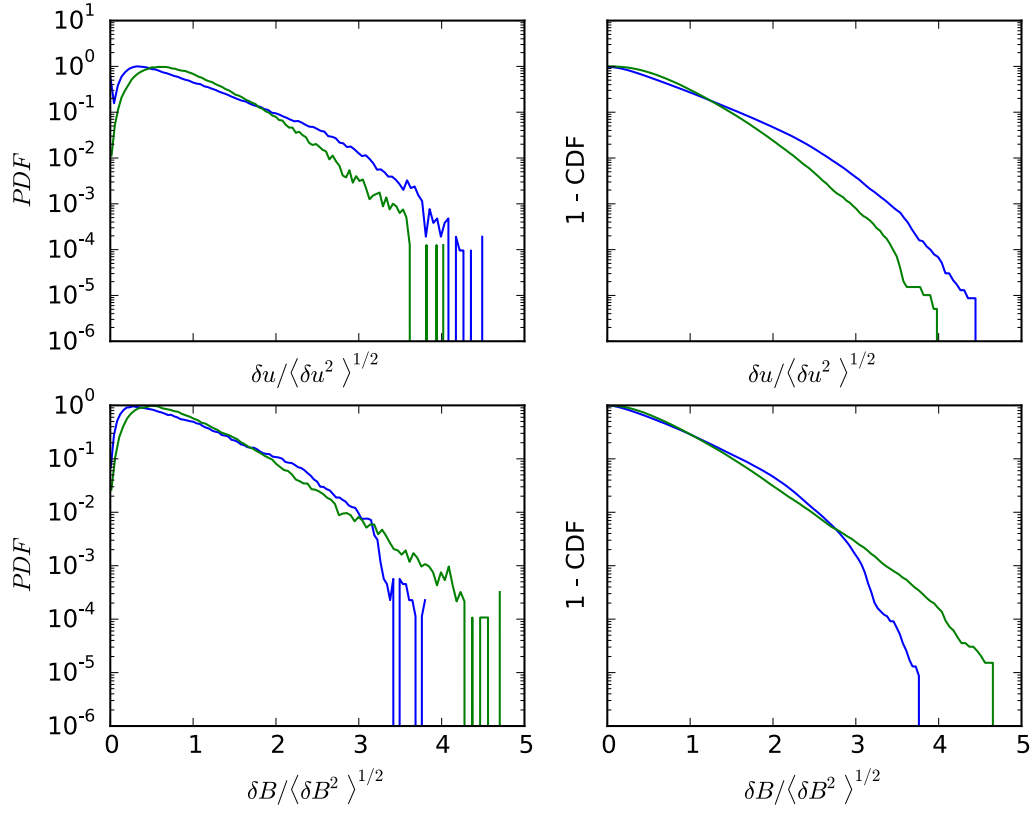

**Figure 5:** Database increments of 32  $dx$  (in green) and *WIND* increments of 9.5 minutes (in blue).

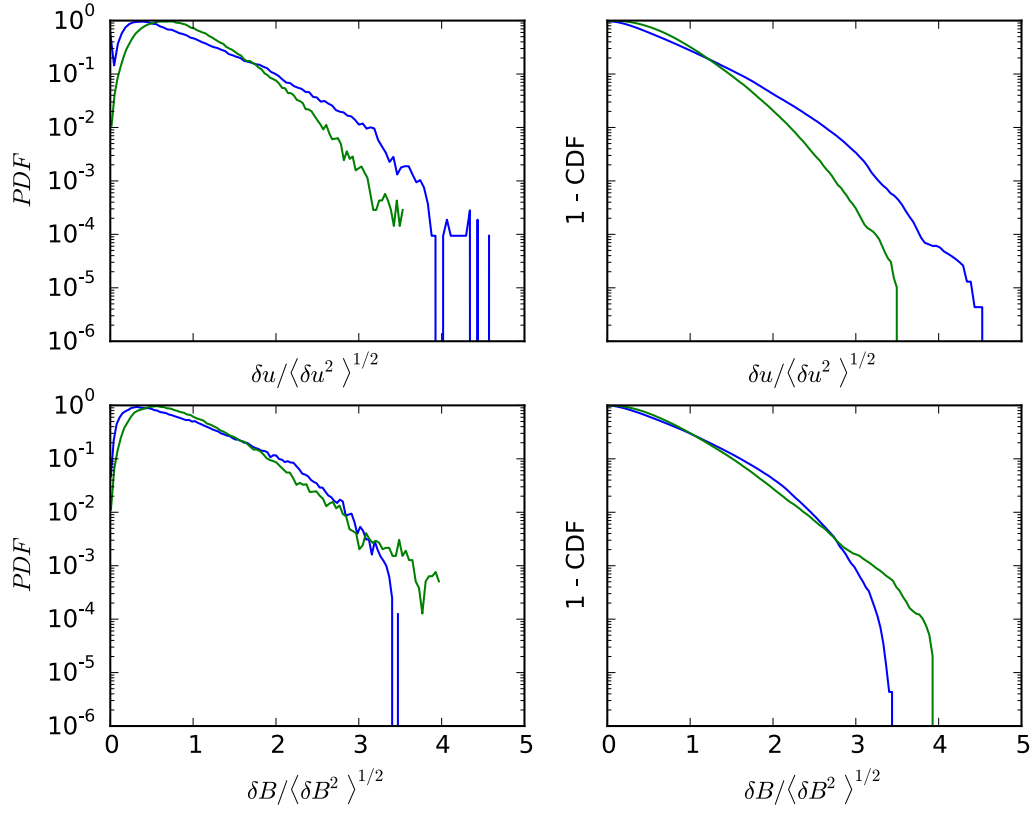

**Figure 6:** Database increments of 44  $dx$  (in green) and  $WIND$  increments of 13.1 minutes (in blue).

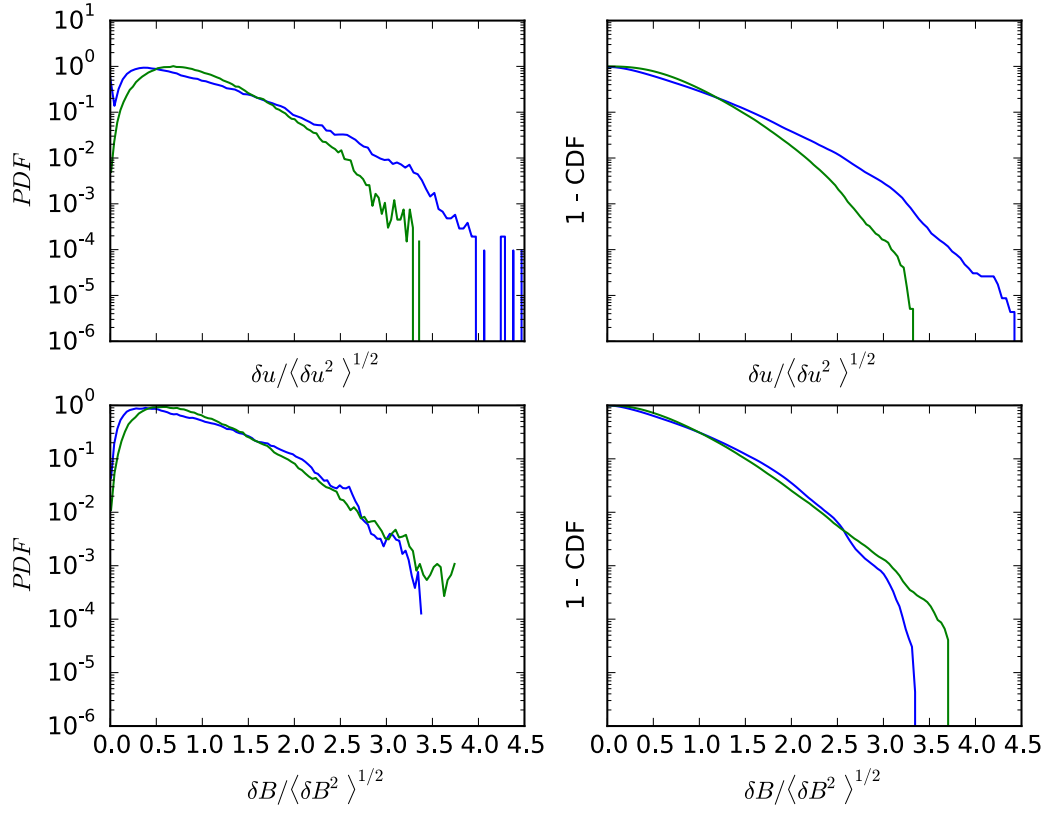

**Figure 7:** Database increments of 57  $dx$  (in green) and WIND increments of 17.1 minutes (in blue).

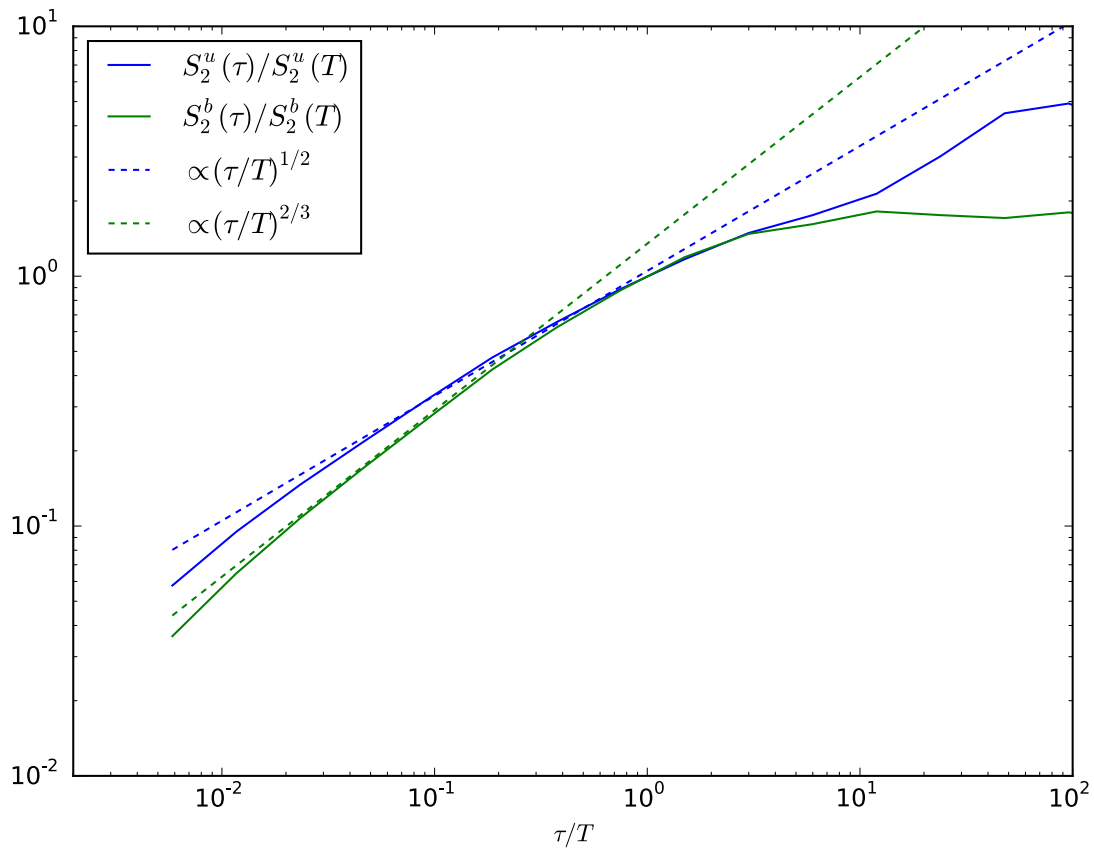

**Figure 8:** Solar Wind Structure Function

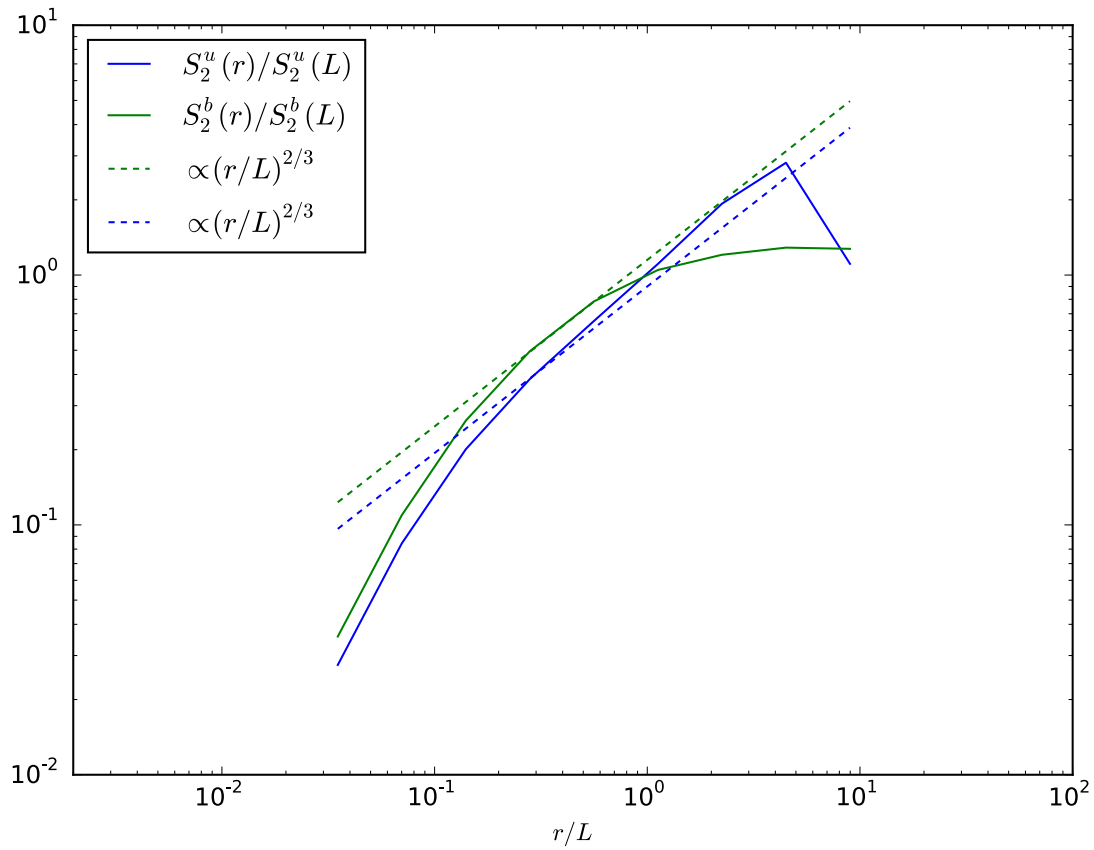

**Figure 9:** JHUTDB Structure Function
